# Supplementary material for: Quantum-Hybrid Stereo Matching With Nonlinear Regularization and Spatial Pyramids
Source: arXiv:2312.16118 source file (2024-12-06)
Supplement: Supplementary file 1 [file X_suppl.tex]

\onecolumn
\setcounter{section}{1}

\clearpage
\makeatletter
\appendix

\addcontentsline{toc}{section}{Supplementary Material}
\part{\Large Supplementary Material} 
This supplement contains material which is relevant to our work, but could not be included in the main body of our paper due to the page limit. In \cref{sec:deriving_rectifiers}, we present the formula and proofs for the function $\Lambda(.,.)$ % promised at the end of
complementing 
\cref{subsec:formulating_mrfs_as_qubos} (main paper). In \cref{sec:binary_encoding_of_mrf_map}, we explain the binary encoding scheme for our MRF as mentioned in \cref{subsec:formulating_mrfs_as_qubos}. In \cref{sec:embedding_problem_graphs}, we also offer an analysis of how our QUBO problems embed onto modern quantum hardware, which was also briefly mentioned in \cref{subsec:formulating_mrfs_as_qubos}. 
In \cref{sec:regularization_hyper_parameters}, we provide the hyperparameters we used in our algorithm as promised in \cref{subsec:stereo_matching_as_an_mrf} (main paper). 
In \cref{sec:coarse_to_fine_ablation}, we ablate our coarse-to-fine method by examining what happens when we remove one intermediate coarse-to-fine step, as we note that each step is necessary in \cref{subsec:stereo_matching_as_an_mrf}. In \cref{sec:rectifier_strength}, we examine what happens to our stereo matching results when we lower the values of the rectifier function $\Lambda(.,.)$, as we mention in \cref{subsec:formulating_mrfs_as_qubos}. Finally, in \cref{sec:sintel_experiments}, we include additional results of running our algorithm on some examples from the Sintel dataset for stereo matching \cite{Butler:ECCV:2012}. 

\section{Deriving Rectifiers For the One-Hot Encoding Scheme}\label{sec:deriving_rectifiers}
\subsection{Deriving Upper Bounds on Non-Granular Rectifiers}
We will now derive the function $\Lambda(\lab{\vv}^r,\lab{\vv}^s)$, which produces sufficiently high rectifier terms in \cref{eq:quadratic_form_equals_markov_energy_with_granular_constraints} such that the QUBO minimizer is the MRF MAP inference. In this section, we define this function such that the constraints are of the form used in QSync \cite{birdal2021quantum}. In \cref{subsec:granular_constraint_implementation}, we derive the more granular function. To define $\Lambda(\lab{\vv}^r,\lab{\vv}^s)$, we require some additional notation. Suppose $(\vp,\vq) \in \mathcal{E}$. Let 
\begin{equation} \label{eq:gamma_def}
    \gamma(\lab{\vp}^r,\vq) :=  \text{max}_{\lab{\vq}^s \in \mathcal{L}_\vq} \{ \varphi_{\vp,\vq}(\lab{\vp}^r,\lab{\vq}^s) \}\,.
\end{equation}
Thus, $\gamma(\lab{\vp}^r,\vq)$ represents the maximum regularization cost present on the edge $(\vp,\vq)$, if $\vp$ has been assigned the label $\lab{\vp}^r$. Next, we define: 
\begin{equation} \label{eq:chi_def}
            \chi(\vp) := \text{max}\{0, \text{min}_{\lab{\vp}^r \in \mathcal{L}_\vp} \{ \varphi_\vp(\lab{\vp}^r) + \sum_{(\vp,\vq) \in \mathcal{E}} \text{max}\{0, \gamma(\lab{\vp}^r,\vq) \} \} + \epsilon \}\,.\\
\end{equation}
$\chi(\vp)$ is an upper bound of the energy increase of flipping a label $\vx_{\lab{\vp}^r}$ of $\vp$ to be $1$. This energy increase is calculated from the data cost of flipping each label, added to the potential highest possible regularization costs of flipping that label. If all labels for $\vp$ are set to $0$, one can always pick a label to flip such that that energy increase is less than or equal to $\chi(\vp)$. 
We now define 
\begin{equation} \label{zeta_def}
    \zeta(\lab{\vp}^r) := \sum_{(\vp,\vq) \in \mathcal{E}} \sum_{\lab{\vq}^s \in \mathcal{L}_\vq} \text{min}\{0,  \varphi_{\vp,\vq}(\lab{\vp}^r, \lab{\vq}^s) \}\}\,.
\end{equation}
This value tracks all negative regularization energy that can be incurred by flipping $\vx_{\lab{\vp}^r}$ of $\vp$ to be $1$. 
Next, define 
\begin{equation}
    \Theta(\lab{\vp}^r,\lab{\vp}^s) := \text{min} \{0, \varphi_\vp(\lab{\vp}^r) + \zeta(\lab{\vp}^r) - \epsilon, \varphi_\vq(\lab{\vq}^s) + \zeta(\lab{\vq}^s) - \epsilon \} \,. 
\end{equation}
This value accounts for the smaller energy decrease of either flipping $\lab{\vp}^r$ or $\lab{\vp}^s$ to $1$.
Now, for any two labels $\lab{\vp}^i, \lab{\vp}^j \in \mathcal{L}_\vp$, we can define our function $\Lambda(\lab{\vp}^i, \lab{\vp}^j)$ as follows: 
\begin{equation}
    \Lambda(\lab{\vp}^i, \lab{\vp}^j) :=  \text{max} \{ \chi(\vp), \text{max}_{\lab{\vp}^r, \lab{\vp}^s \in \mathcal{L}_\vp} \{-\Theta(\lab{\vp}^r, \lab{\vp}^s)\} \}\,.
\end{equation}
We will now show that the lowest energy solution to the QUBO with the matrix presented in \cref{eq:quadratic_form_equals_markov_energy_with_granular_constraints} must satisfy the constraints presented in \cref{eq:onehot_qubo_constraints}.
\subsection{Every Variable Receives at Least One Label} \label{subsubsec:atleast}
This bound ensures that \textit{at least} one binary label $\vx_{\lab{\vp}^r}$ is $1$ for every variable $\vp$. Assume that all other labels $\vx_{\lab{\vp}^s}$ of $\vp$ are set to $0$. We select a label to flip $\lab{\vp}^r$ such that: 
\begin{align}
    \lab{\vp}^r = \text{argmin}_{\lab{\vp}^r \in \mathcal{L}_\vp} \{ \varphi_\vp(\lab{\vp}^r) + \sum_{(\vp,\vq) \in \mathcal{E}} \text{max}\{0, \gamma(\lab{\vp}^r,\vq) \} \} \,. 
\end{align}
Let $c$ be the regularization cost incurred by flipping $\lab{\vp}^r$ to $1$. Then, the total change in energy caused by flipping $\lab{\vp}^r$ is 
\begin{equation} \label{WorstCaseFlipScenario}
% \small
    \begin{split}
        & \varphi_\vp(\lab{\vp}^r) + c - \Lambda(\lab{\vp}^r,\lab{\vp}^r) \leq \\ 
        & \varphi_\vp(\lab{\vp}^r) + c - \chi(\vp) \leq \\
        & \varphi_\vp(\lab{\vp}^r) + c -\text{min}_{\lab{\vp}^r \in \mathcal{L}_\vp} \{ \varphi_\vp(\lab{\vp}^r) + \sum_{(\vp,\vq) \in \mathcal{E}} \text{max}\{0, \gamma(\lab{\vp}^r,\vq) \} \} - \epsilon \,. 
    \end{split}
\end{equation}
By our construction,
\begin{equation}
    c \leq \sum_{(\vp,\vq) \in \mathcal{E}} \text{max}\{0, \gamma(\lab{\vp}^r,\vq) \},
\end{equation}
which means
\begin{equation}
% \small
    \begin{split}
        \varphi_\vp(\lab{\vp}^r) + c \leq \text{min}_{\lab{\vp}^r \in \mathcal{L}_\vp} \{ \varphi_\vp(\lab{\vp}^r) + \sum_{(\vp,\vq) \in \mathcal{E}} \text{max}\{0, \gamma(\lab{\vp}^r,\vq) \} \} \,. \\
    \end{split}
\end{equation}
Therefore, the expression \eqref{WorstCaseFlipScenario} must be less than or equal to $-\epsilon < 0$. Thus, there is still a lower energy to set $\vx_{\lab{\vp}^r} = 1$ rather than $0$.
\subsection{Every Variable Receives at Most One Label} \label{subsubsec:atmost}
Conversely, this bound ensures that \textit{at most} one label $\vx_{\lab{\vp}^r}$ is set to $1$ for a variable $\vp$. Suppose $\vx_{\lab{\vp}^r}$ and $\vx_{\lab{\vp}^s}$ are two binary labels of the same variable. Assume without loss of generality that $\vx_{\lab{\vp}^r}=1$ and $\vx_{\lab{\vp}^s} = 0$. Now, consider the total change in energy that will occur if we flip $\vx_{\lab{\vp}^s}$ to $1$: there will be the cost incurred by the diagonal entry of $Q$ ($ \varphi_\vp(\lab{\vp}^s) - \Lambda(\lab{\vp}^s,\lab{\vp}^s)$), the cost of incurred by setting $\vx_{\lab{\vp}^r}$ and $\vx_{\lab{\vp}^s}$ to $1$  ($2 \Lambda(\lab{\vp}^s,\lab{\vp}^r)$), and some regularization cost from neighbor variables, which we will write as $c$. We sum all of these terms together to consider the total change in energy: 
\begin{align} \label{PrimitiveBoundAtMost}
\begin{split}
    & \varphi_\vp(\lab{\vp}^s) - \Lambda(\lab{\vp}^s,\lab{\vp}^s) + 2 \Lambda(\lab{\vp}^s,\lab{\vp}^r) + c = \\
    & \varphi_\vp(\lab{\vp}^s) + \Lambda(\lab{\vp}^s,\lab{\vp}^s) + c  \geq \\
    & \varphi_\vp(\lab{\vp}^s) + \text{max}_{\lab{\vp}^r, \lab{\vp}^s \in \mathcal{L}_\vp} \{-\Theta(\lab{\vp}^r, \lab{\vp}^s)\} + c \geq \\
    & \varphi_\vp(\lab{\vp}^s)  -\Theta(\lab{\vp}^r, \lab{\vp}^s) + c = \\
    & \varphi_\vp(\lab{\vp}^s)  -\text{min} \{0, \varphi_\vp(\lab{\vp}^r) + \zeta(\lab{\vp}^r) - \epsilon, \varphi_\vp(\lab{\vp}^s) + \zeta(\lab{\vp}^s) - \epsilon \} + c = \\
    & \varphi_\vp(\lab{\vp}^s) +  \text{max} \{0, -\varphi_\vp(\lab{\vp}^r) - \zeta(\lab{\vp}^r) + \epsilon, -\varphi_\vp(\lab{\vp}^s) -\zeta(\lab{\vp}^s) + \epsilon \} + c \geq \\
    & \varphi_\vp(\lab{\vp}^s) -\varphi_\vp(\lab{\vp}^s) -\zeta(\lab{\vp}^s) + \epsilon + c = \\
    & -\zeta(\lab{\vp}^s) + \epsilon + c \,.
\end{split}
\end{align}
By the construction of $\zeta(\lab{\vp}^s)$ in \cref{zeta_def}, $\zeta(\lab{\vp}^s)$ must be less than or equal to $c$. Thus, our expression above is greater than or equal to $\epsilon > 0$. Thus, there is a net increase in energy when we set both labels to $1$.  

\subsection{Proof of Correct QUBO Behaviour} \label{subsubsec:CorrectBehaviour}
We can guarantee that the lowest energy state satisfies our constraints. To understand this, consider a QUBO solution $\vx$ where, for some Markov variable $\vp$, all binary variables $\vx_{\lab{\vp}^i}$ are $0$. Then \cref{subsubsec:atleast} proves that there is a label that can be flipped to $1$ to lower the energy. Therefore, $\vx$ must not be the optimal solution. Now, consider a solution $\vx$ where $2$ or more binary variables that act as labels for Markov variable $\vp$ are set to $1$. \ref{subsubsec:atmost} shows that there will be a net energy decrease if one of those variables is flipped to $0$. Therefore, $\vx$ cannot be the optimal solution. Therefore, the optimal QUBO solution must obey the constraints in \cref{eq:onehot_qubo_constraints}. 

Let $\vx$ be a QUBO solution which obeys all constraints, and corresponds to a labelling $\ell$. The total energy of the QUBO is: 
\begin{equation} 
    \vx^TQ\vx = E(\ell) - \sum_{\vp \in \mathcal{V}} \Lambda(\lab{\vp}^i,\lab{\vp}^i) \,,
    \label{EnergyOfConstrainedSolution}
\end{equation}
with $E(\ell)$ as defined in \cref{eq:markov_cost_quadratic_form}. Because $\sum_{\vp \in \mathcal{V}} \Lambda(\lab{\vp}^i,\lab{\vp}^i)$ is a constant, it is clear that any solution $\vx^*$ which minimizes $\vx^TQ\vx$ must therefore minimize $E(\ell_{(.)})$. 
\subsection{A More Granular Implementation of Constraints}\label{subsec:granular_constraint_implementation}
We can treat $\Lambda$ is a function of individual labels:
\begin{equation}
    \Lambda(\lab{\vp}^r,\lab{\vp}^s) = 
    \begin{cases}
        \chi(\vp) & \text{ if } r = s \\
        \frac{\chi(\vp) -\Theta(\lab{\vp}^r, \lab{\vp}^s)}{2} & \text{ else } \,.\\
    \end{cases}  \\
\end{equation}
We prove that the resulting QUBO obeys our constraints at its optimum, and then the rest of the proof follows exactly the derivations in \cref{subsubsec:CorrectBehaviour}.

To prove that every variable receives at least one label, the same argument given in \cref{subsubsec:atleast} holds in this case as well. We can show that for every $\vp$, there exists a label $\lab{\vp}^r$ such that flipping it to $1$ will cause an energy change of $\varphi_\vp(\lab{\vp}^r) + c - \chi(\vp) < 0$ if no other label has been flipped yet.

To prove that every variable receives at most one label, the argument given in \cref{subsubsec:atmost} needs to be modified slightly. In this case, the net change in energy from flipping $\vx_{\lab{\vp}^2}$ to $1$ is:
\begin{align}
    \begin{split}
        &\varphi_\vp(\lab{\vp}^s) - \chi(\vp) + 2 \frac{\chi(\vp) -\Theta(\lab{\vp}^r,\lab{\vp}^s)}{2} + c = \\
        &\varphi_\vp(\lab{\vp}^s) - \Theta(\lab{\vp}^r,\lab{\vp}^s) + c \,.\\
    \end{split}
\end{align}
From here, the proof follows the same logic as in \cref{PrimitiveBoundAtMost}. 

\subsection{Analysis of Improvement}
The decrease in $\Lambda(\lab{\vp}^r, \lab{\vp}^s)$ for  $r=s$ is: 
\begin{equation}
    \text{max} \{0 , \text{max}_{\lab{\vp}^r, \lab{\vp}^s \in \mathcal{L}_\vp} \{-\Theta(\lab{\vp}^r, \lab{\vp}^s)\} - \chi(\vp) \} \,.
\end{equation}
The decrease in $\Lambda(\lab{\vp}^r, \lab{\vp}^s)$ for  $r \neq s$ is:
\begin{equation}
        \text{max} \bigg\{ \frac{\chi(\vp) + \Theta(\lab{\vp}^r, \lab{\vp}^s)}{2} ,  \text{max}_{\lab{\vp}^r, \lab{\vp}^s \in \mathcal{L}_\vp} \{-\Theta(\lab{\vp}^r, \lab{\vp}^s)\} - \frac{\chi(\vp) -\Theta(\lab{\vp}^r, \lab{\vp}^s)}{2} \bigg\} \,.
\end{equation}
By implementing more granular constraints, we can be less disruptive to the energy landscape with the same constraint guarantees. Thus, this formulation is an improvement upon the less granular formulation presented in \cite{birdal2021quantum}
\section{The Binary Encoding of MRF MAP Inference}\label{sec:binary_encoding_of_mrf_map}
\subsection{Encoding the MRF Energy as a High-Order Binary Polynomial}

Let $\operatorname{deg}(\vp)$ represent the degree of variable $\vp$, that is, how many variables are neighbors of $\vp$, and define:
\begin{equation} \label{f_def}
    f_{\vp,\vq}(\lab{\vp},\lab{\vq}) = \frac{\varphi_\vp(\ell_\vp)}{\operatorname{deg}(\vp)} + \varphi_{\vp,\vq}(\ell_\vp,\ell_\vq) + \frac{\varphi_\vq(\ell_\vq)}{\operatorname{deg}(\vq)} \,. 
\end{equation}
We can view the Markov cost function \cref{eq:MRF_energy} from a different perspective: 
\begin{equation} \label{eq:label_energy_full_sum}
    E(\ell_{(\cdot)}) = \sum_{(\vp,\vq) \in \mathcal{E}} f_{\vp,\vq}(\lab{\vp},\lab{\vq}) \,. 
\end{equation}

For every Markov variable $\vp$, we define our label space to be $\mathcal{L}_\vp = \{0, 1\}^n$, and we define binary variables $\{\vx_{\vp,0},...,\vx_{\vp,n}\}$. Each $\vx_{\vp,i}$ is flipped to $0$ or $1$, and the sequence $\vx_{\vp,0},...,x_{\vp,n}$ is a binary encoding of a label in $\mathcal{L}_\vp$. For label spaces whose size is not a power of $2$, we include extra labels to round the size up to the nearest power of $2$. The extra labels can be duplicates of the original labels. 

We will now represent $f_{\vp,\vq}$ as a polynomial of the binary variables $\{\vx_{\vp,0},...,\vx_{\vp,n}\}$, and $\{\vx_{\vq,0},...,\vx_{\vq,m}\}$. To construct this polynomial, we require the following notation: Let $(\sigma_\vp)_i$ be the $i^\text{th}$ entry of the binary string $\sigma_\vp \in \mathcal{\vp}$. Define:
\begin{align}
    \begin{split}
    \delta(\sigma_\vp, \vx_{\vp,i}) =
        \begin{cases}
            \vx_{\vp,i} & \text{if } (\sigma_\vp)_i = 1\\
            1, & \text{if } (\sigma_\vp)_i = 0 \,. 
        \end{cases}
    \end{split}
\end{align}
Then, $f_{\vp,\vq}$ is a polynomial of the following form: 
\begin{align} \label{eq:higher_order_binary_polynomial}
    f_{\vp,\vq}(\vx_{\vp,0},...,\vx_{\vp,n},\vx_{\vq,0},...,\vx_{\vp,m}) = \sum_{(\sigma_\vp,\sigma_\vq) \in \mathcal{L}_\vp \times \mathcal{L}_\vq} a_{\sigma_\vp,\sigma_\vq} (\Pi_{i \in 
 [1, ... , n]} \delta (\sigma_\vp,\vx_{\vp,i})) \cdot (\Pi_{j \in [1, ... , m]}\delta (\sigma_\vq,\vx_{\vq,j}))\,.
\end{align}
where the formula for $a_{\sigma_\vp,\sigma_\vq}$ is defined as follows: We order $\sigma'_\vp \leq \sigma_\vp$, if for every index $i$, $(\sigma'_\vp)_i \leq (\sigma_\vp)_i$. Additionally, we define $\kappa (\sigma_\vp)$ to be equal to the number of $1$'s present in $\kappa (\sigma_\vp)$. We can write $a_{\sigma_\vp,\sigma_\vq}$ as:
\begin{align} \label{eq:binary_encoding_coefficient_formula}
    a_{\sigma_\vp,\sigma_\vq} := \sum_{\sigma'_\vp \leq \sigma_\vp , \sigma'_\vq \leq \sigma_\vq}  (-1)^{\kappa(\sigma_\vp) + \kappa(\sigma_\vq)  - \kappa(\sigma'_\vp)  - \kappa(\sigma'_\vq)} f_{\vp,\vq}(\sigma'_\vp,\sigma'_\vq) \,. 
\end{align}
We now prove that this formula provides the correct coefficients for our polynomial.
\subsection{Proof of Coefficient Formula Correctness}
If we plug in the binary strings  $\vx_\vp \equiv \vx_{\vp,0},...,\vx_{\vp,n}$ and $\vx_\vq \equiv \vx_{\vq,0},...,\vx_{\vp,m}$ into \cref{eq:higher_order_binary_polynomial}, we obtain:
\begin{align}
    \begin{split}
        f_{\vp,\vq}(x_\vp,x_\vq)  & = \sum_{\sigma_\vp \leq x_\vp,\sigma_\vq \leq x_\vq} a_{\sigma_\vp,\sigma_\vq} \\
        & = \sum_{\sigma_\vp \leq x_\vp,\sigma_\vq \leq x_\vq} \sum_{\sigma'_\vp \leq \sigma_\vp , \sigma'_\vq \leq \sigma_\vq}  (-1)^{\kappa(\sigma_\vp) + \kappa(\sigma_\vq)  - \kappa(\sigma'_\vp)  - \kappa(\sigma'_\vq)} f_{\vp,\vq}(\sigma'_\vp,\sigma'_\vq) \\
        & = \sum_{\sigma'_\vp \leq x_\vp,\sigma'_\vq \leq x_\vq} f_{\vp,\vq}(\sigma'_\vp,\sigma'_\vq) \sum_{\sigma'_\vp \leq \sigma_\vp \leq x_\vp , \sigma'_\vq \leq \sigma_\vq \leq x_\vq}  (-1)^{\kappa(\sigma_\vp) + \kappa(\sigma_\vq)  - \kappa(\sigma'_\vp)  - \kappa(\sigma'_\vq)} \,.
    \end{split}
\end{align}
We now focus on simplifying the inner term: 
\begin{align}
    \begin{split} \label{eq:combinatorial_sum_term}
    \sum_{\sigma'_\vp \leq \sigma_\vp \leq x_\vp , \sigma'_\vq \leq \sigma_\vq \leq x_\vq}  (-1)^{\kappa(\sigma_\vp) + \kappa(\sigma_\vq)  - \kappa(\sigma'_\vp)  - \kappa(\sigma'_\vq)} \,. 
    \end{split}
\end{align}
We can regroup this sum into terms with different values of $\kappa(\sigma'_\vp) + \kappa(\sigma'_\vq)$. From combinatorics, we know that there are exactly $\binom{ \kappa(x_\vp) + \kappa(x_\vq) - \kappa(\sigma'_\vp) - \kappa(\sigma'_\vq) }{k - \kappa(\sigma'_\vp) - \kappa(\sigma'_\vq) }$ pairs of binary strings $\sigma_\vp$, $\sigma_\vq$ such that $\kappa(\sigma_\vp) + \kappa(\sigma_\vq) = k$. Therefore, we can express \cref{eq:combinatorial_sum_term} as: 
\begin{align}
    \sum_{\kappa(\sigma'_\vp) + \kappa(\sigma'_\vq) \leq k \leq \kappa(x_\vp) + \kappa(x_\vq) } \binom{ \kappa(x_\vp) + \kappa(x_\vq) - \kappa(\sigma'_\vp) - \kappa(\sigma'_\vq)   }{ k - \kappa(\sigma'_\vp) - \kappa(\sigma'_\vq) } (-1)^{ k - \kappa(\sigma'_\vp) - \kappa(\sigma'_\vq) } \,. 
\end{align}
We can shift the indices of this sum by $\kappa(\sigma'_\vp) + \kappa(\sigma'_\vq)$:
\begin{align}
    \sum_{ 0 \leq k \leq \kappa(x_\vp) + \kappa(x_\vq) - \kappa(\sigma'_\vp) - \kappa(\sigma'_\vq) } \binom{ \kappa(x_\vp) + \kappa(x_\vq) - \kappa(\sigma'_\vp) - \kappa(\sigma'_\vq)  }{k } (-1)^{ k } \,.
\end{align}
Next, we multiply this term by $1^{\kappa(x_\vp) + \kappa(x_\vq) - \kappa(\sigma'_\vp) - \kappa(\sigma'_\vq) - k } \equiv 1$ and obtain: 
\begin{align}
    \sum_{ 0 \leq k \leq \kappa(x_\vp) + \kappa(x_\vq) - \kappa(\sigma'_\vp) - \kappa(\sigma'_\vq) } \binom{ \kappa(x_\vp) + \kappa(x_\vq) - \kappa(\sigma'_\vp) - \kappa(\sigma'_\vq) }{ k } (-1)^{ k } 1^{ \kappa(x_\vp) + \kappa(x_\vq) - \kappa(\sigma'_\vp) - \kappa(\sigma'_\vq) - k } \,.
\end{align}
By the binomial theorem, this is equivalent to: 
\begin{align}
    (-1 + 1)^{\kappa(x_\vp) + \kappa(x_\vq) - \kappa(\sigma'_\vp) - \kappa(\sigma'_\vq)} \,.
\end{align}
If $\sigma'_\vp = x_\vp$ and $\sigma'_\vq = x_\vq$, this expression is $1$, and $0$ otherwise. Therefore, we can evaluate the last expression in \cref{eq:higher_order_binary_polynomial} to be equal to $f_{\vp,\vq}(x_\vp,x_\vq)$, as needed. This completes the proof. 
Therefore, if we could somehow transform the minimization of 
\begin{align}
    E(\ell_{(\cdot)}) = \sum_{(\vp,\vq) \in \mathcal{E}}
    \sum_{(\sigma_\vp,\sigma_\vq) \in \mathcal{L}_\vp \times \mathcal{L}_\vq} a_{\sigma_\vp,\sigma_\vq} (\Pi_{i \in [1, ... , n]} \delta (\sigma_\vp,x_{\vp,i})) \cdot (\Pi_{j \in [1, ... , m]}\delta (\sigma_\vq,x_{\vq,j})), 
\end{align}
into the minimization of a quadratic polynomial, we will have formed a QUBO problem. 

\subsection{Transforming Higher-Order Binary Vector Polynomial Minimization into a QUBO}
A technique to transform higher-order polynomial minimization over a binary vector into a QUBO 
exists and is well explained in Ishikawa \cite{5444874}: In Sec.~4.2, it is shown that, in a polynomial minimization problem in which all variables are binary, a polynomial term 
\begin{equation}
    a\vx_0...\vx_k
\end{equation}
can be transformed into 
\begin{equation}
    \text{min}_{w \in \{0,1\}} a w \{ S_1 - (k-1) \}, 
\end{equation} 
when $a < 0$ and 
\begin{equation}
    \text{min}_{w_0,...w_{\lfloor \frac{k-1}{2}\rfloor} \in \{0,1\}} a \{ \sum_{i=1}^k w_i(c_{i,k} (-S_1 + 2i)-1) + a S_2 \},
\end{equation}
when $a > 0$, and the minimal argument of the polynomial remains the same. Here, $c_{i,k} = 1$ if $k$ is odd and $i=k$, and $c_{i,k} = 2$ otherwise. $S_1$ and $S_2$ are defined as:
\begin{equation}
    S_1 = \sum_{i=1}^k \vx_i \,\,\mathrm{and}
\end{equation}
\begin{equation}
    S_2 = \frac{S_1(S_1-1)}{2} \,.
\end{equation}
This construction introduces auxiliary binary variables ($w$ if $a < 0$ or $w_1,...,w_k$ if $a > 0$) to handle the complexity of higher-order terms. These auxiliary binary variables are added into our QUBO problem, and must be optimized alongside our original binary variables. However, once the optimization is complete, we can read off our solution from the original variables and discard the response of the auxiliary variables. 

With these techniques, minimization of a polynomial of binary variables of any order can be reduced to a minimization of a quadratic polynomial of binary variables by iteratively applying the transformations explained above to any terms of order greater than $2$. A full proof of why these transformations preserve the minimal argument of the polynomial is too long to explain here, but is elaborated on at length in Ishikawa \cite{5444874}. 

We have shown how to express the minimization of $E(\ell_{(\cdot)})$ as a minimization over binary variables. A sketch of the full encoding algorithm goes as follows: 1) For each edge $(\vp,\vq)$, calculate all $a_{\vp,\vq}$ from \cref{eq:binary_encoding_coefficient_formula}; 2) sum all $f_{\vp, \vq}$ into one large polynomial $E(\ell_{(\cdot)})$ (See \cref{eq:label_energy_full_sum}), and reduce all higher-order terms to quadratic or lower using the techniques in Ishikawa \cite{5444874}; 3) build $Q$ from the resulting coefficients. 
\section{Embedding QUBO Problem Graphs onto D-Wave}\label{sec:embedding_problem_graphs}
One key bottleneck for modern quantum computing is minor embedding: once a QUBO is defined, all the binary variables of $\vx$ must be mapped to physical qubits present on the QPU, and all non-zero entries of the off-diagonals of $Q$ must be mapped to the appropriate physical couplers connecting physical qubits. To make this embedding process more flexible, it is possible to chain qubits together: any two physical qubits which share a coupler can be treated as a single physical qubit during the embedding. However, during annealing, qubit chains are at risk of breaking (\textit{i.e.,} not behaving like a single physical qubit), making it ill-defined to measure the QUBO solution from the annealer. The longer the qubit chain, the higher the risk of the chain breaking. Therefore, we aim to keep chains as small as possible.  

We first examine the embedding properties of our one-hot encoding scheme, and then turn our attention to the binary encoding scheme proposed in \cref{sec:binary_encoding_of_mrf_map}, and see why it is more challenging to embed.

\subsection{Embedding of the One-Hot Encoding Scheme}
A QUBO's \textit{problem graph} is a useful concept for discussing minor embedding. For a QUBO problem represented by the matrix $Q$, the corresponding problem graph has vertices corresponding to each binary variable of the QUBO, and edges connecting any two vertices whose corresponding binary variables interact in the QUBO problem. We visualize the QUBO problem graphs for the first epipolar line of the Venus image pair at all three coarse-to-fine steps in \cref{fig:qubo_problem_graphs}. We visualize those same problem graphs when they are embedded onto the D-Wave Pegasus hardware in \cref{fig:qubo_problem_embeddings}. The numerics for these problem graphs and embeddings are given in \cref{tab:dwave_embeddings_one_hot}.

For all steps, an embedding is possible, meaning our algorithm can be run on modern hardware. Additionally, the number of vertices of our QUBO problem graph grows linearly as the number of disparities considered by the algorithm increases, or when the length of the epipolar line increases. This means that the one-hot encoding scales well as our problem size increases.
\begin{figure}
    \centering
    \setlength\tabcolsep{1.5pt}
    \begin{tabular}{c c c}
                   \textbf{Step 1} & \textbf{Step 2} & \textbf{Step 3} \\
       \includegraphics[width=\embeddingtableimagewidth, height=\embeddingtableimageheight]{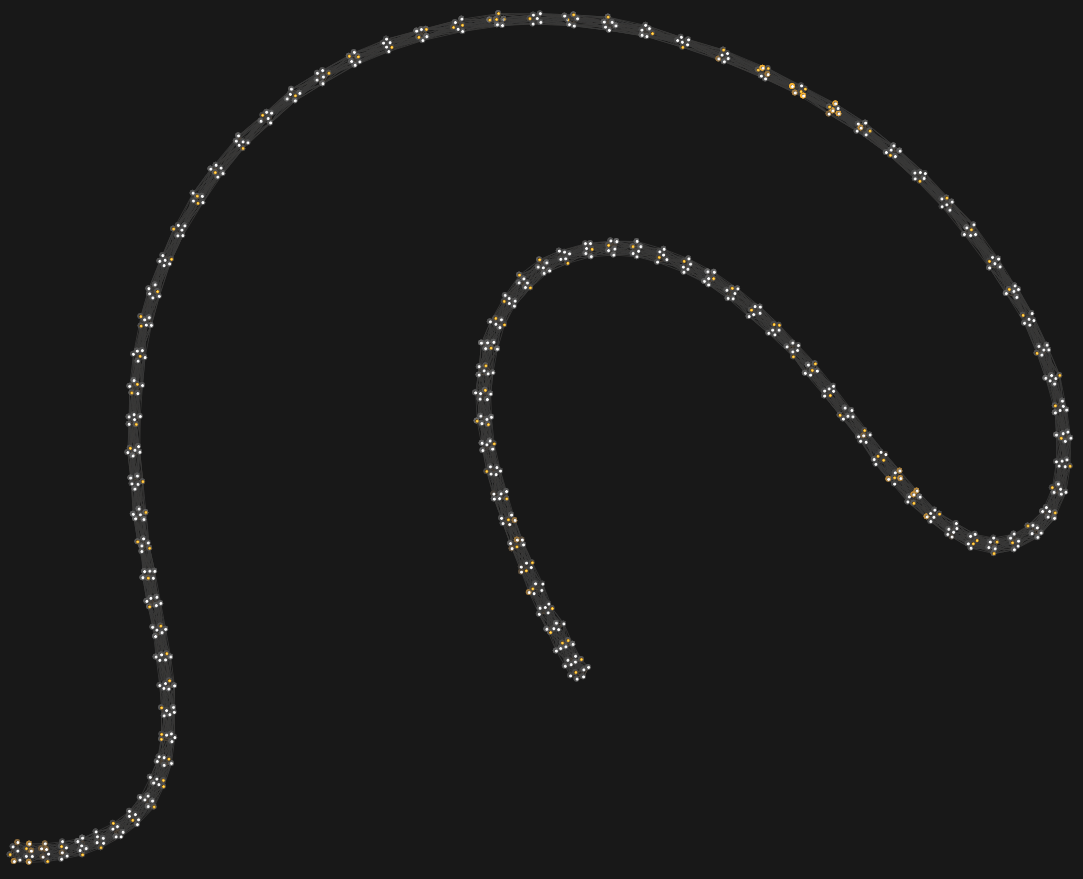} & \includegraphics[width=\embeddingtableimagewidth, height=\embeddingtableimageheight]{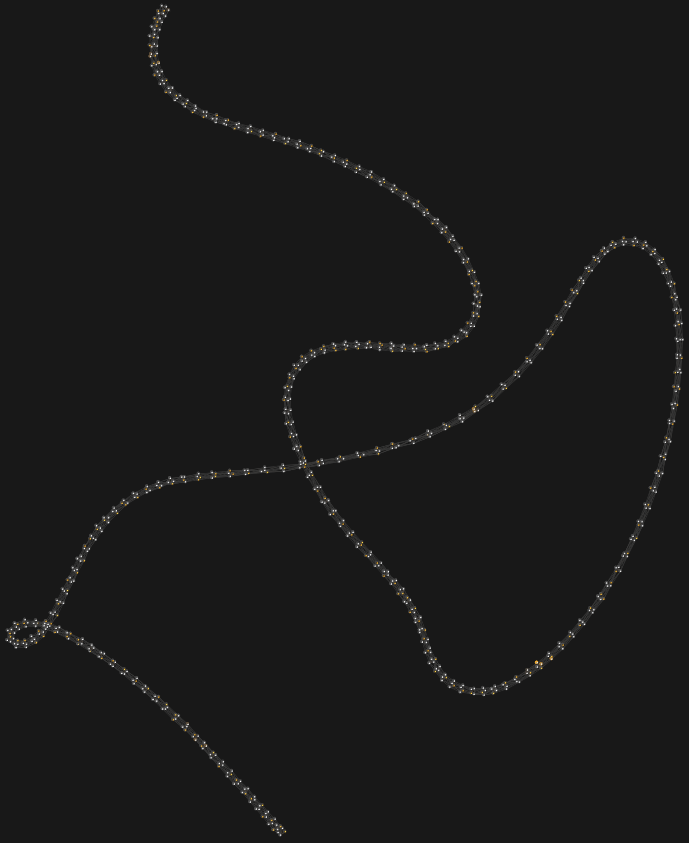}  & \includegraphics[width=\embeddingtableimagewidth, height=\embeddingtableimageheight]{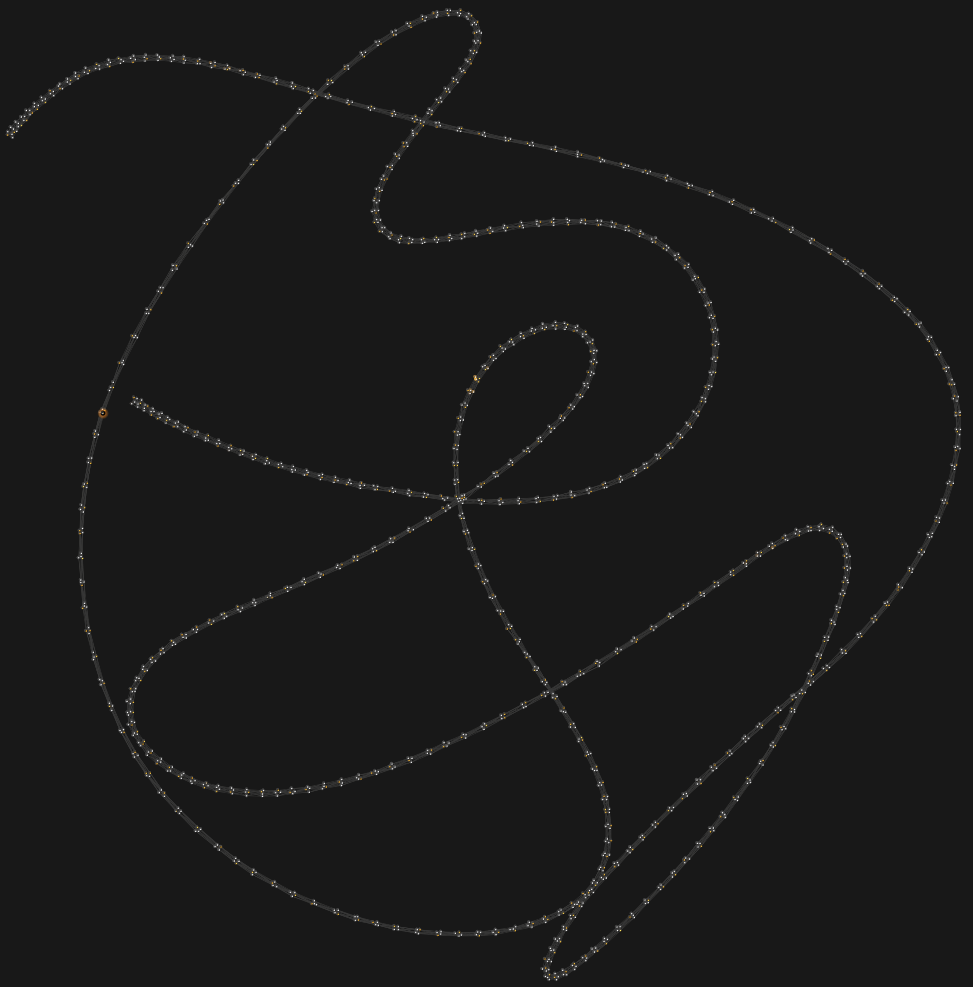} \\
    \end{tabular}
    \caption{The QUBO problem graphs for the first epipolar line of Venus image pair visualized using D-Wave's Problem Inspector. The single curve structure of these graphs arises because regularization costs only occur between the immediate neighbors on the epipolar line.} 
    \label{fig:qubo_problem_graphs}
\end{figure}
\begin{figure}
    \centering
    \setlength\tabcolsep{1.5pt}
    \begin{tabular}{c c c}
                   \textbf{Step 1} & \textbf{Step 2} & \textbf{Step 3} \\
       \includegraphics[width=\embeddingtableimagewidth, height=\embeddingtableimageheight]{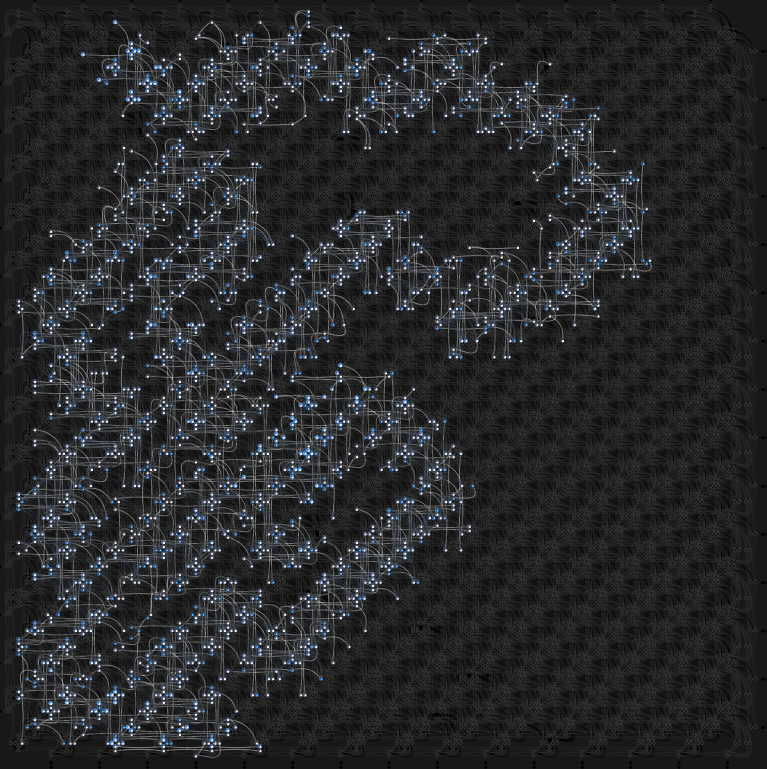} & \includegraphics[width=\embeddingtableimagewidth, height=\embeddingtableimageheight]{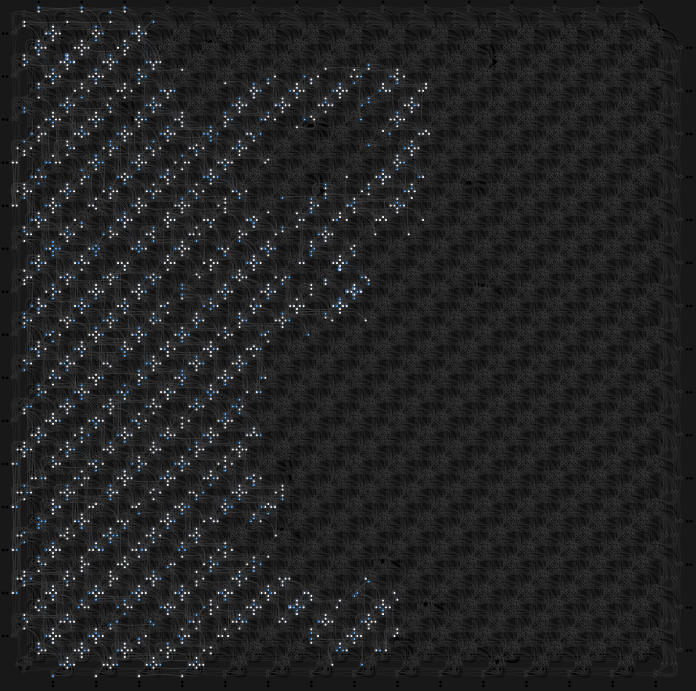}  & \includegraphics[width=\embeddingtableimagewidth, height=\embeddingtableimageheight]{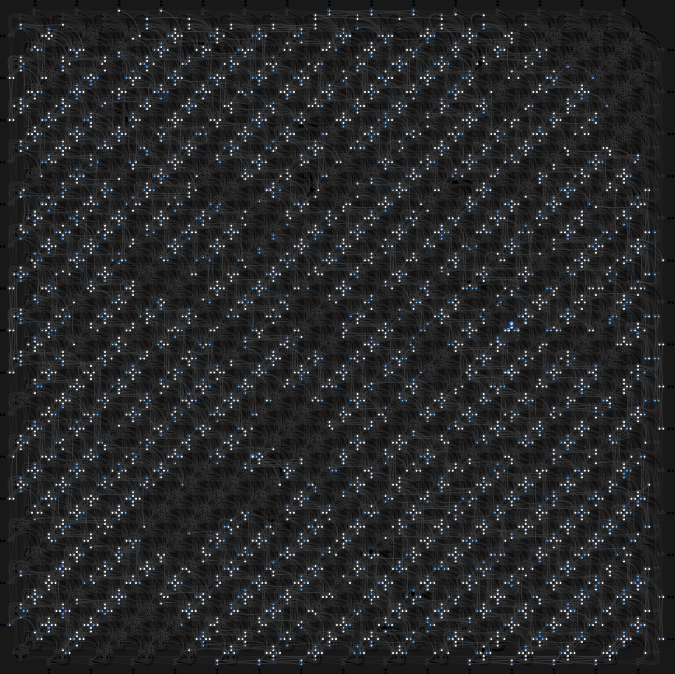} \\
    \end{tabular} 
    \caption{The QUBO problem embeddings onto D-Wave's Pegasus QPU for the first epipolar line of Venus image pair visualized using D-Wave's Problem Inspector. The Pegasus QPU has $5,640$ qubits with $40,484$ couplers \cite{2020arXiv200300133B}. Although the QUBO problem graphs have much fewer vertices and edges than the Pegasus QPU's qubits and couplers, one can see that a large portion of these resources are needed in order to embed properly. This is because many qubit chains are used for the embedding.} 
    \label{fig:qubo_problem_embeddings} 
\end{figure}

\begin{table}
    \centering
    \begin{tabular}{|c|c|c|c|}
        \hline
        \textbf{Step} & \textbf{1} & \textbf{2} & \textbf{3}  \\
        \hline
        \textbf{Epipolar Line Length} & 108 & 217 & 434 \\
        \hline
        \textbf{Disparity Levels} & 6 & 4 & 4 \\
        \hline
        \textbf{QUBO Graph Nodes} & 648 & 868 & 1,736 \\
        \hline
        \textbf{QUBO Graph Edges} & 5,472 & 4,758 & 9,532\\
        \hline
        \textbf{Physical Qubits} & 2,254 & 1,937 & 3,795\\
        \hline
        \textbf{Physical Couplers} & 6,541 & 5,827 & 11,591\\
        \hline
        \textbf{Physical Max Chain Length} & 10 & 5 & 5\\
        \hline
    \end{tabular}
  \caption{QUBO Problem graph statistics for our method with a one-hot encoding scheme for a single epipolar line, and statistics on the computed embeddings of the QUBO problem graphs onto the D-Wave Pegasus QPU. The epipolar line length is from the widest of the Middlebury images, Venus and Sawtooth. Thus, our stereo matching QUBO problems are embeddable on modern quantum hardware.}
  \label{tab:dwave_embeddings_one_hot}
\end{table}
\subsection{Embedding of the Binary Encoding Scheme}
We report the number of QUBO problem graph edges and vertices required for stereo matching the Venus image pair (across all steps) in \cref{tab:dwave_embeddings_binary_encoding}. For Step 1, the number of edges is greater than the number of couplers, meaning it is impossible to find an embedding.
As the number of disparities grows, the number of auxiliary binary variables needed grows exponentially (see Section 5.4 of Ishikawa \cite{5444874}). This explains why the problem graph for the initial step is so large. Note that the number of binary variables needed still grows linearly with respect to epipolar line length. 

D-Wave's upcoming QPU with the Zephyr topology (expected in 2024) should contain $7.4 \cdot 10^4$ qubits \cite{Zephyr2021}. However, we were still unable to find an embedding for Step 1 in this topology. Because we cannot embed this binary encoding approach into modern or next-generation QPU's, we decided to focus our attention on using the one-hot encoding scheme.
\begin{table}
    \centering
    \begin{tabular}{|c|c|c|c|}
        \hline
        \textbf{Step} & \textbf{1} & \textbf{2} & \textbf{3}  \\
        \hline
        \textbf{QUBO Graph Nodes} & 5,461 & 1,514 & 3,033 \\
        \hline
        \textbf{QUBO Graph Edges} & 147,452 & 7,561 & 15,156 \\
        \hline
    \end{tabular}
  \caption{Computed embeddings for the D-Wave Pegasus, binary encoding. Given the increased complexity of the graph topology, we were unable to calculate embeddings for all $3$ resolution levels. 
  } 
  \label{tab:dwave_embeddings_binary_encoding}
\end{table} 
\section{Model Hyperparameters} \label{sec:regularization_hyper_parameters}
We summarize our model parameters used across all three coarse-to-fine levels of our algorithm in \cref{tab:model_hyperparamters}. These parameters were found to optimize RMSE while keeping an acceptable BPP. The median filter is across an entire window -- and not a vertical median filter as in \cite{9653310} -- as we found this improved the estimation. We found that at the full resolution, a non-truncated regularizer worked best in general. Nevertheless, we still leverage the truncation at lower levels, so it is still present in our approach. Also, note that the range of $I^L, I^R$ is on the interval $[0,1]$. 
\begin{table}[]
    \centering
    \begin{tabular}{|c| c | c | c | }
        \hline
        \textbf{Step} & \textbf{1} & \textbf{2}  & \textbf{3}  \\ \hline
        Downsample Factor (\cref{alg:full_quantum_algorithm}) & 4 & 2 & 1  \\ \hline
        Displacements Considered (\cref{alg:full_quantum_algorithm})  & 6 & 4 & 4 \\ \hline
        $\tau$ (\cref{eq:edge_aware_potts_model}) & 0.15 & 0.15 & 0.3  \\ \hline
        q (\cref{eq:edge_aware_potts_model})  & 10 & 10 & 10 \\ \hline
        m (\cref{eq:truncated_linear_regularizer}) &  0.0015 & 0.0015 & $\infty$ \\ \hline
        s (\cref{eq:truncated_linear_regularizer}) & 0.0005 & 0.0003 & 0.0005\\ \hline
        Median Filter Window (\cref{alg:full_quantum_algorithm}) & 7$\times$7 & 7$\times$7& 7$\times$7 \\ \hline
        Bilateral Filter Diameter (\cref{alg:full_quantum_algorithm}) & \textbf{n/a} & \textbf{n/a} & 12 \\ \hline
        Bilateral Filter Sigma Color (\cref{alg:full_quantum_algorithm}) & \textbf{n/a} & \textbf{n/a} & 75 \\ \hline 
        Bilateral Filter Sigma Space (\cref{alg:full_quantum_algorithm}) & \textbf{n/a} & \textbf{n/a} & 75 \\ \hline 
        \end{tabular}   
    \caption{Hyperparameters for our stereo matching algorithm described in \cref{subsec:our_algorithm} of the main paper.} 
    \label{tab:model_hyperparamters}
\end{table}
\section{Ablation Study on the Coarse-to-Fine Levels}\label{sec:coarse_to_fine_ablation}
We investigated how well our method works if we have fewer coarse-to-fine levels. In the following experiment, we removed the iteration which considers stereo matching at a downsampling factor of $2$ (step $2$). The modified algorithm can still estimate all disparities (rounded to the nearest integer) present in the ground truth, provided that it makes the correct estimation at each step.  The visual results as shown in \cref{fig:ablation_ctof} and numerical results are shown in \cref{tab:ctof_ablation}. 
Other than the Sawtooth image pair, we see a decline visually and numerically in our estimates. We conclude that having intermediate resolution steps is useful to our method. They give the algorithm more opportunities to adjust as higher resolution details are shown, correcting previous inaccuracies. We also suspect that the inaccurate estimates for Sawtooth begin in the second iteration because its omission leads to better numerical results, and the improvement is particularly noticeable in the troublesome lower left area. 
\begin{table}[]
    \centering
    \begin{tabular}{|c| c | c || c | c |}
        \hline
        \multirow{2}{*}{\textbf{Image Pair}} &  \multicolumn{2}{ c ||}{\textbf{AS}} & \multicolumn{2}{ c |}{\textbf{NS2}}  \\ \cline{2-5} 
            & RMSE & BPP & RMSE & BPP  \\
            \hline
        \textbf{Tsukuba} & 1.53 & 12.93 & 1.60 & 13.97 \\ \hline
        \textbf{Bull}    & 0.58 & 3.46 & 0.82 & 10.15    \\ \hline
        \textbf{Sawtooth} & 1.89 & 24.51 & 1.71 & 18.06  \\ \hline
        \textbf{Venus}   & 0.96 & 8.16 & 1.15 & 13.62  \\ \hline
        \textbf{Average} & \textbf{1.24} & \textbf{12.27} & 1.32 & 13.95  \\ \hline
        \end{tabular}
    \caption{The Root Mean Squared Error (RMSE) and Bad Pixel Percentage (BPP) of our full method with \textbf{A}ll \textbf{S}teps, and  our method when the iteration step at the intermediate resolution is removed (\textbf{N}o \textbf{S}tep \textbf{2}). The Gurobi optimizer is used in both cases. The full algorithm has lower RMSE an BPP. }
    \label{tab:ctof_ablation}
\end{table}

\begin{figure}
    \centering
    \setlength\tabcolsep{1.5pt}
    \begin{tabular}{c c c c c}
                   & Tsukuba & Bull & Sawtooth & Venus \\
       \rotatebox{90}{\textcolor{white}{------------}\textbf{GT}} & \includegraphics[width=\tableimagewidth, height=\tableimageheight]{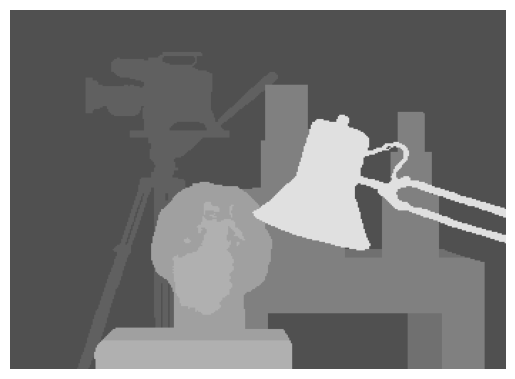} & \includegraphics[width=\tableimagewidth, height=\tableimageheight]{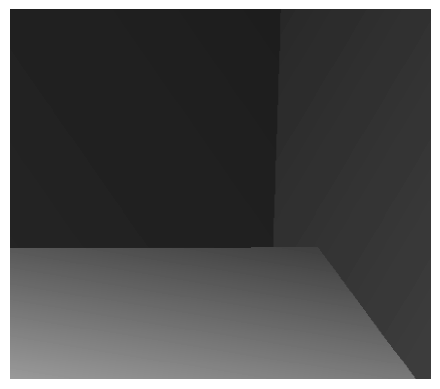}  & \includegraphics[width=\tableimagewidth, height=\tableimageheight]{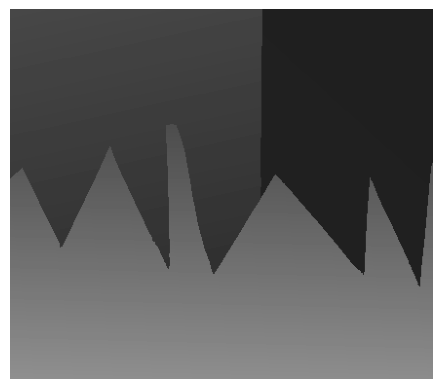} & \includegraphics[width=\tableimagewidth, height=\tableimageheight]{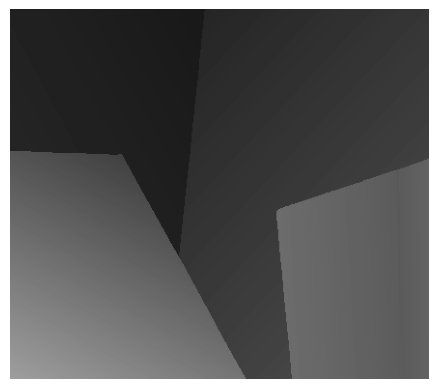}\\
       \rotatebox{90}{\textcolor{white}{-----------}\textbf{AS}} & \includegraphics[width=\tableimagewidth, height=\tableimageheight]{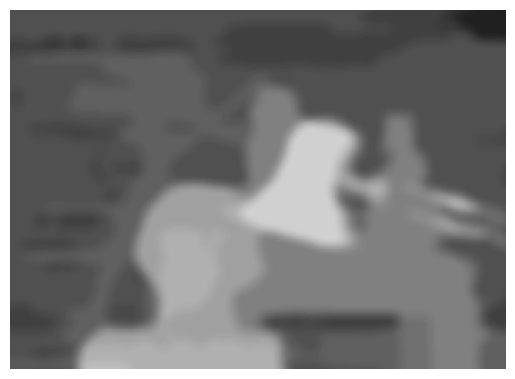} & \includegraphics[width=\tableimagewidth, height=\tableimageheight]{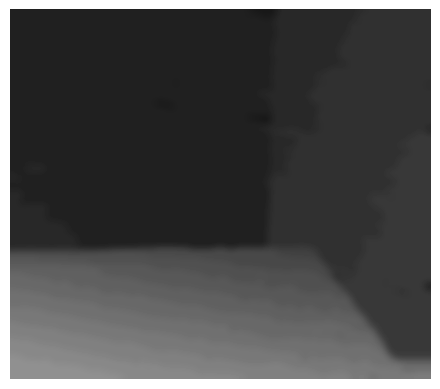}  & \includegraphics[width=\tableimagewidth, height=\tableimageheight]{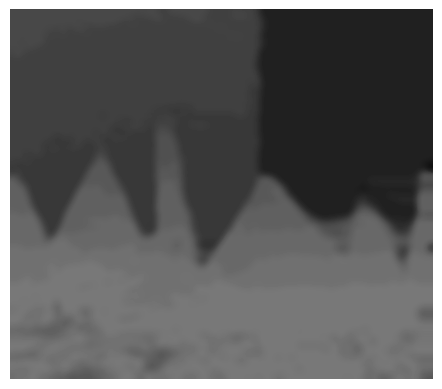} & \includegraphics[width=\tableimagewidth, height=\tableimageheight]{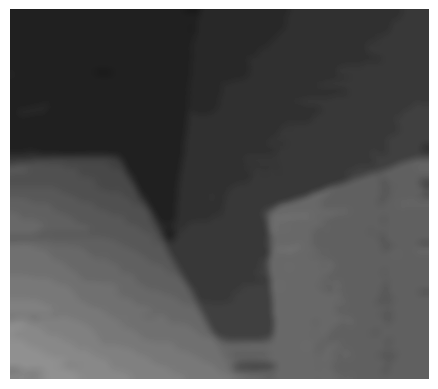}\\
       \rotatebox{90}{\textcolor{white}{------------}\textbf{NS2}} & \includegraphics[width=\tableimagewidth, height=\tableimageheight]{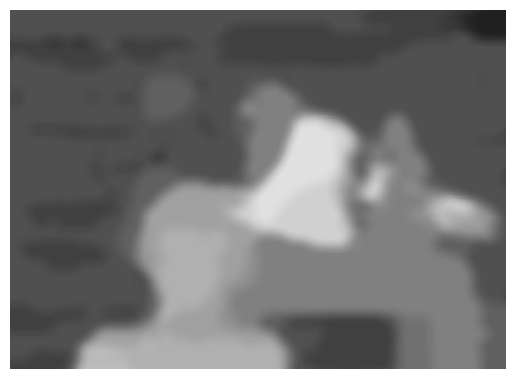} & \includegraphics[width=\tableimagewidth, height=\tableimageheight]{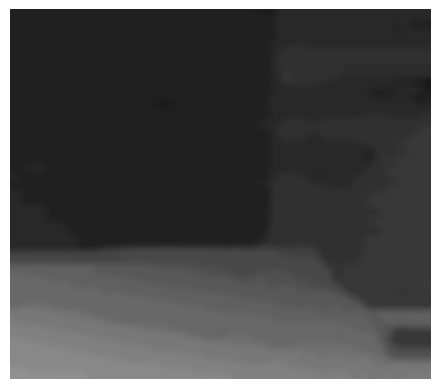}  & \includegraphics[width=\tableimagewidth, height=\tableimageheight]{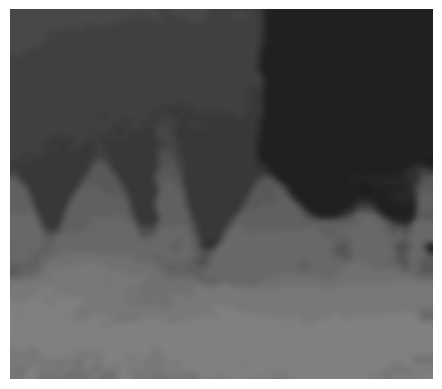} & \includegraphics[width=\tableimagewidth, height=\tableimageheight]{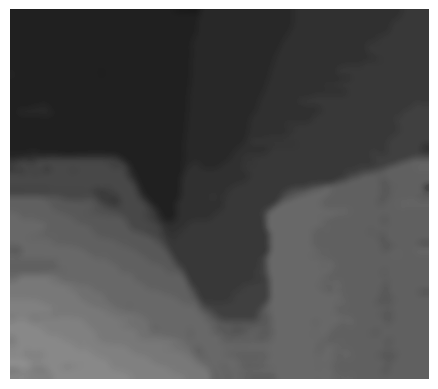}\\

    \end{tabular}
    \caption{By row: \textbf{G}round-\textbf{T}ruth displacements for each pair, our full method with \textbf{A}ll \textbf{S}teps, and  our method when the iteration step at the intermediate resolution is removed (\textbf{N}o \textbf{S}tep \textbf{2}). We can see that removing the second step means that some details are inaccurately estimated, such as a portion of the lamp in Tsukuba and planar regions in Venus. However, in the case of Sawtooth this lack of iterations and attention to details works to the algorithm's benefit. } 
    \label{fig:ablation_ctof}
\end{figure}
\section{Ablation Study on the Strength of the Rectifiers}\label{sec:rectifier_strength}
As discussed in Birdal \etal \cite{birdal2021quantum}, larger constraint values can negatively affect annealer performance. Therefore, we wanted to see if we can improve performance by decreasing these constraint values. What this means in practice is that we modify our QUBO matrix given in \cref{eq:quadratic_form_equals_markov_energy_with_granular_constraints} to the following:
\begin{equation}
\begin{split}
    \forall \vv \in \mathcal{V},\, \forall \lab{\vv}^l \in \mathcal{L}_\vv: & \,\, Q_{\lab{\vv}^l,\lab{\vv}^l} = \varphi_\vv(\lab{\vv}^l)  - t \cdot \Lambda(\lab{\vv}^l,\lab{\vv}^l) \\
    \forall \vp \in \mathcal{V},\, \forall \lab{\vp}^r,\lab{\vp}^s \in \mathcal{L}_\vp,\, r \neq s: & \,\, Q_{\lab{\vp}^r,\lab{\vp}^s} = t \cdot \Lambda(\lab{\vp}^r,\lab{\vp}^s) \\
    & \,\, Q_{\ell_\vp^j,\ell_\vp^i} = t \cdot \Lambda(\lab{\vp}^r,\lab{\vp}^s) \\
    \forall (\vp,\vq) \in E, \forall \ell_\vp^i \in \mathcal{L}_\vp \forall \ell_\vq^j \in \mathcal{L}_\vq: & \,\, Q_{\ell_\vp^i, \ell_\vq^j} = \frac{1}{2}\varphi_{\vp,\vq}(\ell_\vp^i,\ell_\vq^j) \\ 
      & \,\, Q_{ \ell_\vq^j, \ell_\vp^i} = \frac{1}{2}\varphi_{\vp,\vq}(\ell_\vp^i,\ell_\vq^j). \\
\end{split}
\label{eq:quadratic_form_equals_markov_energy_with_variable_rectifiers}
\end{equation}
Here, $t \geq 0$ can adjust the strength of our rectifiers. Our formulation in \cref{eq:quadratic_form_equals_markov_energy_with_granular_constraints} is a specialized case of \cref{eq:quadratic_form_equals_markov_energy_with_variable_rectifiers} where $t = 1$. For this experiment, we ran our stereo matching algorithm on the four Middlebury image pairs using all the default settings as described in \cref{sec:regularization_hyper_parameters}, while changing this newly introduced variable $t$. We show the visual results in \cref{fig:ablation_rectifier_strength} and numerical results in \cref{tab:our_sa_vary_t}. Note that in the case that two or more disparities are chosen during annealing, the lower disparity is chosen. In the case that no disparity was selected, the lowest possible disparity was selected. These experiments ran on D-Wave's simulated annealer. 

By graphing the of the average RMSE and BPP of these stereo estimates over $t$ (as shown in \cref{fig:rectifier_strength_graph}), we observe that lowering $t$ actually improves our results, with an optimum around $t = 0.25$, even though for this value, our constraints have not been formally proven to be obeyed. We also observe that some $t > 0$ is necessary to avoid the simulator returning the trivial answer of $0$. Given more time, we would like to investigate this performance improvement further to optimize $t$, and conduct experiments on the actual QPU.

\begin{table}[]
    \centering
    \begin{adjustbox}{width=\columnwidth,center}
    \begin{tabular}{|c| c | c || c | c || c | c || c | c || c | c || c | c || c | c |}
        \hline
        \multirow{2}{*}{\textbf{Image Pair}} &  \multicolumn{2}{ c ||}{$t = 0$ (\textbf{SA}) } & \multicolumn{2}{ c ||}{$t = 0.25$ (\textbf{SA})} & \multicolumn{2}{ c ||}{$t = 0.5$ (\textbf{SA})} &  \multicolumn{2}{ c ||}{$t = 0.75$ (\textbf{SA})} &  \multicolumn{2}{ c ||}{$t = 1$ (\textbf{SA})} &  \multicolumn{2}{ c ||}{$t = 1.25$ (\textbf{SA})} &  \multicolumn{2}{ c |}{$t = 1.5$ (\textbf{SA})} \\ \cline{2-15}
            & RMSE & BPP & RMSE & BPP & RMSE & BPP & RMSE & BPP & RMSE & BPP & RMSE & BPP & RMSE & BPP \\
            \hline
        \textbf{Tsukuba}  & 7.29  & 100 & 1.87  & 26.24 & 1.80  & 23.70  & 1.79 & 24.37 & 1.87 & 30.64 & 1.84 & 27.11 & 1.89 & 30.06\\ \hline
        \textbf{Bull}     & 8.29  & 100 & 1.30  & 24.28 & 1.42  & 31.59  & 1.97 & 38.53 & 1.87 & 45.29 & 2.10 & 43.74 & 2.21 & 48.11 \\ \hline
        \textbf{Sawtooth} & 10.72 & 100 & 2.86  & 38.09 & 2.84  & 46.84  & 2.98 & 53.85 & 3.04 & 56.75 & 3.23 & 59.50 & 3.22 & 60.96 \\ \hline
        \textbf{Venus}    & 9.39  & 100 & 2.04  & 36.73 & 2.12  & 42.35  & 2.26 & 47.83 & 2.27 & 47.73 & 2.35 & 50.28 & 2.56 & 53.71 \\ \hline
        \textbf{Average}  & 8.92  & 100 & \textbf{2.02}  & \textbf{31.34} & 2.05  & 36.12  & 2.25 & 41.15 & 2.26 & 45.10 & 2.38 & 45.16 & 2.47 & 48.21\\ \hline
        \end{tabular}
    \end{adjustbox}
    
    \caption{The Root Mean Squared Error (RMSE) and Bad Pixel Percentage (BPP) of the \textbf{S}imulated \textbf{A}nnealing method for increasing values of $t$. Lowering $t$ below $1$ can improve our metrics. }
    \label{tab:our_sa_vary_t}
\end{table}
\begin{figure}
    \centering
    \includegraphics[width=\graphimagewidth, height=\graphimageheight]{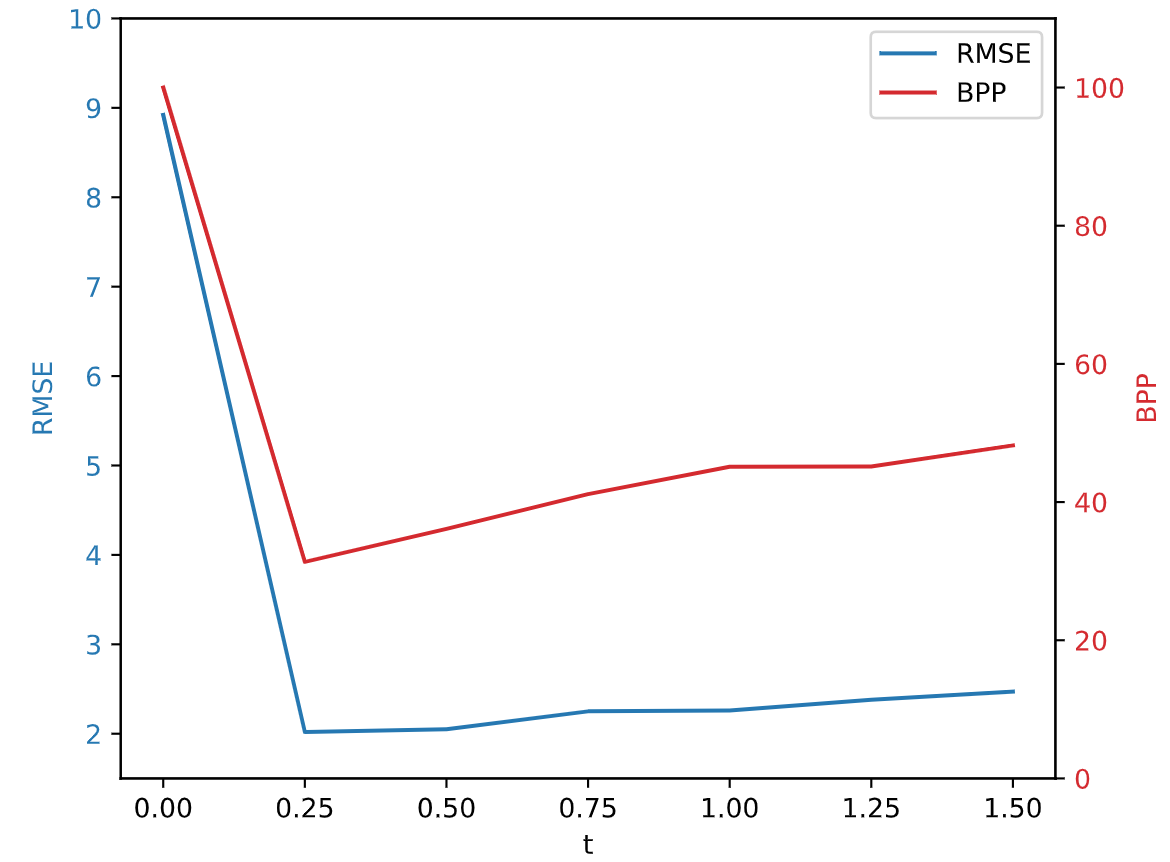}
    \caption{The average RMSE and BPP for the four Middlebury benchmarks over the rectifier strength $t$. We observe that both error metrics obtain a minimum around $t = 0.25$.} 
    \label{fig:rectifier_strength_graph}
\end{figure}

\begin{figure}
    \centering
    \setlength\tabcolsep{1.5pt}
    \begin{tabular}{c c c c c}
                   & Tsukuba & Bull & Sawtooth & Venus \\
       \rotatebox{90}{\textcolor{white}{-----.---}\textbf{GT}} & \includegraphics[width=\rectifiertableimagewidth, height=\rectifiertableimageheight]{sec/images/ground_truth_displacements/tsukuba.png} & \includegraphics[width=\rectifiertableimagewidth, height=\rectifiertableimageheight]{sec/images/ground_truth_displacements/bull.png}  & \includegraphics[width=\rectifiertableimagewidth, height=\rectifiertableimageheight]{sec/images/ground_truth_displacements/sawtooth.png} & \includegraphics[width=\rectifiertableimagewidth, height=\rectifiertableimageheight]{sec/images/ground_truth_displacements/venus.png}\\
       \rotatebox{90}{\textcolor{white}{----}$t = 0$ (\textbf{SA})} & \includegraphics[width=\rectifiertableimagewidth, height=\rectifiertableimageheight]{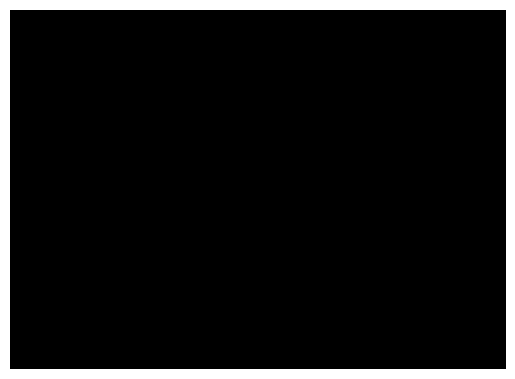} & \includegraphics[width=\rectifiertableimagewidth, height=\rectifiertableimageheight]{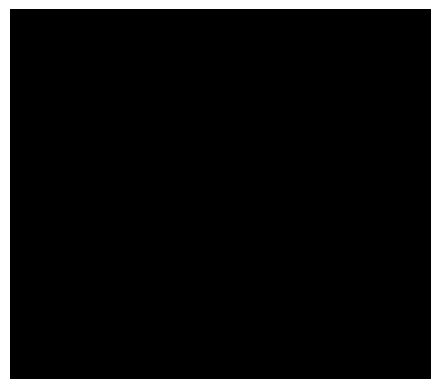}  & \includegraphics[width=\rectifiertableimagewidth, height=\rectifiertableimageheight]{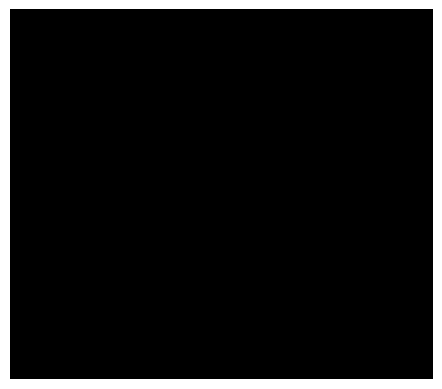} & \includegraphics[width=\rectifiertableimagewidth, height=\rectifiertableimageheight]{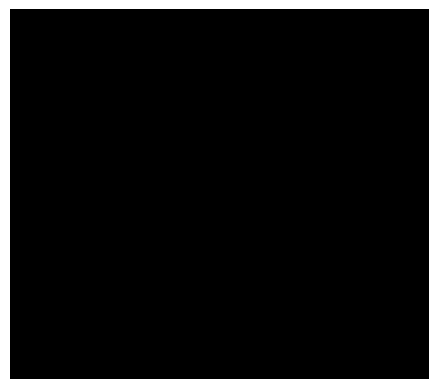}\\
       \rotatebox{90}{\textcolor{white}{--.}$t = 0.25$ (\textbf{SA})} & \includegraphics[width=\rectifiertableimagewidth, height=\rectifiertableimageheight]{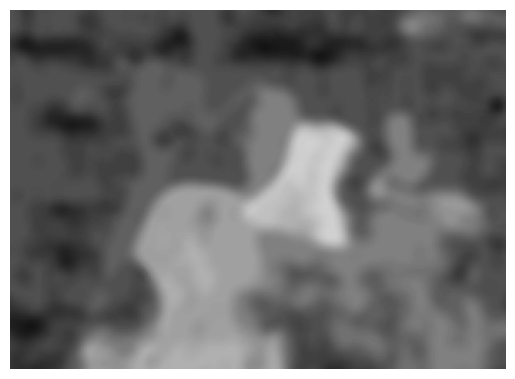} & \includegraphics[width=\rectifiertableimagewidth, height=\rectifiertableimageheight]{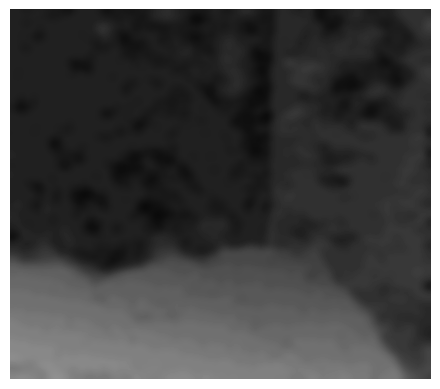}  & \includegraphics[width=\rectifiertableimagewidth, height=\rectifiertableimageheight]{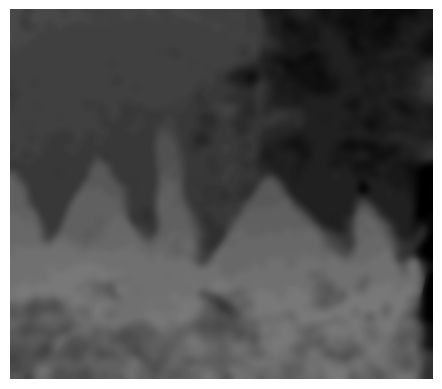} & \includegraphics[width=\rectifiertableimagewidth, height=\rectifiertableimageheight]{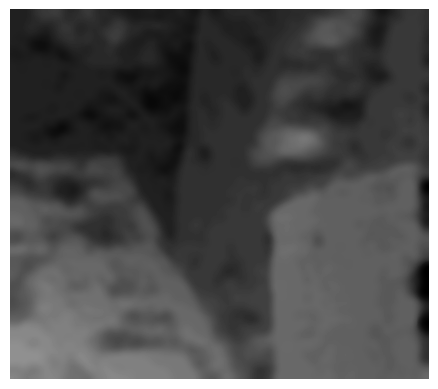}\\
       \rotatebox{90}{\textcolor{white}{---}$t = 0.5$ (\textbf{SA})} & \includegraphics[width=\rectifiertableimagewidth, height=\rectifiertableimageheight]{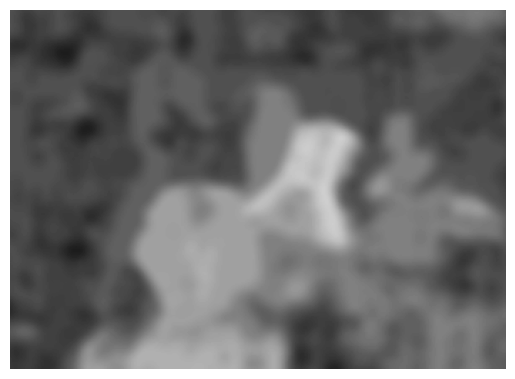} & \includegraphics[width=\rectifiertableimagewidth, height=\rectifiertableimageheight]{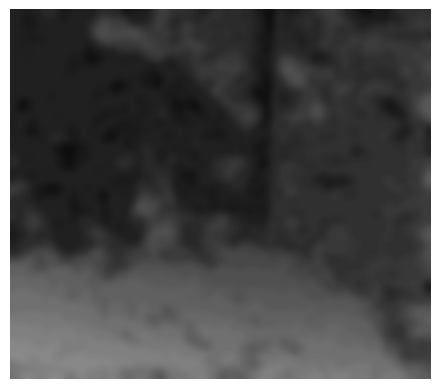}  & \includegraphics[width=\rectifiertableimagewidth, height=\rectifiertableimageheight]{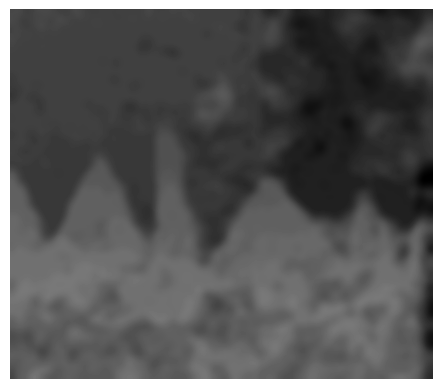} & \includegraphics[width=\rectifiertableimagewidth, height=\rectifiertableimageheight]{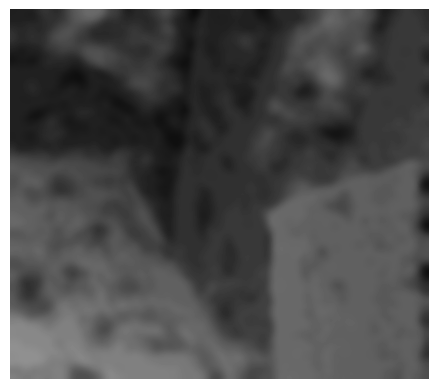}\\
       \rotatebox{90}{\textcolor{white}{--.}$t = 0.75$ (\textbf{SA})} & \includegraphics[width=\rectifiertableimagewidth, height=\rectifiertableimageheight]{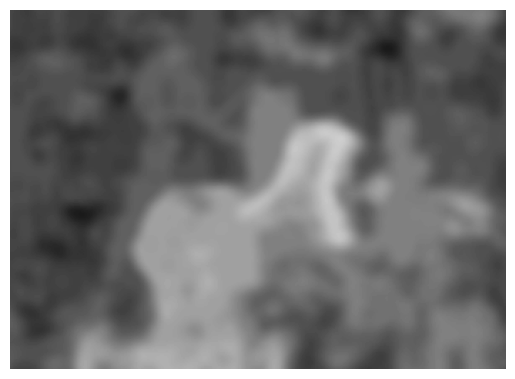} & \includegraphics[width=\rectifiertableimagewidth, height=\rectifiertableimageheight]{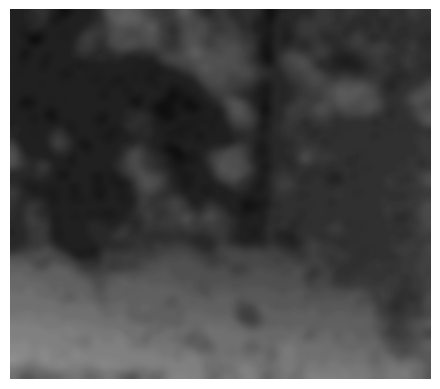}  & \includegraphics[width=\rectifiertableimagewidth, height=\rectifiertableimageheight]{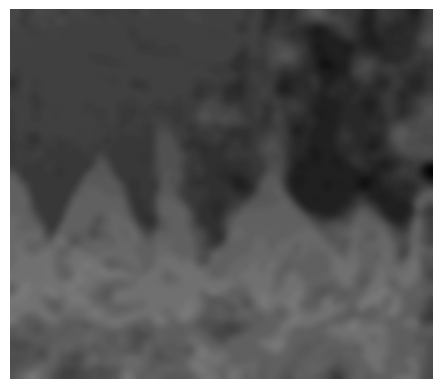} & \includegraphics[width=\rectifiertableimagewidth, height=\rectifiertableimageheight]{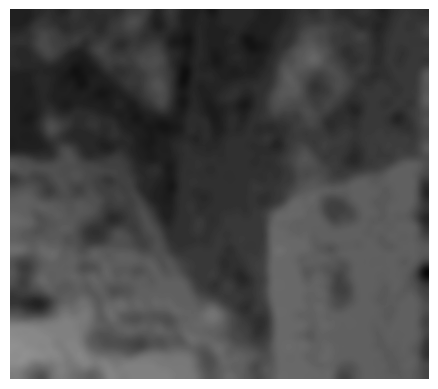}\\
       \rotatebox{90}{\textcolor{white}{----.}$t = 1$ (\textbf{SA})} & \includegraphics[width=\rectifiertableimagewidth, height=\rectifiertableimageheight]{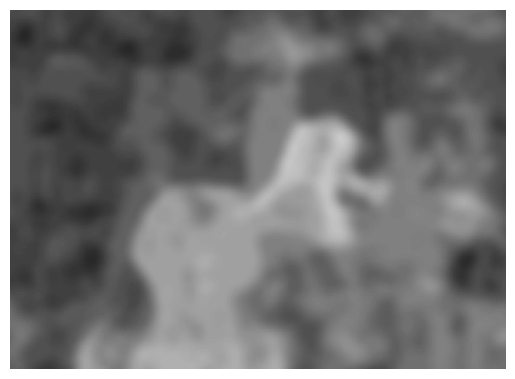} & \includegraphics[width=\rectifiertableimagewidth, height=\rectifiertableimageheight]{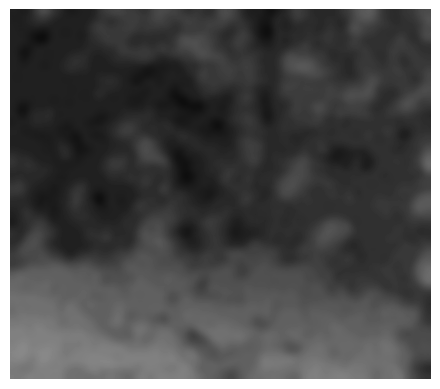}  & \includegraphics[width=\rectifiertableimagewidth, height=\rectifiertableimageheight]{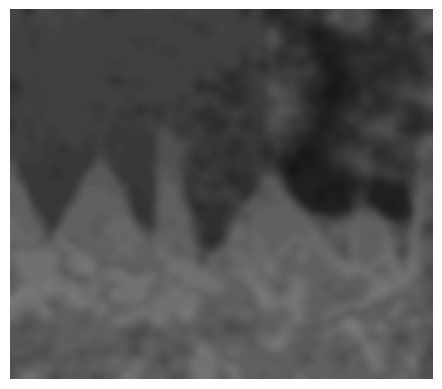} & \includegraphics[width=\rectifiertableimagewidth, height=\rectifiertableimageheight]{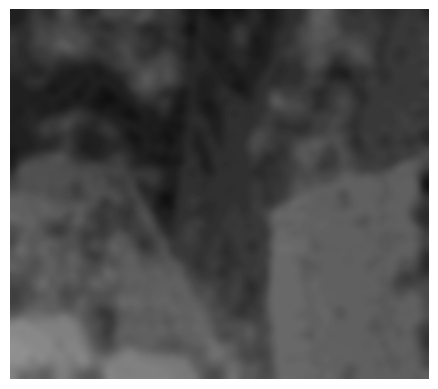}\\
       \rotatebox{90}{\textcolor{white}{--.}$t = 1.25$ (\textbf{SA})} & \includegraphics[width=\rectifiertableimagewidth, height=\rectifiertableimageheight]{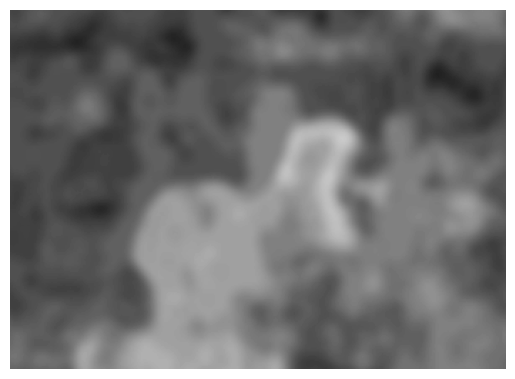} & \includegraphics[width=\rectifiertableimagewidth, height=\rectifiertableimageheight]{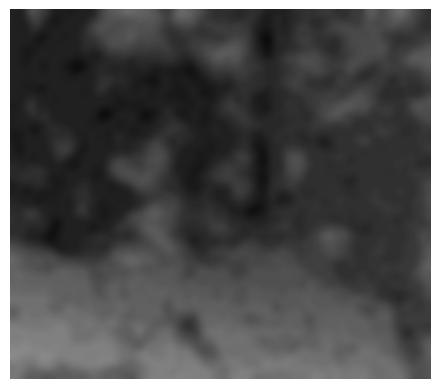}  & \includegraphics[width=\rectifiertableimagewidth, height=\rectifiertableimageheight]{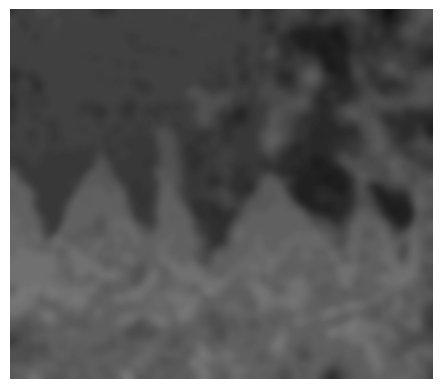} & \includegraphics[width=\rectifiertableimagewidth, height=\rectifiertableimageheight]{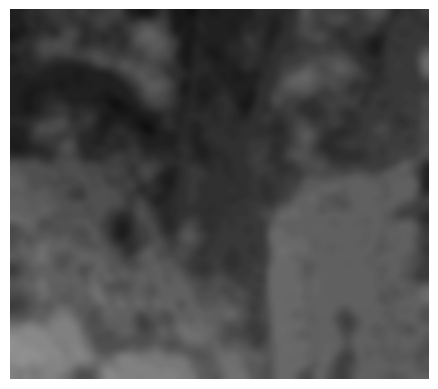}\\
       \rotatebox{90}{\textcolor{white}{---.}$t = 1.5$ (\textbf{SA})} & \includegraphics[width=\rectifiertableimagewidth, height=\rectifiertableimageheight]{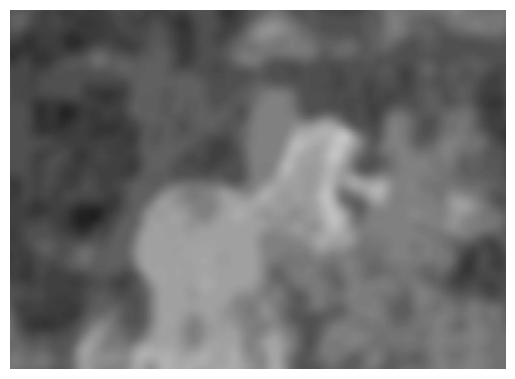} & \includegraphics[width=\rectifiertableimagewidth, height=\rectifiertableimageheight]{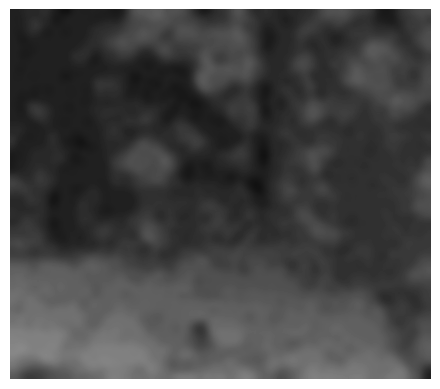}  & \includegraphics[width=\rectifiertableimagewidth, height=\rectifiertableimageheight]{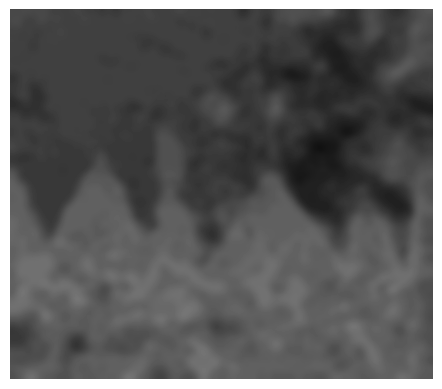} & \includegraphics[width=\rectifiertableimagewidth, height=\rectifiertableimageheight]{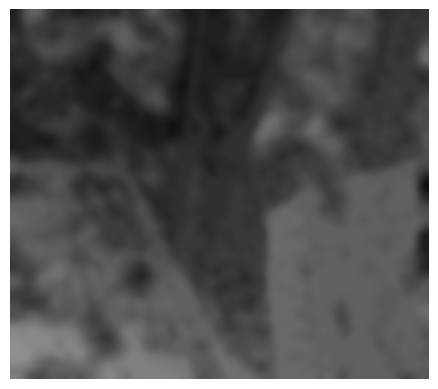}\\
    \end{tabular}
    \caption{\textbf{G}round-\textbf{T}ruth displacements compared with our \textbf{S}imulated \textbf{A}nnealing approach for increasing $t$ values.} 
    \label{fig:ablation_rectifier_strength}
\end{figure}
\section{Sintel Experiments} \label{sec:sintel_experiments}
We ran our model on several stereo image pairs from the  Sintel dataset \cite{Butler:ECCV:2012}. To account for the larger displacements present in the Sintel data, we adjusted our method to now have six coarse-to-fine levels in total. The full configuration of hyperparameters is given in \cref{tab:model_hyperparamters_sintel}. Visual results can be found in \cref{fig:sintel_results}, and numerical results can be found in \cref{tab:sintel_stats}. All estimates were done using Gurobi \cite{Gurobi2023}.

We observe that our method is capable of scaling up to larger image pairs with more complex scenes. In particular, stereo pairs with a continuous gradient of disparities, such as the walls in Alley 2, are estimated well. The method is also capable of picking out finer details, such as the ladder in the lower left section of Alley 2. At the same time, there are still some challenges. Small errors in coarser iterations compound into larger errors (observe the blotchy artifact in the upper right section of Alley 2, for example). The proposed approach also struggles with precision in detail-heavy foregrounds. For example, the hair in Alley 1 is missing some finer details. We suspect that in this case, the brightness constancy assumption is insufficient, and more advanced data terms could be investigated in the future. 

\begin{table}[]
    \centering
    %\begin{adjustbox}{width=\columnwidth,center}
    \begin{tabular}{|c| c | c | c | c | c | c | }
        \hline
        \textbf{Step} & \textbf{1} & \textbf{2}  & \textbf{3} & \textbf{4} & \textbf{5}  & \textbf{6}  \\ \hline\hline
        Downsample Factor (\cref{alg:full_quantum_algorithm}) & 32 & 16 & 8 & 4 & 2 & 1  \\ \hline
        Displacements Considered (\cref{alg:full_quantum_algorithm})  & 6 & 6 & 6 & 4 & 4 & 4 \\ \hline
        $\tau$ (\cref{eq:edge_aware_potts_model})  & 0.15 & 0.15 & 0.15 & 0.15 & 0.15 & 0.3  \\ \hline
        q (\cref{eq:edge_aware_potts_model})  & 10 & 10 & 10 & 10 & 10 & 10 \\ \hline
        m (\cref{eq:truncated_linear_regularizer})  &  0.0015 &  0.0015 & 0.0015 &  0.0015 & 0.0015 & $\infty$ \\ \hline
        s (\cref{eq:truncated_linear_regularizer}) & 0.0005  & 0.0005 & 0.0005 & 0.0005 & 0.0003 & 0.0005\\ \hline
        Median Filter Window (\cref{alg:full_quantum_algorithm}) & 3$\times$3 & 3$\times$3 & 3$\times$3 & 3$\times$3 & 3$\times$3 & 7$\times$7 \\ \hline
        Bilateral Filter Diameter (\cref{alg:full_quantum_algorithm}) & \textbf{n/a} & \textbf{n/a} & \textbf{n/a} & \textbf{n/a} & \textbf{n/a} & 12 \\ \hline
        Bilateral Filter Sigma Color (\cref{alg:full_quantum_algorithm}) & \textbf{n/a} & \textbf{n/a} & \textbf{n/a} & \textbf{n/a} & \textbf{n/a} & 75 \\ \hline 
        Bilateral Filter Sigma Space (\cref{alg:full_quantum_algorithm}) & \textbf{n/a} & \textbf{n/a} & \textbf{n/a} & \textbf{n/a} & \textbf{n/a} & 75 \\ \hline 
        \end{tabular}
    \caption{Hyperparameters for our stereo matching algorithm for the Sintel dataset \cite{Butler:ECCV:2012}.}
    \label{tab:model_hyperparamters_sintel}
\end{table}

\begin{figure}
    \centering
    \setlength\tabcolsep{1.5pt}
    \begin{tabular}{c c c c}
                & Alley 1 & Alley 2 & Sleeping 2 \\
        \rotatebox{90}{\textcolor{white}{--------}\textbf{LI}} & \includegraphics[width=\sinteltableimagewidth, height=\sinteltableimageheight]{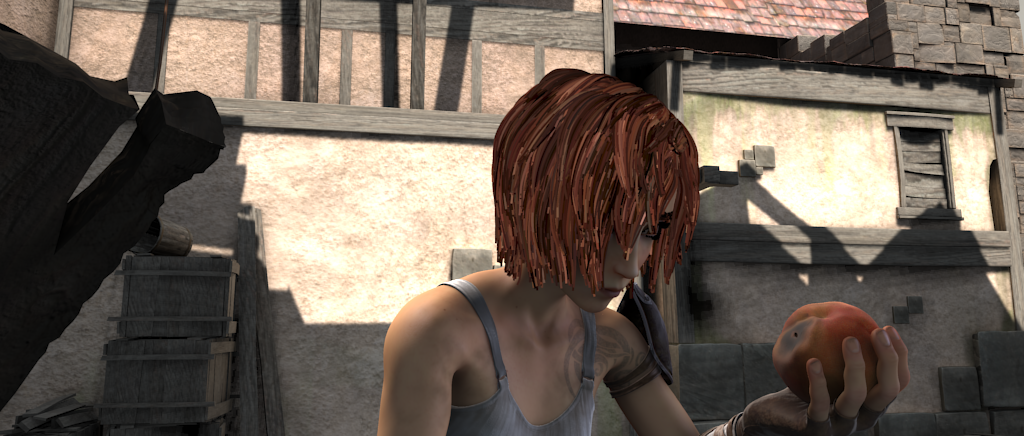} & \includegraphics[width=\sinteltableimagewidth, height=\sinteltableimageheight]{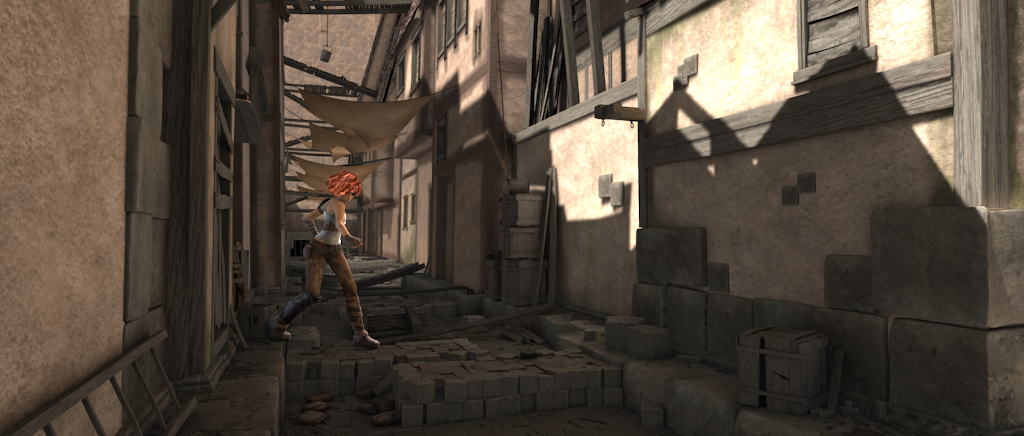}  & \includegraphics[width=\sinteltableimagewidth, height=\sinteltableimageheight]{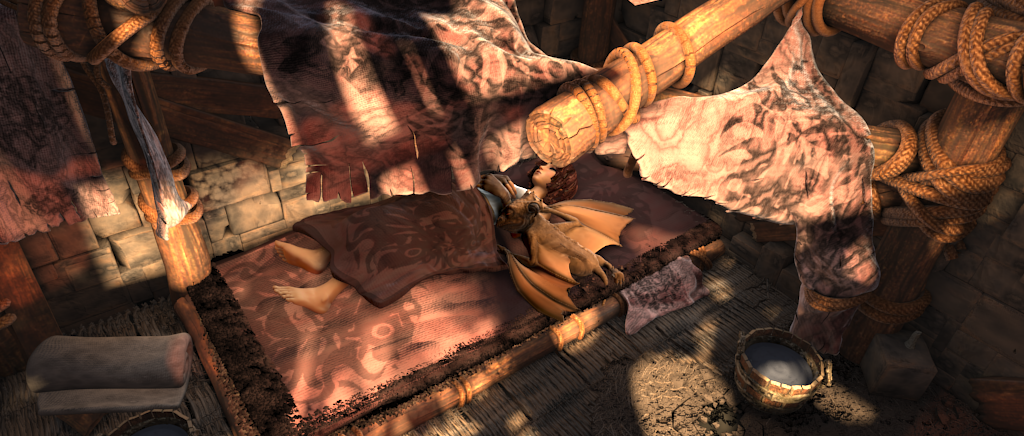} \\
       \rotatebox{90}{\textcolor{white}{---------}\textbf{GT}} & \includegraphics[width=\sinteltableimagewidth, height=\sinteltableimageheight]{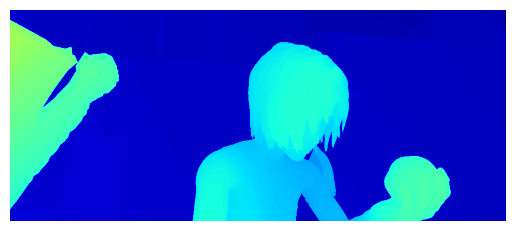} & \includegraphics[width=\sinteltableimagewidth, height=\sinteltableimageheight]{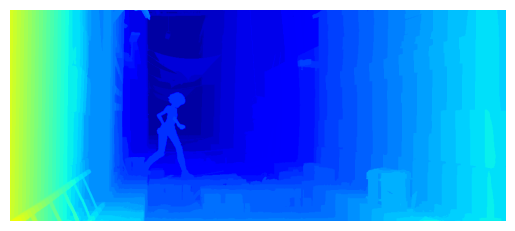}  & \includegraphics[width=\sinteltableimagewidth, height=\sinteltableimageheight]{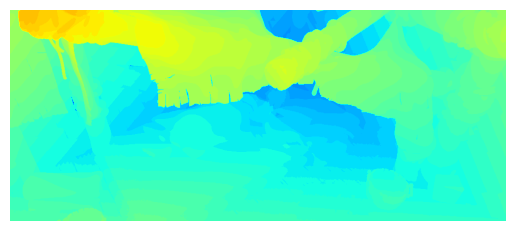} \\
       \rotatebox{90}{\textcolor{white}{------}Ours (\textbf{G})} & \includegraphics[width=\sinteltableimagewidth, height=\sinteltableimageheight]{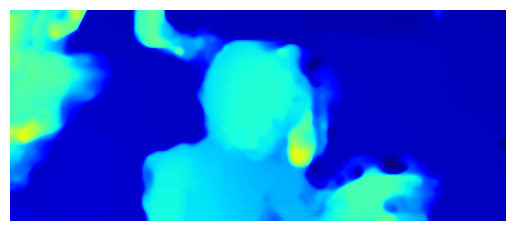} & \includegraphics[width=\sinteltableimagewidth, height=\sinteltableimageheight]{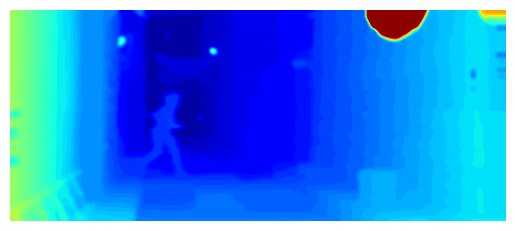}  & \includegraphics[width=\sinteltableimagewidth, height=\sinteltableimageheight]{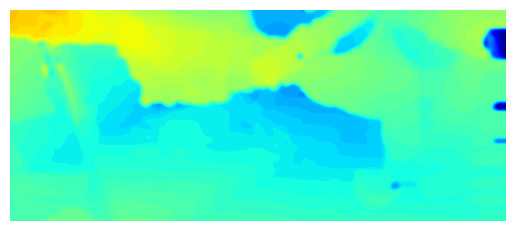} \\
                   & Temple 2 & Market 2 & Sleeping 1 \\
        \rotatebox{90}{\textcolor{white}{--------}\textbf{LI}} & \includegraphics[width=\sinteltableimagewidth, height=\sinteltableimageheight]{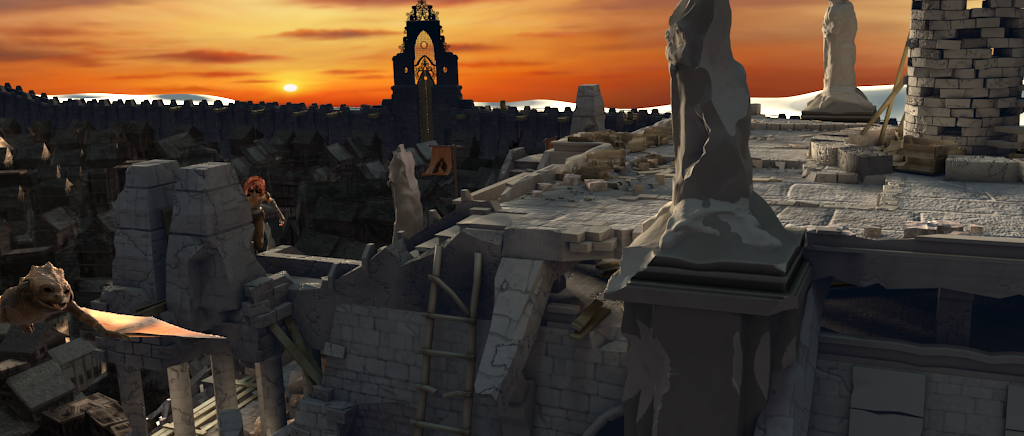} & \includegraphics[width=\sinteltableimagewidth, height=\sinteltableimageheight]{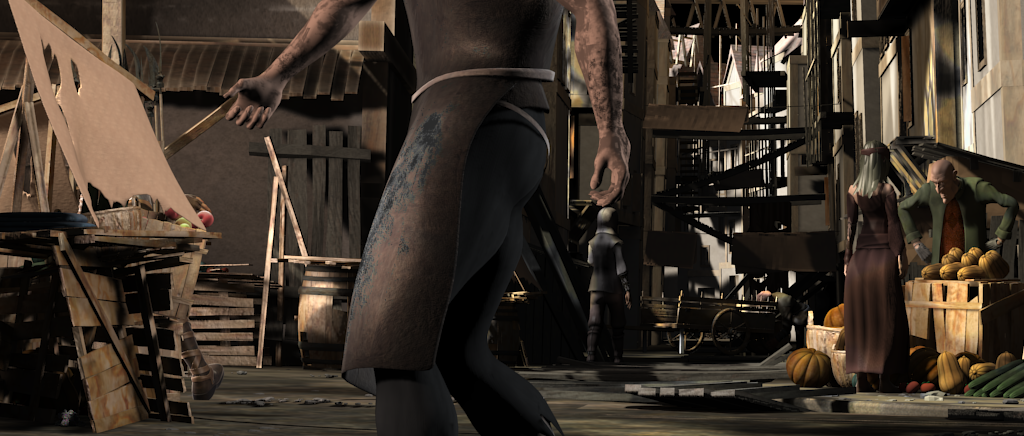}  & \includegraphics[width=\sinteltableimagewidth, height=\sinteltableimageheight]{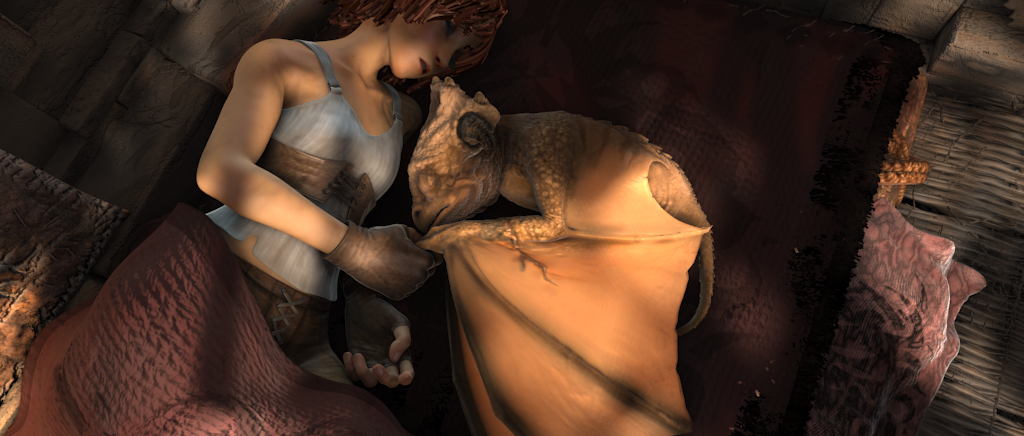} \\
       \rotatebox{90}{\textcolor{white}{---------}\textbf{GT}} & \includegraphics[width=\sinteltableimagewidth, height=\sinteltableimageheight]{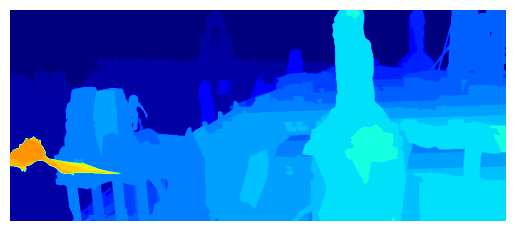} & \includegraphics[width=\sinteltableimagewidth, height=\sinteltableimageheight]{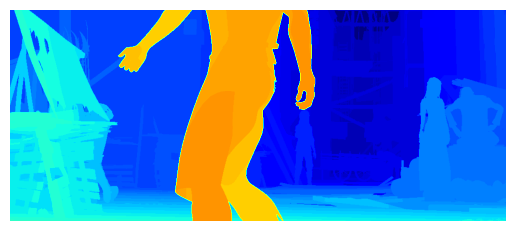}  & \includegraphics[width=\sinteltableimagewidth, height=\sinteltableimageheight]{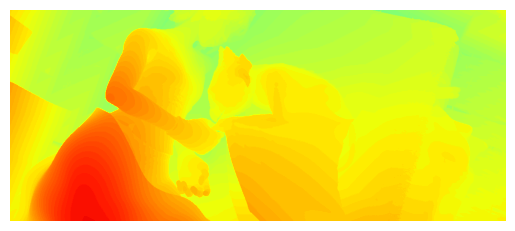} \\
       \rotatebox{90}{\textcolor{white}{------}Ours (\textbf{G})} & \includegraphics[width=\sinteltableimagewidth, height=\sinteltableimageheight]{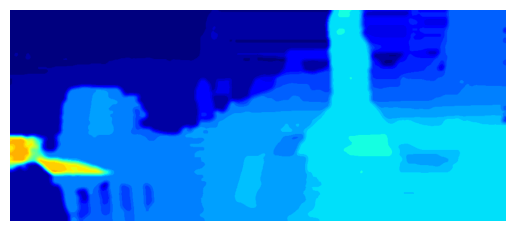} & \includegraphics[width=\sinteltableimagewidth, height=\sinteltableimageheight]{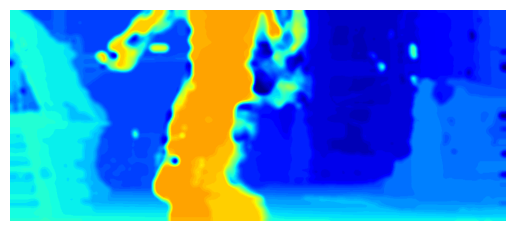}  & \includegraphics[width=\sinteltableimagewidth, height=\sinteltableimageheight]{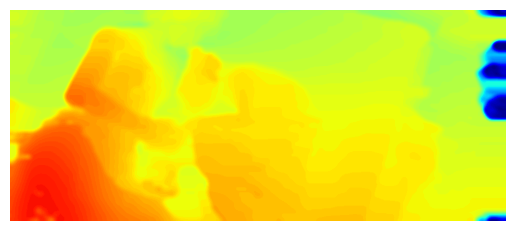} \\
    \end{tabular}
    \caption{The first and fourth rows show the \textbf{L}eft \textbf{I}mage from the first frame of the selected scenes of the Sintel stereo pairs. The second and fifth rows show the \textbf{G}round-\textbf{T}ruth displacements for each pair. The third and sixth rows show our stereo estimation approach using \textbf{G}urobi. We observe that our method can still make robust estimates, even though the input data is of higher resolution and more visually complex.} 
    \label{fig:sintel_results}
\end{figure}

\begin{table}[]
    \centering
    \begin{tabular}{|c| c | c |}
        \hline
        \multirow{2}{*}{\textbf{Image Pair}} &  \multicolumn{2}{ c |}{Ours (\textbf{G})} \\ \cline{2-3} 
            & RMSE & BPP \\
            \hline
        \textbf{Alley 1}    & 38.44 & 50.21  \\ \hline
        \textbf{Alley 2}    & 12.44 & 23.03  \\ \hline
        \textbf{Sleeping 2} &  3.47 & 20.23 \\ \hline
        \textbf{Temple 2}    &  1.88 & 10.30  \\ \hline
        \textbf{Market 2}    & 10.83 & 31.22  \\ \hline
        \textbf{Sleeping 1}  &  8.73 & 60.35  \\ \hline
        \end{tabular}
    
    \caption{The Root Mean Squared Error (RMSE) and Bad Pixel Percentage (BPP) of our method using \textbf{G}urobi on frame pairs from the Sintel dataset.} 
    \label{tab:sintel_stats}
\end{table}
\section{QUBO Matrix Visualization}
In this section, we examine the quantum annealing process on the first epipolar line on the Tsukuba image pair at the coarsest resolution. We first visualize the Ising model problem derived from the QUBO problem for stereo matching across this epipolar line. The Ising model problem attempts to minimize the following energy:
\begin{equation}
    H(s) = \sum_i h_i s_i + \sum_{i \neq j} J_{i,j} s_i s_j
\end{equation}
where each $s_i \in \{-1,1\}$ corresponds to the QUBO variable $\vx_i$ via the equation:
\begin{equation}
    s_i = 2\vx_i - 1
\end{equation}
and each $h_i$ is calculated from $Q= \{q_{i,j}\}$ as
\begin{equation}
    h_i = \frac{q_{ii}}{2} + \sum_{j \neq i} \frac{q_{i,j} + q_{j,i}}{4}
\end{equation}
and each $J_{i,j}$ is calculated as
\begin{equation}
    J_{i,j} = \frac{q_{i,j}}{4}
\end{equation}
The weights from the Ising model problem are directly translated into the QPU component's energies, therefore by visualizing these weights, one can better understand the energy landscape and topological complexity of the problem. To visualize these weights, we place them into a matrix with the diagonal is populated with $h_i$, and the off diagonal is populated with $J_{i,j}$. We then visualize the value of the matrix entries in \cref{fig:ising_matrix_visualization} 
\begin{figure}
    \centering
    \setlength\tabcolsep{1.5pt}
    \begin{tabular}{c}
        \includegraphics[width=\matrixvisualizationtableimagewidth, height=\matrixvisualizationtableimageheight]{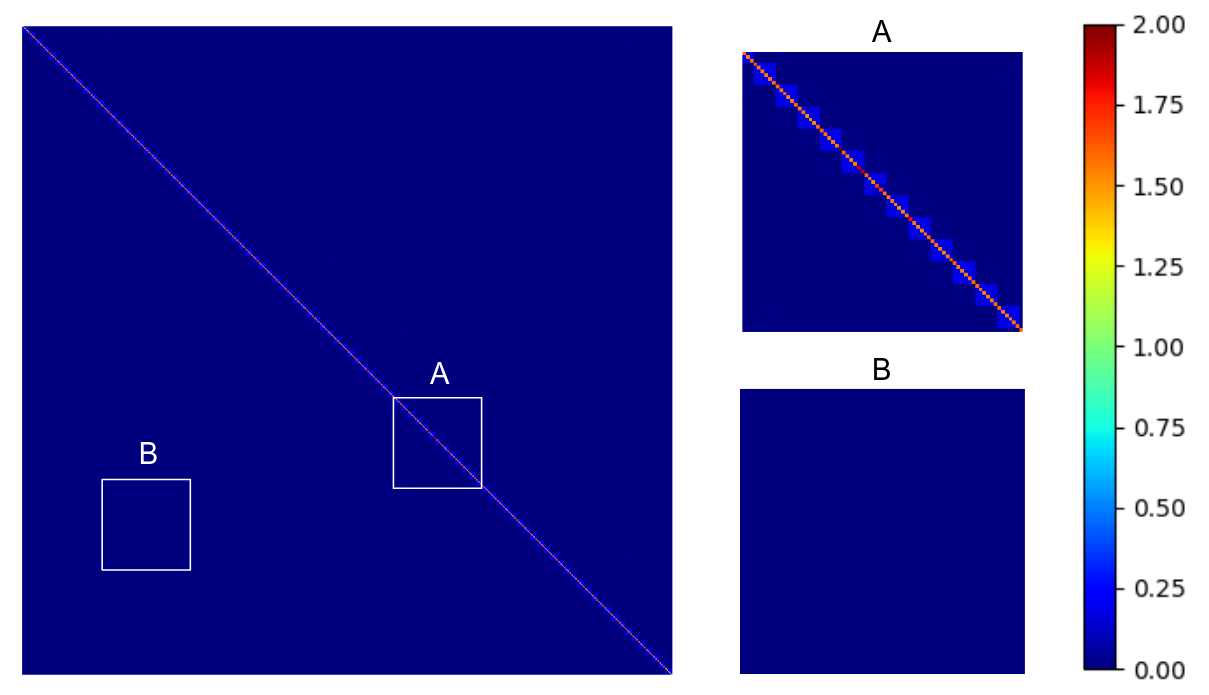} \\
    \end{tabular}
    \caption{The Ising model matrix's values visualized with a color mapping. The matrix has an observable pattern of $6 \times 6$ submatrices of higher values centered on the diagonal, is shown in the zoomed in section A. Each one of these $6 \times 6$ submatrices encodes the energy costs of selecting one of the $6$ possible labels for a particular pixel. The majority of the entries are $0$, as shown in the zoomed in section B. We scaled the entries of this matrix to be in the standard range accepted by the D-Wave QPUs, see \cite{SolverProperties}. The relative sparseness of the matrix means that it is easier to embed than a denser matrix (See \cref{sec:embedding_problem_graphs} for an in-depth discussion on embedding). We also observe that, of the non-zero entries, the highest entries are concentrated on the diagonal, and are significantly higher than other entries. This lack of balance between entries can exacerbate the minimum gap problem.} 
    \label{fig:ising_matrix_visualization}
\end{figure}

We also wanted to examine how the minimum gap was affected by the constraints, as we observed better annealing performance with lower constraints. To do so, we looked a small $10$ qubit subproblem from the first epipolar line of the Tsukuba image pair at the coarsest resolution. Beyond $10$ or so qubits makes it impossible to tractably calculate the Hamiltonian's eigenspectrum (the Hamiltonian grows exponentially with the number of qubits). We plotted the two lowest eigenvalues over time for this problem in \cref{fig:eigenvalues_over_time} for different constraint weights. We found that the hard constrained problem ($t=1$) had a minimum gap of $0.039$, while the soft constrained problem ($t=0.25$) had a minimum gap of $0.109$. Thus, we can see that the minimum gap problem is lessened when constraints are relaxed. We ran this experiment for the other Middlebury image pairs, see \cref{fig:additional_eigenvalues_over_time}

\begin{figure}
    \centering
    \setlength\tabcolsep{1.5pt}
    \begin{tabular}{c c}
        Hard Constraints & Soft Constraints \\
        \includegraphics[width=\eigenspectrumtableimagewidth, height=\eigenspectrumtableimageheight]{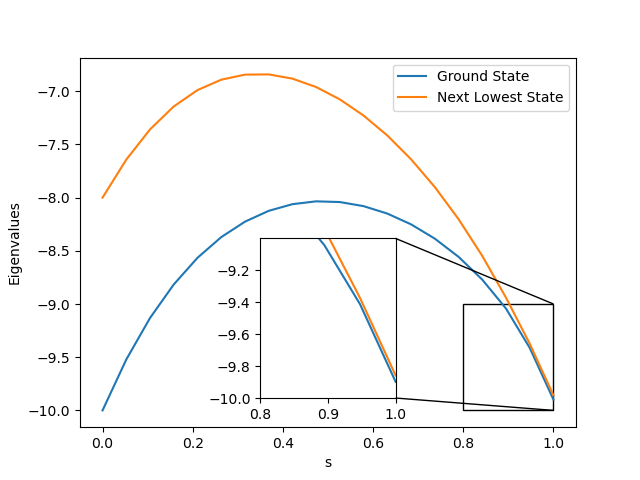} & \includegraphics[width=\eigenspectrumtableimagewidth, height=\eigenspectrumtableimageheight]{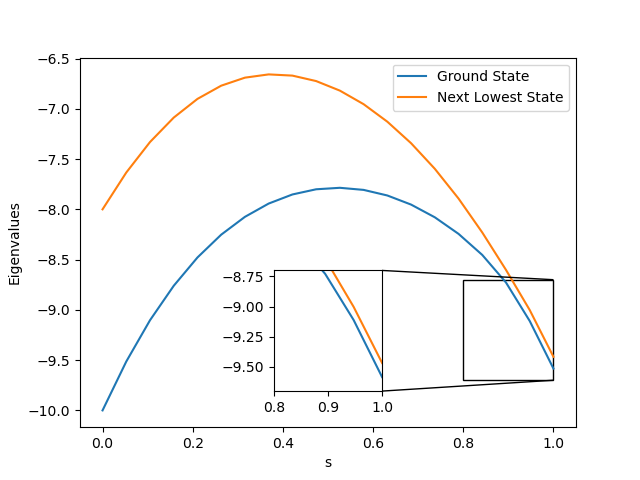}  \\
    \end{tabular}
    \caption{The two lowest value spectral lines of the Hamiltonian as it transitions from its initial state to the final state. We compare between a final problem Hamiltonian which enforces hard constraints ($t=1$), compared with a same final problem Hamiltonian using soft constraints ($t=0.25$), which had better performance on the simulated annealer. In both cases, the minimum gap occurs near the end of the annealing, but we can observe that this gap remains larger in the soft constraint case, which can help explain the improved annealing performance. The near convergence of the spectral lines as the Hamiltonian becomes our problem Hamiltonian also implies that the nature of this problem will be challenging to globally optimize on an annealer, even with softened constraints. Ideally, we would run an eigenspectrum analysis on the full epipolar line problem, however this is not computationally feasible. It is possible that with a larger problem, the difference in minimum gaps would be more pronounced.} 
    \label{fig:eigenvalues_over_time}
\end{figure}

\begin{figure}
    \centering
    \setlength\tabcolsep{1.5pt}
    
    \begin{tabular}{c c}
        Hard Constraints & Soft Constraints \\
        \includegraphics[width=\eigenspectrumtableimagewidth, height=\eigenspectrumtableimageheight]{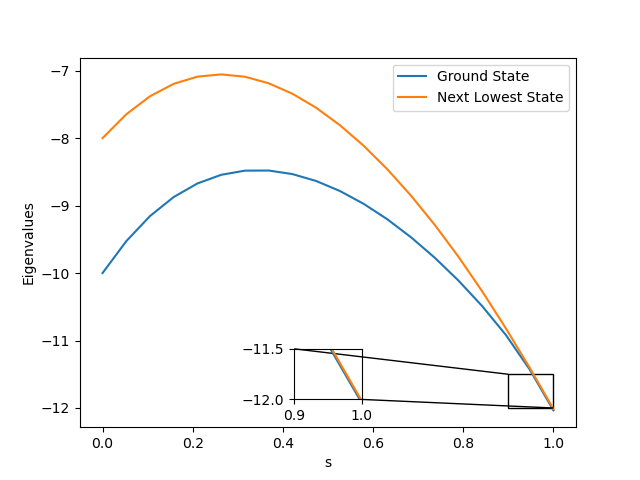} & \includegraphics[width=\eigenspectrumtableimagewidth, height=\eigenspectrumtableimageheight]{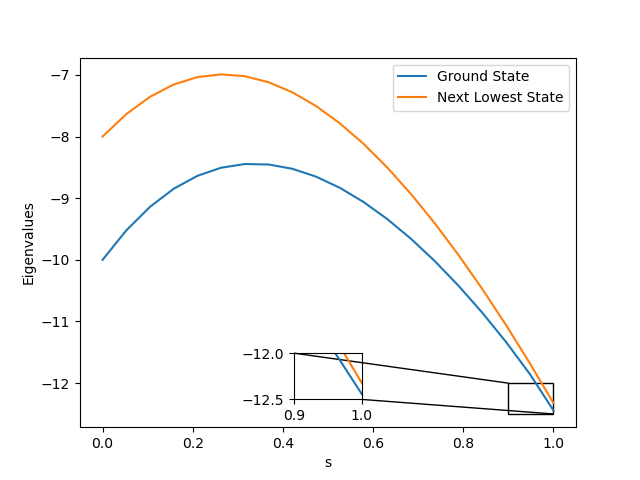} \\
        \includegraphics[width=\eigenspectrumtableimagewidth, height=\eigenspectrumtableimageheight]{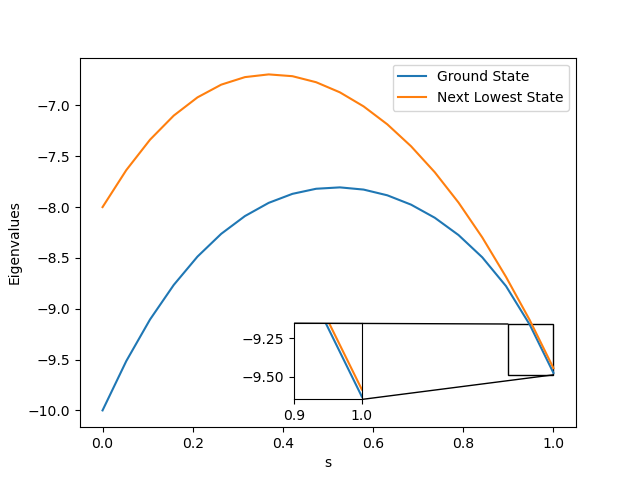} & \includegraphics[width=\eigenspectrumtableimagewidth, height=\eigenspectrumtableimageheight]{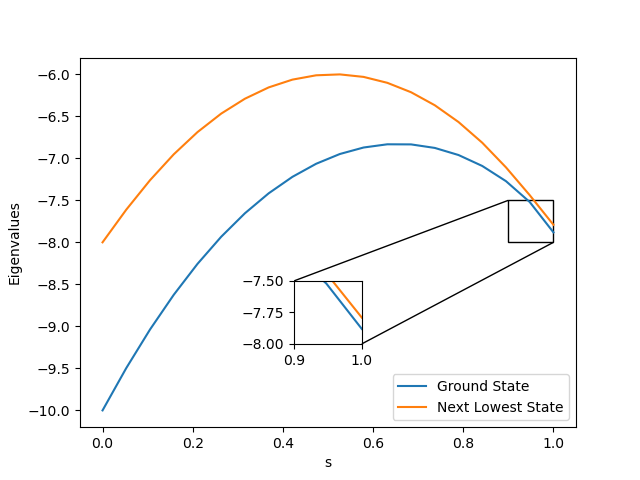}  \\
        \includegraphics[width=\eigenspectrumtableimagewidth, height=\eigenspectrumtableimageheight]{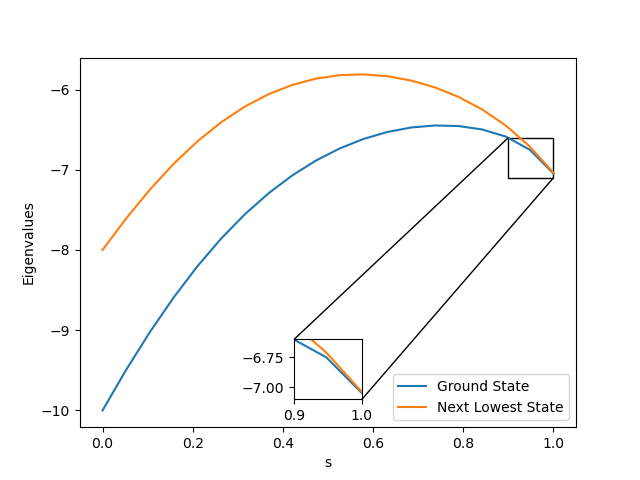} & \includegraphics[width=\eigenspectrumtableimagewidth, height=\eigenspectrumtableimageheight]{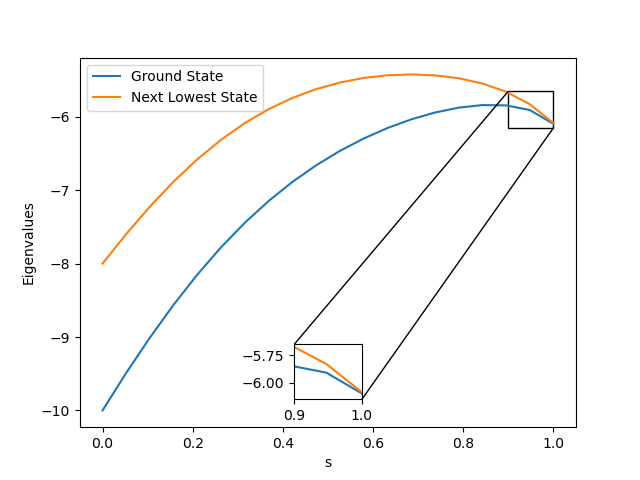}
    \end{tabular}
    \caption{The same experiment as in \cref{fig:eigenvalues_over_time}, only this time we consider the Bull, Sawtooth, and Venus image pairs (presented in that order top to bottom). We see that in all three of these cases, the minimum gap is always smaller in the $t=1$ case than in the $t=0.25$ case. For Bull, the difference is between $0.020$ and $0.119$. For Sawtooth, the difference is between $0.045$ and $0.081$. For Venus, the difference is between $0.001$ and $0.011$. This is further evidence that relaxing constraints shrinks the minimum gap 
    } 
    \label{fig:additional_eigenvalues_over_time}
\end{figure}
\section{Algorithm Diagrams}
We visualize the core of our algorithm in \cref{fig:algorithm_sketch}. This shows the image values along the epipolar lines of our images are processed by our algorithm, and ultimately influence the programming of the QPU.
\begin{figure}
    \begin{center}
        \includegraphics[width=\algorithmsketchwidth]{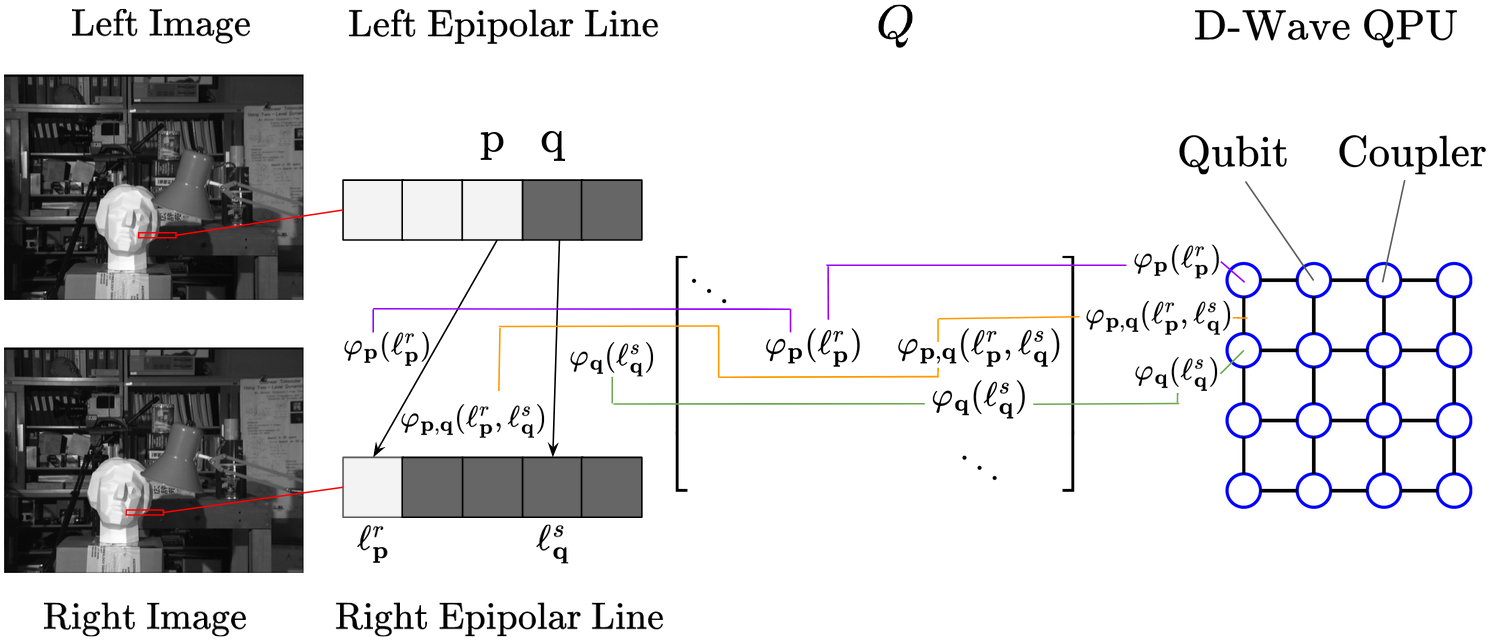}
    \end{center}
    \caption{Visualization of Our Algorithm: We zoom in on the corresponding epipolar lines (See \cref{subsec:stereo_matching_as_an_mrf}) for the Tsukuba image pair. For pixels with Markov variables $\vp$ and $\vq$, we consider their respective displacement labels $\lab{\vp}^r$ and $\lab{\vq}^s$ (See \cref{subsec:formulating_mrfs_as_qubos}). We classically calculate the data costs $\varphi_\vp(\lab{\vp}^r)$ and $\varphi_\vq(\lab{\vq}^s)$, and the regularization cost $\varphi_{\vp,\vq}(\lab{\vq}^s,\lab{\vp}^r)$. These values are then processed into the QUBO matrix $Q$ (See \cref{subsec:background}), which is then used to set the qubit and coupler energies on the D-Wave QPU (Also see \cref{subsec:background}). The diagram only sketches how these cost values calculated from the image pair are programmed into the QPU. Numerical details of the QUBO encoding scheme in $Q$ and minor embedding in the D-Wave QPU have been omitted for the sake of simplicity. 
    } 
    \label{fig:algorithm_sketch} 
\end{figure}
