# Supplementary material for: Quantum-Hybrid Stereo Matching With Nonlinear Regularization and Spatial Pyramids
Source: arXiv:2312.16118 source file (2024-12-06)
Supplement: Supplementary file 2 [file additional_qubo_matrix_visualization.tex]

\section{QUBO Matrix Visualization}
In this section, we examine the quantum annealing process on the first epipolar line on the Tsukuba image pair at the coarsest resolution. We first visualize the Ising model problem derived from the QUBO problem for stereo matching across this epipolar line. The Ising model problem attempts to minimize the following energy:
\begin{equation}
    H(s) = \sum_i h_i s_i + \sum_{i \neq j} J_{i,j} s_i s_j
\end{equation}
where each $s_i \in \{-1,1\}$ corresponds to the QUBO variable $\vx_i$ via the equation:
\begin{equation}
    s_i = 2\vx_i - 1
\end{equation}
and each $h_i$ is calculated from $Q= \{q_{i,j}\}$ as
\begin{equation}
    h_i = \frac{q_{ii}}{2} + \sum_{j \neq i} \frac{q_{i,j} + q_{j,i}}{4}
\end{equation}
and each $J_{i,j}$ is calculated as
\begin{equation}
    J_{i,j} = \frac{q_{i,j}}{4}
\end{equation}
The weights from the Ising model problem are directly translated into the QPU component's energies, therefore by visualizing these weights, one can better understand the energy landscape and topological complexity of the problem. To visualize these weights, we place them into a matrix with the diagonal is populated with $h_i$, and the off diagonal is populated with $J_{i,j}$. We then visualize the value of the matrix entries in \cref{fig:ising_matrix_visualization} 
\begin{figure}
    \centering
    \setlength\tabcolsep{1.5pt}
    \begin{tabular}{c}
        \includegraphics[width=\matrixvisualizationtableimagewidth, height=\matrixvisualizationtableimageheight]{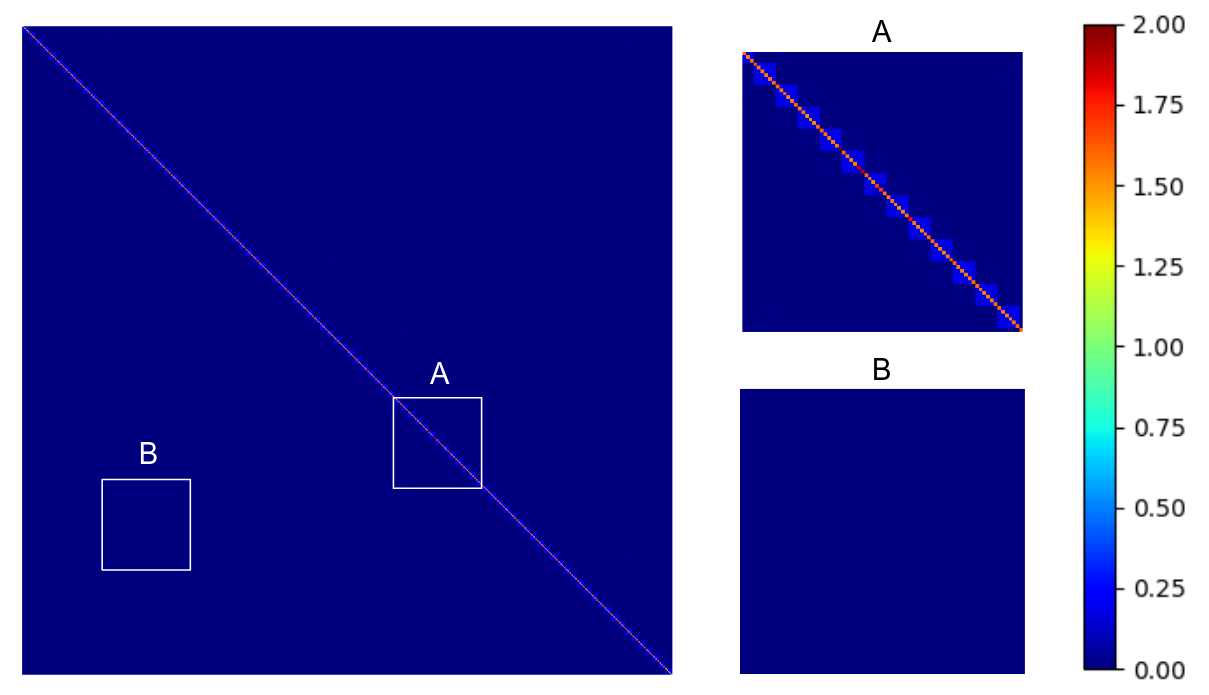} \\
    \end{tabular}
    \caption{The Ising model matrix's values visualized with a color mapping. The matrix has an observable pattern of $6 \times 6$ submatrices of higher values centered on the diagonal, is shown in the zoomed in section A. Each one of these $6 \times 6$ submatrices encodes the energy costs of selecting one of the $6$ possible labels for a particular pixel. The majority of the entries are $0$, as shown in the zoomed in section B. We scaled the entries of this matrix to be in the standard range accepted by the D-Wave QPUs, see \cite{SolverProperties}. The relative sparseness of the matrix means that it is easier to embed than a denser matrix (See \cref{sec:embedding_problem_graphs} for an in-depth discussion on embedding). We also observe that, of the non-zero entries, the highest entries are concentrated on the diagonal, and are significantly higher than other entries. This lack of balance between entries can exacerbate the minimum gap problem.} 
    \label{fig:ising_matrix_visualization}
\end{figure}

We also wanted to examine how the minimum gap was affected by the constraints, as we observed better annealing performance with lower constraints. To do so, we looked a small $10$ qubit subproblem from the first epipolar line of the Tsukuba image pair at the coarsest resolution. Beyond $10$ or so qubits makes it impossible to tractably calculate the Hamiltonian's eigenspectrum (the Hamiltonian grows exponentially with the number of qubits). We plotted the two lowest eigenvalues over time for this problem in \cref{fig:eigenvalues_over_time} for different constraint weights. We found that the hard constrained problem ($t=1$) had a minimum gap of $0.039$, while the soft constrained problem ($t=0.25$) had a minimum gap of $0.109$. Thus, we can see that the minimum gap problem is lessened when constraints are relaxed. We ran this experiment for the other Middlebury image pairs, see \cref{fig:additional_eigenvalues_over_time}

\begin{figure}
    \centering
    \setlength\tabcolsep{1.5pt}
    \begin{tabular}{c c}
        Hard Constraints & Soft Constraints \\
        \includegraphics[width=\eigenspectrumtableimagewidth, height=\eigenspectrumtableimageheight]{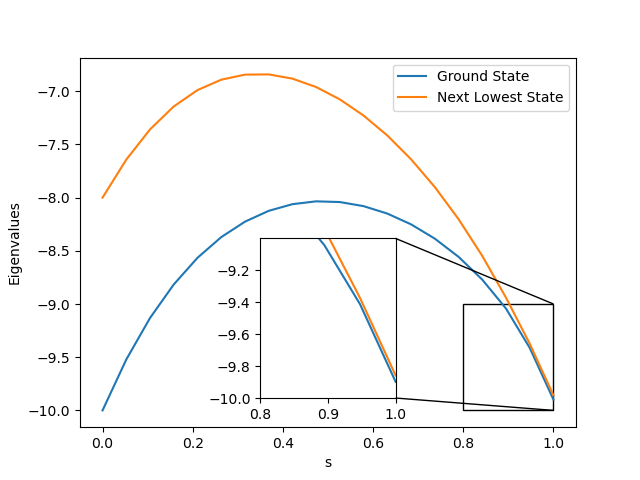} & \includegraphics[width=\eigenspectrumtableimagewidth, height=\eigenspectrumtableimageheight]{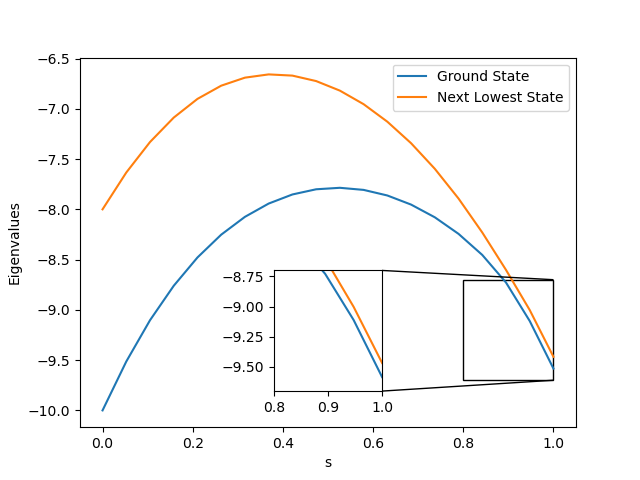}  \\
    \end{tabular}
    \caption{The two lowest value spectral lines of the Hamiltonian as it transitions from its initial state to the final state. We compare between a final problem Hamiltonian which enforces hard constraints ($t=1$), compared with a same final problem Hamiltonian using soft constraints ($t=0.25$), which had better performance on the simulated annealer. In both cases, the minimum gap occurs near the end of the annealing, but we can observe that this gap remains larger in the soft constraint case, which can help explain the improved annealing performance. The near convergence of the spectral lines as the Hamiltonian becomes our problem Hamiltonian also implies that the nature of this problem will be challenging to globally optimize on an annealer, even with softened constraints. Ideally, we would run an eigenspectrum analysis on the full epipolar line problem, however this is not computationally feasible. It is possible that with a larger problem, the difference in minimum gaps would be more pronounced.} 
    \label{fig:eigenvalues_over_time}
\end{figure}

\begin{figure}
    \centering
    \setlength\tabcolsep{1.5pt}
    
    \begin{tabular}{c c}
        Hard Constraints & Soft Constraints \\
        \includegraphics[width=\eigenspectrumtableimagewidth, height=\eigenspectrumtableimageheight]{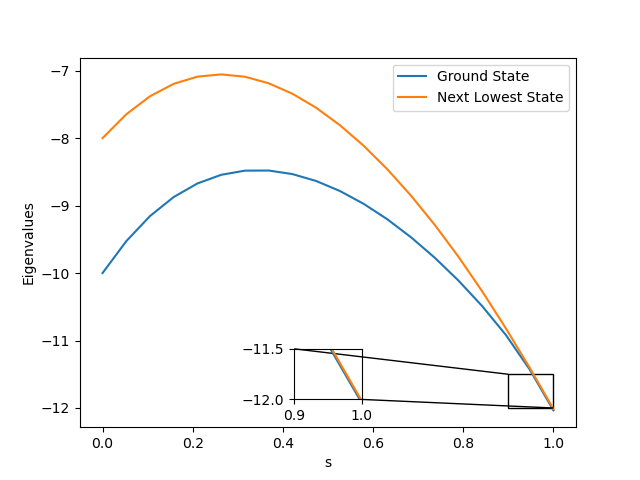} & \includegraphics[width=\eigenspectrumtableimagewidth, height=\eigenspectrumtableimageheight]{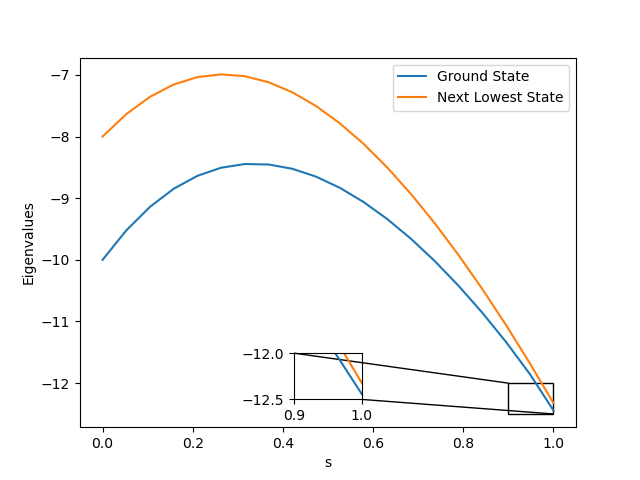} \\
        \includegraphics[width=\eigenspectrumtableimagewidth, height=\eigenspectrumtableimageheight]{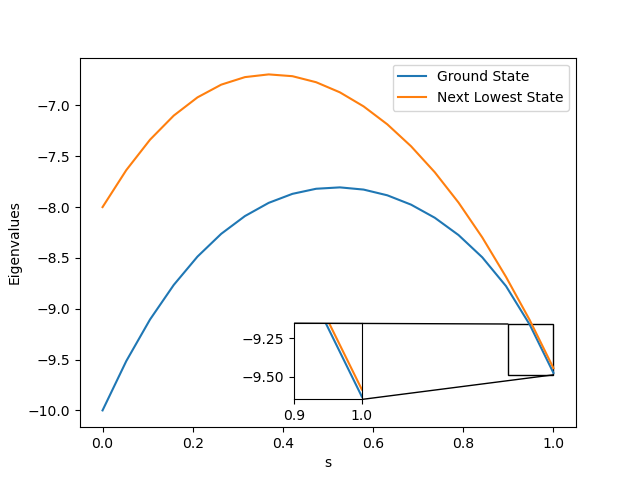} & \includegraphics[width=\eigenspectrumtableimagewidth, height=\eigenspectrumtableimageheight]{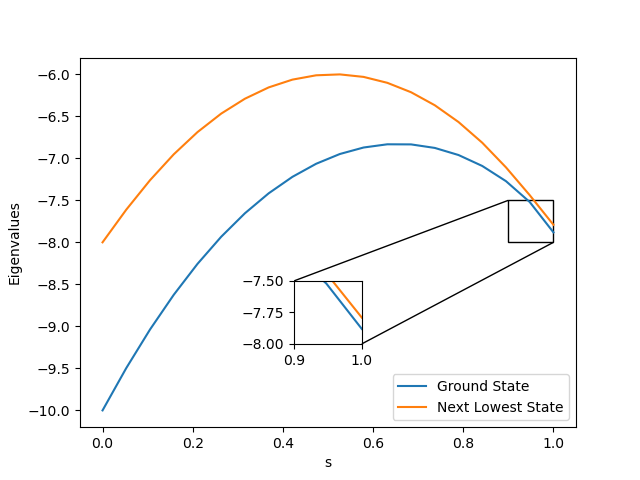}  \\
        \includegraphics[width=\eigenspectrumtableimagewidth, height=\eigenspectrumtableimageheight]{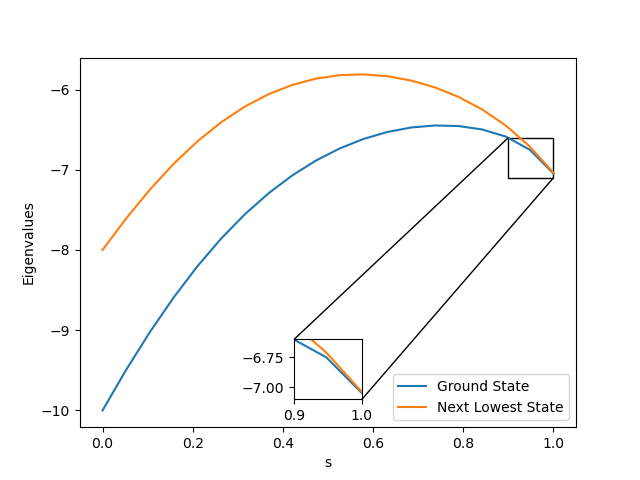} & \includegraphics[width=\eigenspectrumtableimagewidth, height=\eigenspectrumtableimageheight]{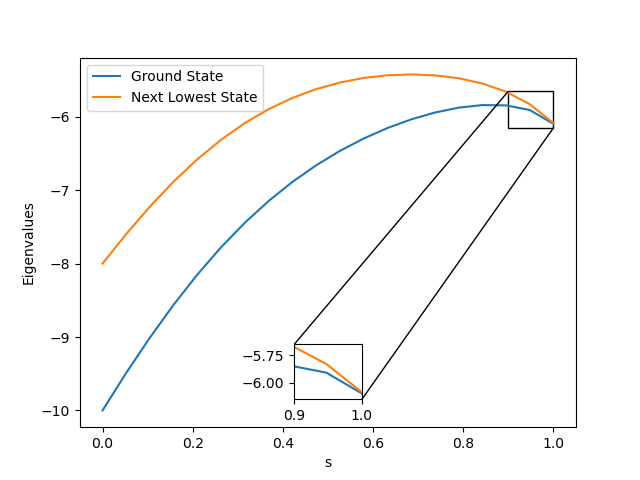}
    \end{tabular}
    \caption{The same experiment as in \cref{fig:eigenvalues_over_time}, only this time we consider the Bull, Sawtooth, and Venus image pairs (presented in that order top to bottom). We see that in all three of these cases, the minimum gap is always smaller in the $t=1$ case than in the $t=0.25$ case. For Bull, the difference is between $0.020$ and $0.119$. For Sawtooth, the difference is between $0.045$ and $0.081$. For Venus, the difference is between $0.001$ and $0.011$. This is further evidence that relaxing constraints shrinks the minimum gap 
    } 
    \label{fig:additional_eigenvalues_over_time}
\end{figure}
