# Supplementary material for: Quantum-Hybrid Stereo Matching With Nonlinear Regularization and Spatial Pyramids
Source: arXiv:2312.16118 source file (2024-12-06)
Supplement: Supplementary file 3 [file additional_sintel_images.tex]

\section{Bonus: Additional Sintel Experiments}
Here we are showing a few extra Sintel experiments (this is may be useful for  the rebuttal, but also to add into Cam's thesis). Visual results are in \cref{fig:additional_sintel_results}, and numerical results are in \cref{tab:additional_sintel_stats}

\begin{figure}
    \centering
    \setlength\tabcolsep{1.5pt}
    \begin{tabular}{c c c c}
                & Alley 1 & Alley 2 & Sleeping 2 \\
        \rotatebox{90}{\textcolor{white}{--------}\textbf{LI}} & \includegraphics[width=\sinteltableimagewidth, height=\sinteltableimageheight]{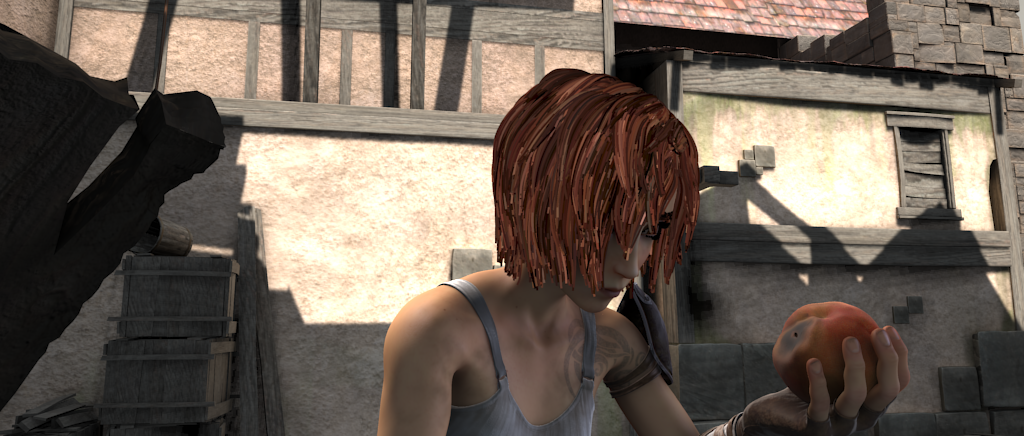} & \includegraphics[width=\sinteltableimagewidth, height=\sinteltableimageheight]{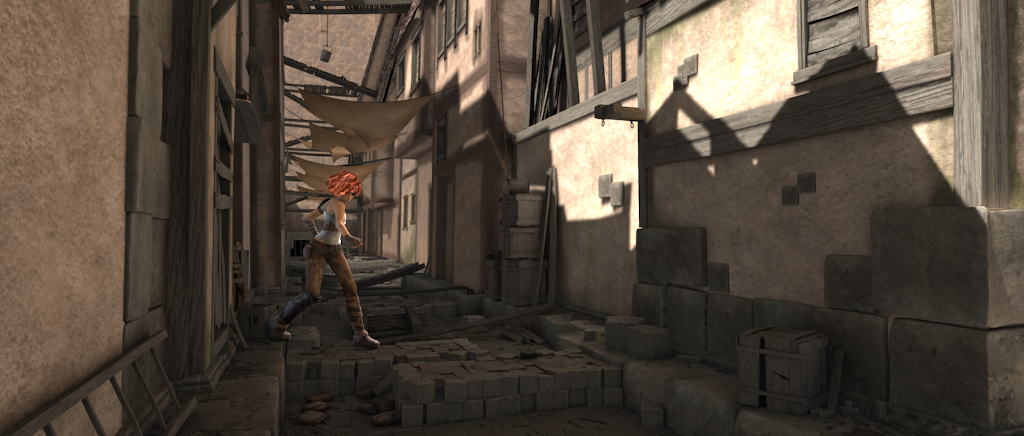}  & \includegraphics[width=\sinteltableimagewidth, height=\sinteltableimageheight]{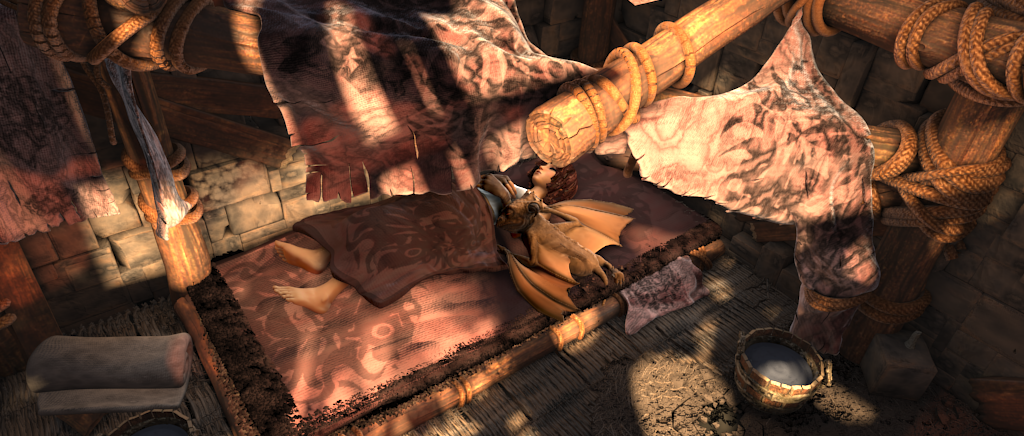} \\
       \rotatebox{90}{\textcolor{white}{---------}\textbf{GT}} & \includegraphics[width=\sinteltableimagewidth, height=\sinteltableimageheight]{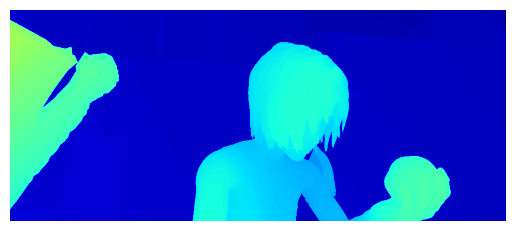} & \includegraphics[width=\sinteltableimagewidth, height=\sinteltableimageheight]{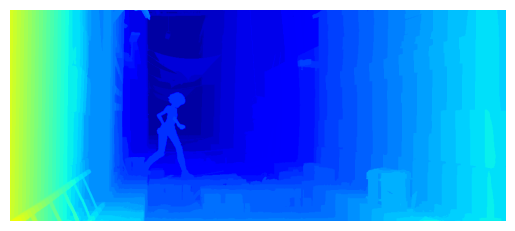}  & \includegraphics[width=\sinteltableimagewidth, height=\sinteltableimageheight]{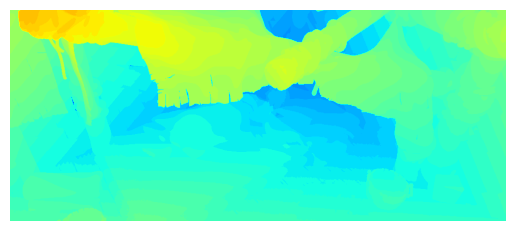} \\
       \rotatebox{90}{\textcolor{white}{------}Ours (\textbf{G})} & \includegraphics[width=\sinteltableimagewidth, height=\sinteltableimageheight]{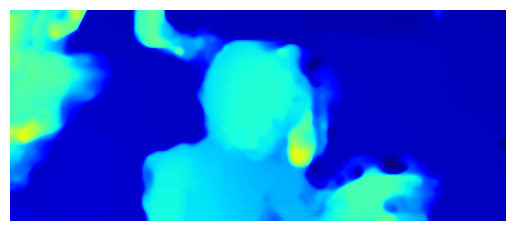} & \includegraphics[width=\sinteltableimagewidth, height=\sinteltableimageheight]{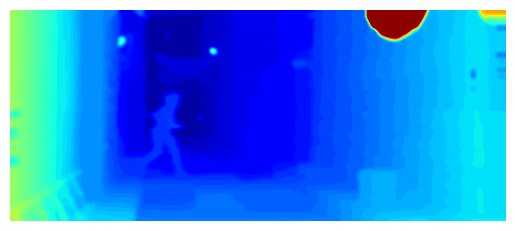}  & \includegraphics[width=\sinteltableimagewidth, height=\sinteltableimageheight]{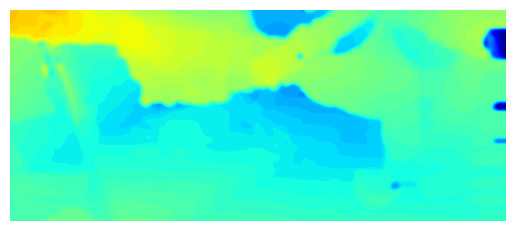} \\
                   & Temple 2 & Market 2 & Sleeping 1 \\
        \rotatebox{90}{\textcolor{white}{--------}\textbf{LI}} & \includegraphics[width=\sinteltableimagewidth, height=\sinteltableimageheight]{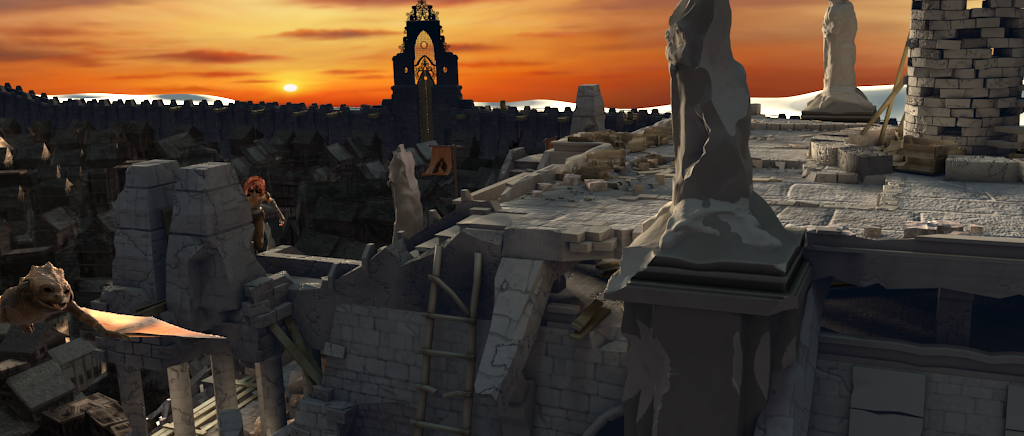} & \includegraphics[width=\sinteltableimagewidth, height=\sinteltableimageheight]{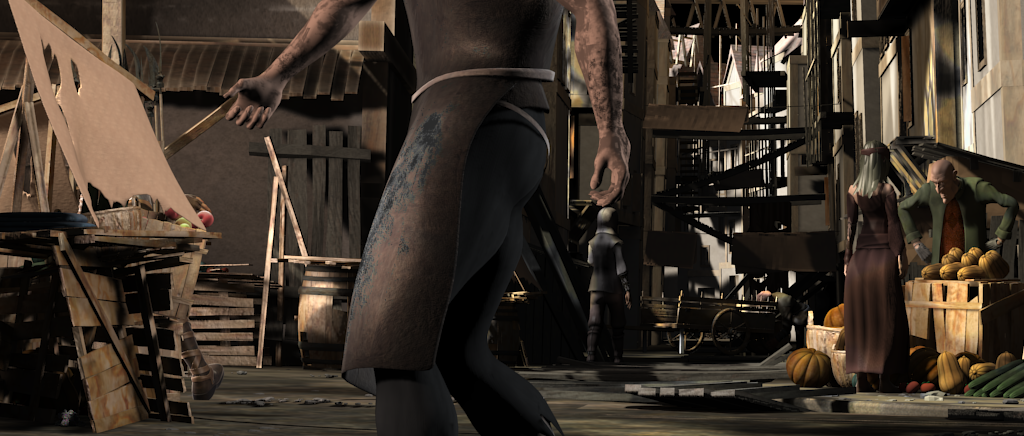}  & \includegraphics[width=\sinteltableimagewidth, height=\sinteltableimageheight]{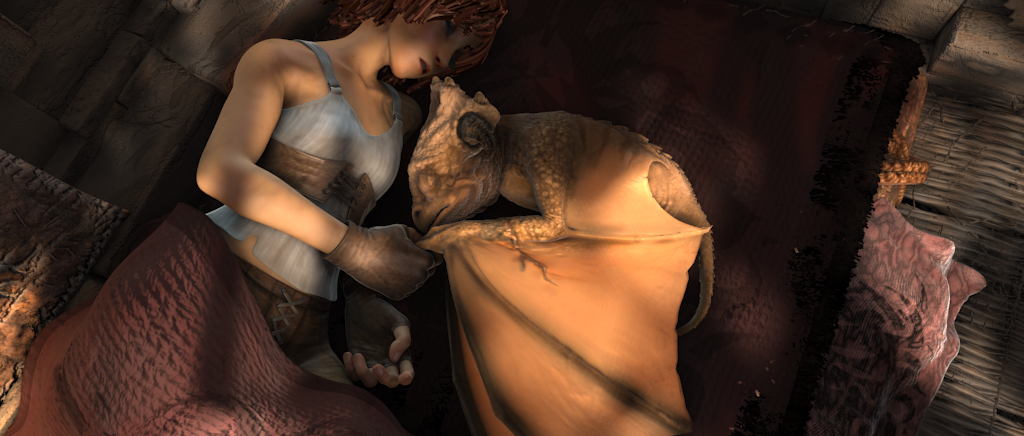} \\
       \rotatebox{90}{\textcolor{white}{---------}\textbf{GT}} & \includegraphics[width=\sinteltableimagewidth, height=\sinteltableimageheight]{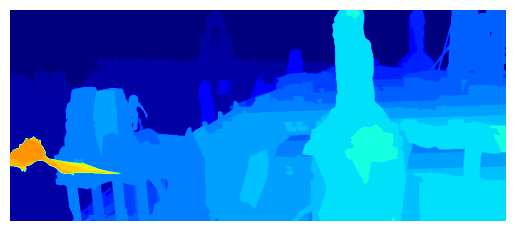} & \includegraphics[width=\sinteltableimagewidth, height=\sinteltableimageheight]{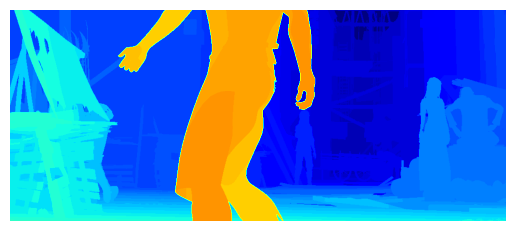}  & \includegraphics[width=\sinteltableimagewidth, height=\sinteltableimageheight]{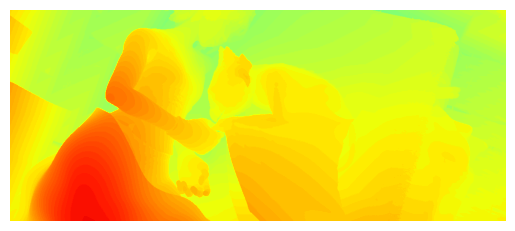} \\
       \rotatebox{90}{\textcolor{white}{------}Ours (\textbf{G})} & \includegraphics[width=\sinteltableimagewidth, height=\sinteltableimageheight]{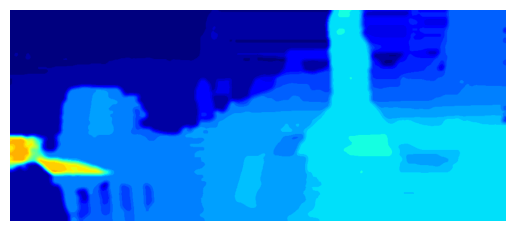} & \includegraphics[width=\sinteltableimagewidth, height=\sinteltableimageheight]{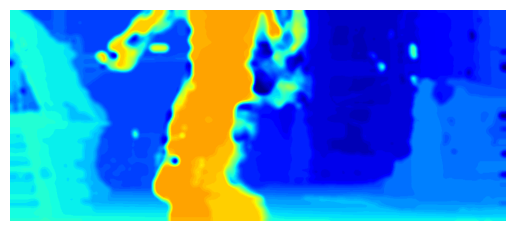}  & \includegraphics[width=\sinteltableimagewidth, height=\sinteltableimageheight]{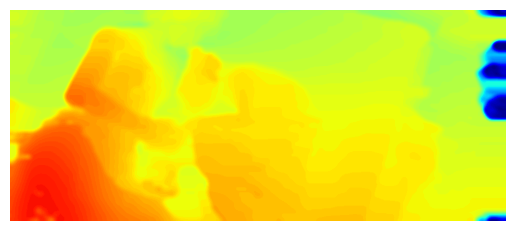} \\
    \end{tabular}
    \caption{The first row shows the \textbf{L}eft \textbf{I}mage from the first frame of the selected scenes of the Sintel stereo pairs. The second row shows the \textbf{G}round-\textbf{T}ruth displacements for each pair. The next row shows our stereo estimation approach using \textbf{G}urobi. We observe that our method can still make robust estimates, even though the input data is of higher resolution and more visually complex.} 
    \label{fig:additional_sintel_results}
\end{figure}

\begin{table}[]
    \centering
    \begin{tabular}{|c| c | c |}
        \hline
        \multirow{2}{*}{\textbf{Image Pair}} &  \multicolumn{2}{ c |}{Ours (\textbf{G})} \\ \cline{2-3} 
            & RMSE & BPP \\
            \hline
        \textbf{Alley 1}    & 38.44 & 50.21  \\ \hline
        \textbf{Alley 2}    & 12.44 & 23.03  \\ \hline
        \textbf{Sleeping 2} &  3.47 & 20.23 \\ \hline
        \textbf{Temple 2}    &  1.88 & 10.30  \\ \hline
        \textbf{Market 2}    & 10.83 & 31.22  \\ \hline
        \textbf{Sleeping 1}  &  8.73 & 60.35  \\ \hline
        \end{tabular}
    
    \caption{The Root Mean Squared Error (RMSE) and Bad Pixel Percentage (BPP) of our method using \textbf{G}urobi on their sequences from the Sintel dataset.} 
    \label{tab:additional_sintel_stats}
\end{table}
