# Supplementary material for: Quantum-Hybrid Stereo Matching With Nonlinear Regularization and Spatial Pyramids
Source: arXiv:2312.16118 source file (2024-12-06)
Supplement: Supplementary file 4 [file algorithm_diagrams.tex]

\section{Algorithm Diagrams}
We visualize the core of our algorithm in \cref{fig:algorithm_sketch}. This shows the image values along the epipolar lines of our images are processed by our algorithm, and ultimately influence the programming of the QPU.
\begin{figure}
    \begin{center}
        \includegraphics[width=\algorithmsketchwidth]{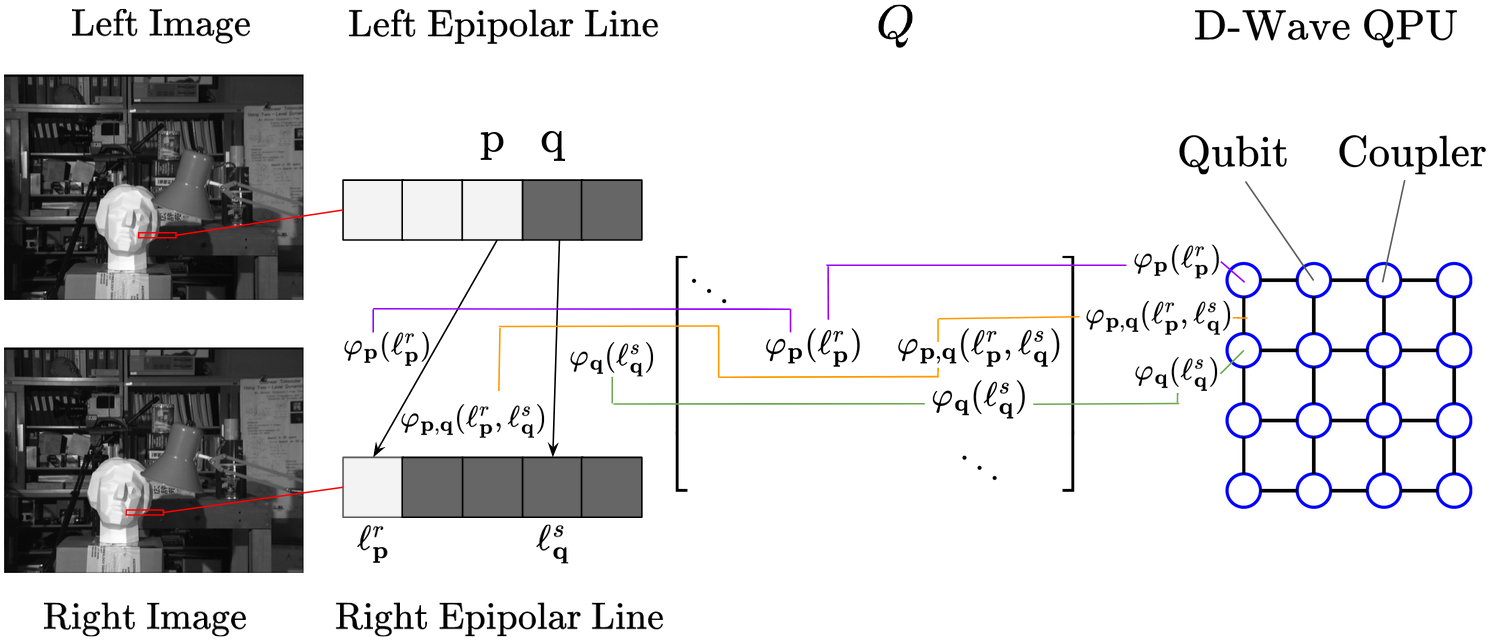}
    \end{center}
    \caption{Visualization of Our Algorithm: We zoom in on the corresponding epipolar lines (See \cref{subsec:stereo_matching_as_an_mrf}) for the Tsukuba image pair. For pixels with Markov variables $\vp$ and $\vq$, we consider their respective displacement labels $\lab{\vp}^r$ and $\lab{\vq}^s$ (See \cref{subsec:formulating_mrfs_as_qubos}). We classically calculate the data costs $\varphi_\vp(\lab{\vp}^r)$ and $\varphi_\vq(\lab{\vq}^s)$, and the regularization cost $\varphi_{\vp,\vq}(\lab{\vq}^s,\lab{\vp}^r)$. These values are then processed into the QUBO matrix $Q$ (See \cref{subsec:background}), which is then used to set the qubit and coupler energies on the D-Wave QPU (Also see \cref{subsec:background}). The diagram only sketches how these cost values calculated from the image pair are programmed into the QPU. Numerical details of the QUBO encoding scheme in $Q$ and minor embedding in the D-Wave QPU have been omitted for the sake of simplicity. 
    } 
    \label{fig:algorithm_sketch} 
\end{figure}
