# Supplementary material for: Quantum-Hybrid Stereo Matching With Nonlinear Regularization and Spatial Pyramids
Source: arXiv:2312.16118 source file (2024-12-06)
Supplement: Supplementary file 5 [file binary_encoding_of_MRF_MAP.tex]

\section{The Binary Encoding of MRF MAP Inference}\label{sec:binary_encoding_of_mrf_map}
\subsection{Encoding the MRF Energy as a High-Order Binary Polynomial}

Let $\operatorname{deg}(\vp)$ represent the degree of variable $\vp$, that is, how many variables are neighbors of $\vp$, and define:
\begin{equation} \label{f_def}
    f_{\vp,\vq}(\lab{\vp},\lab{\vq}) = \frac{\varphi_\vp(\ell_\vp)}{\operatorname{deg}(\vp)} + \varphi_{\vp,\vq}(\ell_\vp,\ell_\vq) + \frac{\varphi_\vq(\ell_\vq)}{\operatorname{deg}(\vq)} \,. 
\end{equation}
We can view the Markov cost function \cref{eq:MRF_energy} from a different perspective: 
\begin{equation} \label{eq:label_energy_full_sum}
    E(\ell_{(\cdot)}) = \sum_{(\vp,\vq) \in \mathcal{E}} f_{\vp,\vq}(\lab{\vp},\lab{\vq}) \,. 
\end{equation}

For every Markov variable $\vp$, we define our label space to be $\mathcal{L}_\vp = \{0, 1\}^n$, and we define binary variables $\{\vx_{\vp,0},...,\vx_{\vp,n}\}$. Each $\vx_{\vp,i}$ is flipped to $0$ or $1$, and the sequence $\vx_{\vp,0},...,x_{\vp,n}$ is a binary encoding of a label in $\mathcal{L}_\vp$. For label spaces whose size is not a power of $2$, we include extra labels to round the size up to the nearest power of $2$. The extra labels can be duplicates of the original labels. 

We will now represent $f_{\vp,\vq}$ as a polynomial of the binary variables $\{\vx_{\vp,0},...,\vx_{\vp,n}\}$, and $\{\vx_{\vq,0},...,\vx_{\vq,m}\}$. To construct this polynomial, we require the following notation: Let $(\sigma_\vp)_i$ be the $i^\text{th}$ entry of the binary string $\sigma_\vp \in \mathcal{\vp}$. Define:
\begin{align}
    \begin{split}
    \delta(\sigma_\vp, \vx_{\vp,i}) =
        \begin{cases}
            \vx_{\vp,i} & \text{if } (\sigma_\vp)_i = 1\\
            1, & \text{if } (\sigma_\vp)_i = 0 \,. 
        \end{cases}
    \end{split}
\end{align}
Then, $f_{\vp,\vq}$ is a polynomial of the following form: 
\begin{align} \label{eq:higher_order_binary_polynomial}
    f_{\vp,\vq}(\vx_{\vp,0},...,\vx_{\vp,n},\vx_{\vq,0},...,\vx_{\vp,m}) = \sum_{(\sigma_\vp,\sigma_\vq) \in \mathcal{L}_\vp \times \mathcal{L}_\vq} a_{\sigma_\vp,\sigma_\vq} (\Pi_{i \in 
 [1, ... , n]} \delta (\sigma_\vp,\vx_{\vp,i})) \cdot (\Pi_{j \in [1, ... , m]}\delta (\sigma_\vq,\vx_{\vq,j}))\,.
\end{align}
where the formula for $a_{\sigma_\vp,\sigma_\vq}$ is defined as follows: We order $\sigma'_\vp \leq \sigma_\vp$, if for every index $i$, $(\sigma'_\vp)_i \leq (\sigma_\vp)_i$. Additionally, we define $\kappa (\sigma_\vp)$ to be equal to the number of $1$'s present in $\kappa (\sigma_\vp)$. We can write $a_{\sigma_\vp,\sigma_\vq}$ as:
\begin{align} \label{eq:binary_encoding_coefficient_formula}
    a_{\sigma_\vp,\sigma_\vq} := \sum_{\sigma'_\vp \leq \sigma_\vp , \sigma'_\vq \leq \sigma_\vq}  (-1)^{\kappa(\sigma_\vp) + \kappa(\sigma_\vq)  - \kappa(\sigma'_\vp)  - \kappa(\sigma'_\vq)} f_{\vp,\vq}(\sigma'_\vp,\sigma'_\vq) \,. 
\end{align}
We now prove that this formula provides the correct coefficients for our polynomial.
\subsection{Proof of Coefficient Formula Correctness}
If we plug in the binary strings  $\vx_\vp \equiv \vx_{\vp,0},...,\vx_{\vp,n}$ and $\vx_\vq \equiv \vx_{\vq,0},...,\vx_{\vp,m}$ into \cref{eq:higher_order_binary_polynomial}, we obtain:
\begin{align}
    \begin{split}
        f_{\vp,\vq}(x_\vp,x_\vq)  & = \sum_{\sigma_\vp \leq x_\vp,\sigma_\vq \leq x_\vq} a_{\sigma_\vp,\sigma_\vq} \\
        & = \sum_{\sigma_\vp \leq x_\vp,\sigma_\vq \leq x_\vq} \sum_{\sigma'_\vp \leq \sigma_\vp , \sigma'_\vq \leq \sigma_\vq}  (-1)^{\kappa(\sigma_\vp) + \kappa(\sigma_\vq)  - \kappa(\sigma'_\vp)  - \kappa(\sigma'_\vq)} f_{\vp,\vq}(\sigma'_\vp,\sigma'_\vq) \\
        & = \sum_{\sigma'_\vp \leq x_\vp,\sigma'_\vq \leq x_\vq} f_{\vp,\vq}(\sigma'_\vp,\sigma'_\vq) \sum_{\sigma'_\vp \leq \sigma_\vp \leq x_\vp , \sigma'_\vq \leq \sigma_\vq \leq x_\vq}  (-1)^{\kappa(\sigma_\vp) + \kappa(\sigma_\vq)  - \kappa(\sigma'_\vp)  - \kappa(\sigma'_\vq)} \,.
    \end{split}
\end{align}
We now focus on simplifying the inner term: 
\begin{align}
    \begin{split} \label{eq:combinatorial_sum_term}
    \sum_{\sigma'_\vp \leq \sigma_\vp \leq x_\vp , \sigma'_\vq \leq \sigma_\vq \leq x_\vq}  (-1)^{\kappa(\sigma_\vp) + \kappa(\sigma_\vq)  - \kappa(\sigma'_\vp)  - \kappa(\sigma'_\vq)} \,. 
    \end{split}
\end{align}
We can regroup this sum into terms with different values of $\kappa(\sigma'_\vp) + \kappa(\sigma'_\vq)$. From combinatorics, we know that there are exactly $\binom{ \kappa(x_\vp) + \kappa(x_\vq) - \kappa(\sigma'_\vp) - \kappa(\sigma'_\vq) }{k - \kappa(\sigma'_\vp) - \kappa(\sigma'_\vq) }$ pairs of binary strings $\sigma_\vp$, $\sigma_\vq$ such that $\kappa(\sigma_\vp) + \kappa(\sigma_\vq) = k$. Therefore, we can express \cref{eq:combinatorial_sum_term} as: 
\begin{align}
    \sum_{\kappa(\sigma'_\vp) + \kappa(\sigma'_\vq) \leq k \leq \kappa(x_\vp) + \kappa(x_\vq) } \binom{ \kappa(x_\vp) + \kappa(x_\vq) - \kappa(\sigma'_\vp) - \kappa(\sigma'_\vq)   }{ k - \kappa(\sigma'_\vp) - \kappa(\sigma'_\vq) } (-1)^{ k - \kappa(\sigma'_\vp) - \kappa(\sigma'_\vq) } \,. 
\end{align}
We can shift the indices of this sum by $\kappa(\sigma'_\vp) + \kappa(\sigma'_\vq)$:
\begin{align}
    \sum_{ 0 \leq k \leq \kappa(x_\vp) + \kappa(x_\vq) - \kappa(\sigma'_\vp) - \kappa(\sigma'_\vq) } \binom{ \kappa(x_\vp) + \kappa(x_\vq) - \kappa(\sigma'_\vp) - \kappa(\sigma'_\vq)  }{k } (-1)^{ k } \,.
\end{align}
Next, we multiply this term by $1^{\kappa(x_\vp) + \kappa(x_\vq) - \kappa(\sigma'_\vp) - \kappa(\sigma'_\vq) - k } \equiv 1$ and obtain: 
\begin{align}
    \sum_{ 0 \leq k \leq \kappa(x_\vp) + \kappa(x_\vq) - \kappa(\sigma'_\vp) - \kappa(\sigma'_\vq) } \binom{ \kappa(x_\vp) + \kappa(x_\vq) - \kappa(\sigma'_\vp) - \kappa(\sigma'_\vq) }{ k } (-1)^{ k } 1^{ \kappa(x_\vp) + \kappa(x_\vq) - \kappa(\sigma'_\vp) - \kappa(\sigma'_\vq) - k } \,.
\end{align}
By the binomial theorem, this is equivalent to: 
\begin{align}
    (-1 + 1)^{\kappa(x_\vp) + \kappa(x_\vq) - \kappa(\sigma'_\vp) - \kappa(\sigma'_\vq)} \,.
\end{align}
If $\sigma'_\vp = x_\vp$ and $\sigma'_\vq = x_\vq$, this expression is $1$, and $0$ otherwise. Therefore, we can evaluate the last expression in \cref{eq:higher_order_binary_polynomial} to be equal to $f_{\vp,\vq}(x_\vp,x_\vq)$, as needed. This completes the proof. 
Therefore, if we could somehow transform the minimization of 
\begin{align}
    E(\ell_{(\cdot)}) = \sum_{(\vp,\vq) \in \mathcal{E}}
    \sum_{(\sigma_\vp,\sigma_\vq) \in \mathcal{L}_\vp \times \mathcal{L}_\vq} a_{\sigma_\vp,\sigma_\vq} (\Pi_{i \in [1, ... , n]} \delta (\sigma_\vp,x_{\vp,i})) \cdot (\Pi_{j \in [1, ... , m]}\delta (\sigma_\vq,x_{\vq,j})), 
\end{align}
into the minimization of a quadratic polynomial, we will have formed a QUBO problem. 

\subsection{Transforming Higher-Order Binary Vector Polynomial Minimization into a QUBO}
A technique to transform higher-order polynomial minimization over a binary vector into a QUBO 
exists and is well explained in Ishikawa \cite{5444874}: In Sec.~4.2, it is shown that, in a polynomial minimization problem in which all variables are binary, a polynomial term 
\begin{equation}
    a\vx_0...\vx_k
\end{equation}
can be transformed into 
\begin{equation}
    \text{min}_{w \in \{0,1\}} a w \{ S_1 - (k-1) \}, 
\end{equation} 
when $a < 0$ and 
\begin{equation}
    \text{min}_{w_0,...w_{\lfloor \frac{k-1}{2}\rfloor} \in \{0,1\}} a \{ \sum_{i=1}^k w_i(c_{i,k} (-S_1 + 2i)-1) + a S_2 \},
\end{equation}
when $a > 0$, and the minimal argument of the polynomial remains the same. Here, $c_{i,k} = 1$ if $k$ is odd and $i=k$, and $c_{i,k} = 2$ otherwise. $S_1$ and $S_2$ are defined as:
\begin{equation}
    S_1 = \sum_{i=1}^k \vx_i \,\,\mathrm{and}
\end{equation}
\begin{equation}
    S_2 = \frac{S_1(S_1-1)}{2} \,.
\end{equation}
This construction introduces auxiliary binary variables ($w$ if $a < 0$ or $w_1,...,w_k$ if $a > 0$) to handle the complexity of higher-order terms. These auxiliary binary variables are added into our QUBO problem, and must be optimized alongside our original binary variables. However, once the optimization is complete, we can read off our solution from the original variables and discard the response of the auxiliary variables. 

With these techniques, minimization of a polynomial of binary variables of any order can be reduced to a minimization of a quadratic polynomial of binary variables by iteratively applying the transformations explained above to any terms of order greater than $2$. A full proof of why these transformations preserve the minimal argument of the polynomial is too long to explain here, but is elaborated on at length in Ishikawa \cite{5444874}. 

We have shown how to express the minimization of $E(\ell_{(\cdot)})$ as a minimization over binary variables. A sketch of the full encoding algorithm goes as follows: 1) For each edge $(\vp,\vq)$, calculate all $a_{\vp,\vq}$ from \cref{eq:binary_encoding_coefficient_formula}; 2) sum all $f_{\vp, \vq}$ into one large polynomial $E(\ell_{(\cdot)})$ (See \cref{eq:label_energy_full_sum}), and reduce all higher-order terms to quadratic or lower using the techniques in Ishikawa \cite{5444874}; 3) build $Q$ from the resulting coefficients.
