# Supplementary material for: Quantum-Hybrid Stereo Matching With Nonlinear Regularization and Spatial Pyramids
Source: arXiv:2312.16118 source file (2024-12-06)
Supplement: Supplementary file 6 [file coarse_to_fine_ablation.tex]

\section{Ablation Study on the Coarse-to-Fine Levels}\label{sec:coarse_to_fine_ablation}
We investigated how well our method works if we have fewer coarse-to-fine levels. In the following experiment, we removed the iteration which considers stereo matching at a downsampling factor of $2$ (step $2$). The modified algorithm can still estimate all disparities (rounded to the nearest integer) present in the ground truth, provided that it makes the correct estimation at each step.  The visual results as shown in \cref{fig:ablation_ctof} and numerical results are shown in \cref{tab:ctof_ablation}. 
Other than the Sawtooth image pair, we see a decline visually and numerically in our estimates. We conclude that having intermediate resolution steps is useful to our method. They give the algorithm more opportunities to adjust as higher resolution details are shown, correcting previous inaccuracies. We also suspect that the inaccurate estimates for Sawtooth begin in the second iteration because its omission leads to better numerical results, and the improvement is particularly noticeable in the troublesome lower left area. 
\begin{table}[]
    \centering
    \begin{tabular}{|c| c | c || c | c |}
        \hline
        \multirow{2}{*}{\textbf{Image Pair}} &  \multicolumn{2}{ c ||}{\textbf{AS}} & \multicolumn{2}{ c |}{\textbf{NS2}}  \\ \cline{2-5} 
            & RMSE & BPP & RMSE & BPP  \\
            \hline
        \textbf{Tsukuba} & 1.53 & 12.93 & 1.60 & 13.97 \\ \hline
        \textbf{Bull}    & 0.58 & 3.46 & 0.82 & 10.15    \\ \hline
        \textbf{Sawtooth} & 1.89 & 24.51 & 1.71 & 18.06  \\ \hline
        \textbf{Venus}   & 0.96 & 8.16 & 1.15 & 13.62  \\ \hline
        \textbf{Average} & \textbf{1.24} & \textbf{12.27} & 1.32 & 13.95  \\ \hline
        \end{tabular}
    \caption{The Root Mean Squared Error (RMSE) and Bad Pixel Percentage (BPP) of our full method with \textbf{A}ll \textbf{S}teps, and  our method when the iteration step at the intermediate resolution is removed (\textbf{N}o \textbf{S}tep \textbf{2}). The Gurobi optimizer is used in both cases. The full algorithm has lower RMSE an BPP. }
    \label{tab:ctof_ablation}
\end{table}

\begin{figure}
    \centering
    \setlength\tabcolsep{1.5pt}
    \begin{tabular}{c c c c c}
                   & Tsukuba & Bull & Sawtooth & Venus \\
       \rotatebox{90}{\textcolor{white}{------------}\textbf{GT}} & \includegraphics[width=\tableimagewidth, height=\tableimageheight]{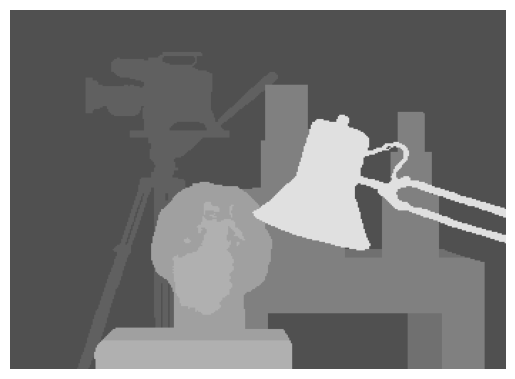} & \includegraphics[width=\tableimagewidth, height=\tableimageheight]{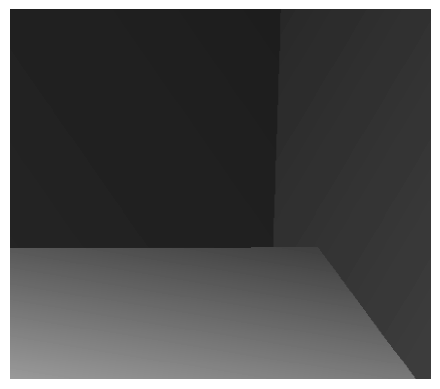}  & \includegraphics[width=\tableimagewidth, height=\tableimageheight]{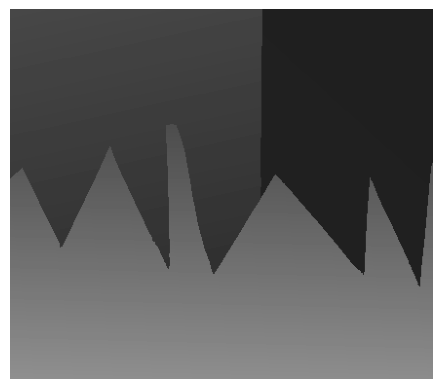} & \includegraphics[width=\tableimagewidth, height=\tableimageheight]{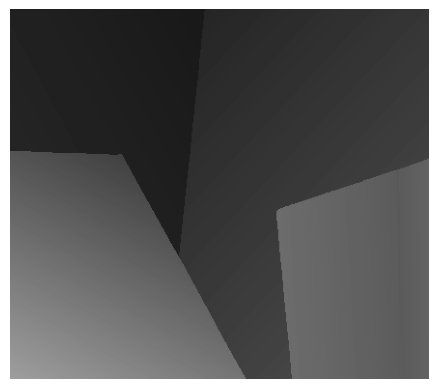}\\
       \rotatebox{90}{\textcolor{white}{-----------}\textbf{AS}} & \includegraphics[width=\tableimagewidth, height=\tableimageheight]{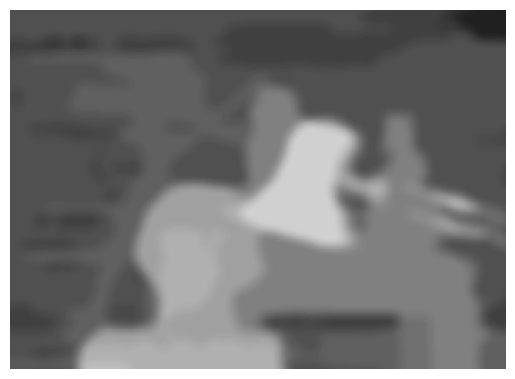} & \includegraphics[width=\tableimagewidth, height=\tableimageheight]{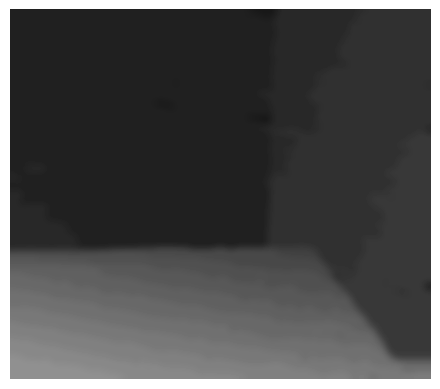}  & \includegraphics[width=\tableimagewidth, height=\tableimageheight]{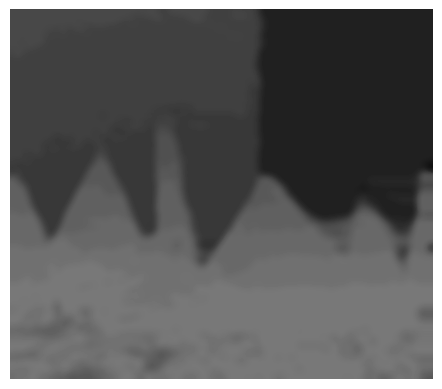} & \includegraphics[width=\tableimagewidth, height=\tableimageheight]{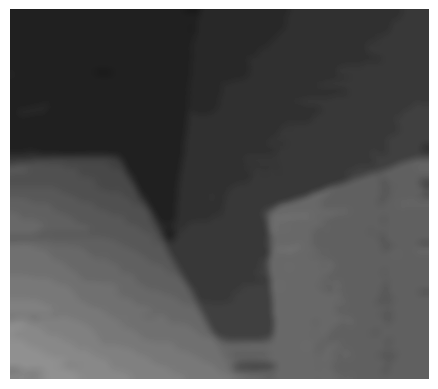}\\
       \rotatebox{90}{\textcolor{white}{------------}\textbf{NS2}} & \includegraphics[width=\tableimagewidth, height=\tableimageheight]{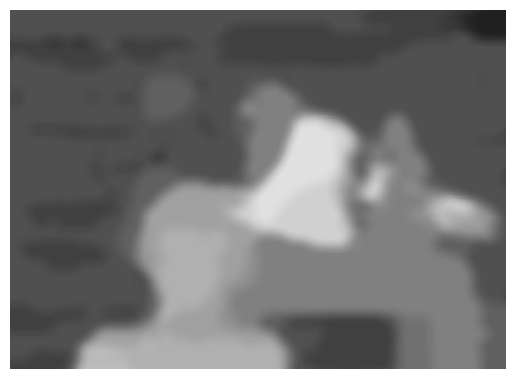} & \includegraphics[width=\tableimagewidth, height=\tableimageheight]{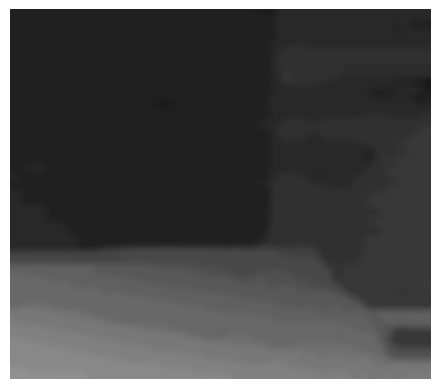}  & \includegraphics[width=\tableimagewidth, height=\tableimageheight]{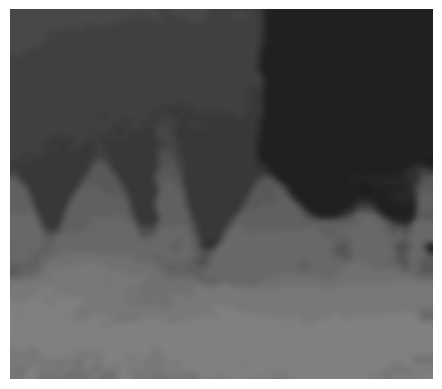} & \includegraphics[width=\tableimagewidth, height=\tableimageheight]{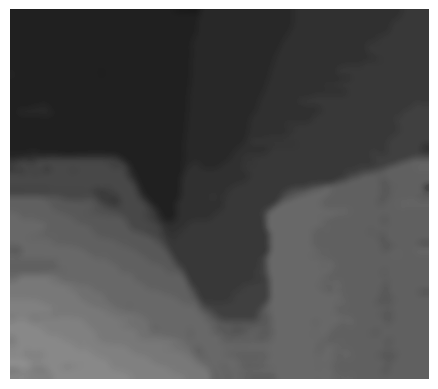}\\

    \end{tabular}
    \caption{By row: \textbf{G}round-\textbf{T}ruth displacements for each pair, our full method with \textbf{A}ll \textbf{S}teps, and  our method when the iteration step at the intermediate resolution is removed (\textbf{N}o \textbf{S}tep \textbf{2}). We can see that removing the second step means that some details are inaccurately estimated, such as a portion of the lamp in Tsukuba and planar regions in Venus. However, in the case of Sawtooth this lack of iterations and attention to details works to the algorithm's benefit. } 
    \label{fig:ablation_ctof}
\end{figure}
