# Supplementary material for: Quantum-Hybrid Stereo Matching With Nonlinear Regularization and Spatial Pyramids
Source: arXiv:2312.16118 source file (2024-12-06)
Supplement: Supplementary file 7 [file deriving_rectifiers.tex]

\section{Deriving Rectifiers For the One-Hot Encoding Scheme}\label{sec:deriving_rectifiers}
\subsection{Deriving Upper Bounds on Non-Granular Rectifiers}
We will now derive the function $\Lambda(\lab{\vv}^r,\lab{\vv}^s)$, which produces sufficiently high rectifier terms in \cref{eq:quadratic_form_equals_markov_energy_with_granular_constraints} such that the QUBO minimizer is the MRF MAP inference. In this section, we define this function such that the constraints are of the form used in QSync \cite{birdal2021quantum}. In \cref{subsec:granular_constraint_implementation}, we derive the more granular function. To define $\Lambda(\lab{\vv}^r,\lab{\vv}^s)$, we require some additional notation. Suppose $(\vp,\vq) \in \mathcal{E}$. Let 
\begin{equation} \label{eq:gamma_def}
    \gamma(\lab{\vp}^r,\vq) :=  \text{max}_{\lab{\vq}^s \in \mathcal{L}_\vq} \{ \varphi_{\vp,\vq}(\lab{\vp}^r,\lab{\vq}^s) \}\,.
\end{equation}
Thus, $\gamma(\lab{\vp}^r,\vq)$ represents the maximum regularization cost present on the edge $(\vp,\vq)$, if $\vp$ has been assigned the label $\lab{\vp}^r$. Next, we define: 
\begin{equation} \label{eq:chi_def}
            \chi(\vp) := \text{max}\{0, \text{min}_{\lab{\vp}^r \in \mathcal{L}_\vp} \{ \varphi_\vp(\lab{\vp}^r) + \sum_{(\vp,\vq) \in \mathcal{E}} \text{max}\{0, \gamma(\lab{\vp}^r,\vq) \} \} + \epsilon \}\,.\\
\end{equation}
$\chi(\vp)$ is an upper bound of the energy increase of flipping a label $\vx_{\lab{\vp}^r}$ of $\vp$ to be $1$. This energy increase is calculated from the data cost of flipping each label, added to the potential highest possible regularization costs of flipping that label. If all labels for $\vp$ are set to $0$, one can always pick a label to flip such that that energy increase is less than or equal to $\chi(\vp)$. 
We now define 
\begin{equation} \label{zeta_def}
    \zeta(\lab{\vp}^r) := \sum_{(\vp,\vq) \in \mathcal{E}} \sum_{\lab{\vq}^s \in \mathcal{L}_\vq} \text{min}\{0,  \varphi_{\vp,\vq}(\lab{\vp}^r, \lab{\vq}^s) \}\}\,.
\end{equation}
This value tracks all negative regularization energy that can be incurred by flipping $\vx_{\lab{\vp}^r}$ of $\vp$ to be $1$. 
Next, define 
\begin{equation}
    \Theta(\lab{\vp}^r,\lab{\vp}^s) := \text{min} \{0, \varphi_\vp(\lab{\vp}^r) + \zeta(\lab{\vp}^r) - \epsilon, \varphi_\vq(\lab{\vq}^s) + \zeta(\lab{\vq}^s) - \epsilon \} \,. 
\end{equation}
This value accounts for the smaller energy decrease of either flipping $\lab{\vp}^r$ or $\lab{\vp}^s$ to $1$.
Now, for any two labels $\lab{\vp}^i, \lab{\vp}^j \in \mathcal{L}_\vp$, we can define our function $\Lambda(\lab{\vp}^i, \lab{\vp}^j)$ as follows: 
\begin{equation}
    \Lambda(\lab{\vp}^i, \lab{\vp}^j) :=  \text{max} \{ \chi(\vp), \text{max}_{\lab{\vp}^r, \lab{\vp}^s \in \mathcal{L}_\vp} \{-\Theta(\lab{\vp}^r, \lab{\vp}^s)\} \}\,.
\end{equation}
We will now show that the lowest energy solution to the QUBO with the matrix presented in \cref{eq:quadratic_form_equals_markov_energy_with_granular_constraints} must satisfy the constraints presented in \cref{eq:onehot_qubo_constraints}.
\subsection{Every Variable Receives at Least One Label} \label{subsubsec:atleast}
This bound ensures that \textit{at least} one binary label $\vx_{\lab{\vp}^r}$ is $1$ for every variable $\vp$. Assume that all other labels $\vx_{\lab{\vp}^s}$ of $\vp$ are set to $0$. We select a label to flip $\lab{\vp}^r$ such that: 
\begin{align}
    \lab{\vp}^r = \text{argmin}_{\lab{\vp}^r \in \mathcal{L}_\vp} \{ \varphi_\vp(\lab{\vp}^r) + \sum_{(\vp,\vq) \in \mathcal{E}} \text{max}\{0, \gamma(\lab{\vp}^r,\vq) \} \} \,. 
\end{align}
Let $c$ be the regularization cost incurred by flipping $\lab{\vp}^r$ to $1$. Then, the total change in energy caused by flipping $\lab{\vp}^r$ is 
\begin{equation} \label{WorstCaseFlipScenario}
% \small
    \begin{split}
        & \varphi_\vp(\lab{\vp}^r) + c - \Lambda(\lab{\vp}^r,\lab{\vp}^r) \leq \\ 
        & \varphi_\vp(\lab{\vp}^r) + c - \chi(\vp) \leq \\
        & \varphi_\vp(\lab{\vp}^r) + c -\text{min}_{\lab{\vp}^r \in \mathcal{L}_\vp} \{ \varphi_\vp(\lab{\vp}^r) + \sum_{(\vp,\vq) \in \mathcal{E}} \text{max}\{0, \gamma(\lab{\vp}^r,\vq) \} \} - \epsilon \,. 
    \end{split}
\end{equation}
By our construction,
\begin{equation}
    c \leq \sum_{(\vp,\vq) \in \mathcal{E}} \text{max}\{0, \gamma(\lab{\vp}^r,\vq) \},
\end{equation}
which means
\begin{equation}
% \small
    \begin{split}
        \varphi_\vp(\lab{\vp}^r) + c \leq \text{min}_{\lab{\vp}^r \in \mathcal{L}_\vp} \{ \varphi_\vp(\lab{\vp}^r) + \sum_{(\vp,\vq) \in \mathcal{E}} \text{max}\{0, \gamma(\lab{\vp}^r,\vq) \} \} \,. \\
    \end{split}
\end{equation}
Therefore, the expression \eqref{WorstCaseFlipScenario} must be less than or equal to $-\epsilon < 0$. Thus, there is still a lower energy to set $\vx_{\lab{\vp}^r} = 1$ rather than $0$.
\subsection{Every Variable Receives at Most One Label} \label{subsubsec:atmost}
Conversely, this bound ensures that \textit{at most} one label $\vx_{\lab{\vp}^r}$ is set to $1$ for a variable $\vp$. Suppose $\vx_{\lab{\vp}^r}$ and $\vx_{\lab{\vp}^s}$ are two binary labels of the same variable. Assume without loss of generality that $\vx_{\lab{\vp}^r}=1$ and $\vx_{\lab{\vp}^s} = 0$. Now, consider the total change in energy that will occur if we flip $\vx_{\lab{\vp}^s}$ to $1$: there will be the cost incurred by the diagonal entry of $Q$ ($ \varphi_\vp(\lab{\vp}^s) - \Lambda(\lab{\vp}^s,\lab{\vp}^s)$), the cost of incurred by setting $\vx_{\lab{\vp}^r}$ and $\vx_{\lab{\vp}^s}$ to $1$  ($2 \Lambda(\lab{\vp}^s,\lab{\vp}^r)$), and some regularization cost from neighbor variables, which we will write as $c$. We sum all of these terms together to consider the total change in energy: 
\begin{align} \label{PrimitiveBoundAtMost}
\begin{split}
    & \varphi_\vp(\lab{\vp}^s) - \Lambda(\lab{\vp}^s,\lab{\vp}^s) + 2 \Lambda(\lab{\vp}^s,\lab{\vp}^r) + c = \\
    & \varphi_\vp(\lab{\vp}^s) + \Lambda(\lab{\vp}^s,\lab{\vp}^s) + c  \geq \\
    & \varphi_\vp(\lab{\vp}^s) + \text{max}_{\lab{\vp}^r, \lab{\vp}^s \in \mathcal{L}_\vp} \{-\Theta(\lab{\vp}^r, \lab{\vp}^s)\} + c \geq \\
    & \varphi_\vp(\lab{\vp}^s)  -\Theta(\lab{\vp}^r, \lab{\vp}^s) + c = \\
    & \varphi_\vp(\lab{\vp}^s)  -\text{min} \{0, \varphi_\vp(\lab{\vp}^r) + \zeta(\lab{\vp}^r) - \epsilon, \varphi_\vp(\lab{\vp}^s) + \zeta(\lab{\vp}^s) - \epsilon \} + c = \\
    & \varphi_\vp(\lab{\vp}^s) +  \text{max} \{0, -\varphi_\vp(\lab{\vp}^r) - \zeta(\lab{\vp}^r) + \epsilon, -\varphi_\vp(\lab{\vp}^s) -\zeta(\lab{\vp}^s) + \epsilon \} + c \geq \\
    & \varphi_\vp(\lab{\vp}^s) -\varphi_\vp(\lab{\vp}^s) -\zeta(\lab{\vp}^s) + \epsilon + c = \\
    & -\zeta(\lab{\vp}^s) + \epsilon + c \,.
\end{split}
\end{align}
By the construction of $\zeta(\lab{\vp}^s)$ in \cref{zeta_def}, $\zeta(\lab{\vp}^s)$ must be less than or equal to $c$. Thus, our expression above is greater than or equal to $\epsilon > 0$. Thus, there is a net increase in energy when we set both labels to $1$.  

\subsection{Proof of Correct QUBO Behaviour} \label{subsubsec:CorrectBehaviour}
We can guarantee that the lowest energy state satisfies our constraints. To understand this, consider a QUBO solution $\vx$ where, for some Markov variable $\vp$, all binary variables $\vx_{\lab{\vp}^i}$ are $0$. Then \cref{subsubsec:atleast} proves that there is a label that can be flipped to $1$ to lower the energy. Therefore, $\vx$ must not be the optimal solution. Now, consider a solution $\vx$ where $2$ or more binary variables that act as labels for Markov variable $\vp$ are set to $1$. \ref{subsubsec:atmost} shows that there will be a net energy decrease if one of those variables is flipped to $0$. Therefore, $\vx$ cannot be the optimal solution. Therefore, the optimal QUBO solution must obey the constraints in \cref{eq:onehot_qubo_constraints}. 

Let $\vx$ be a QUBO solution which obeys all constraints, and corresponds to a labelling $\ell$. The total energy of the QUBO is: 
\begin{equation} 
    \vx^TQ\vx = E(\ell) - \sum_{\vp \in \mathcal{V}} \Lambda(\lab{\vp}^i,\lab{\vp}^i) \,,
    \label{EnergyOfConstrainedSolution}
\end{equation}
with $E(\ell)$ as defined in \cref{eq:markov_cost_quadratic_form}. Because $\sum_{\vp \in \mathcal{V}} \Lambda(\lab{\vp}^i,\lab{\vp}^i)$ is a constant, it is clear that any solution $\vx^*$ which minimizes $\vx^TQ\vx$ must therefore minimize $E(\ell_{(.)})$. 
\subsection{A More Granular Implementation of Constraints}\label{subsec:granular_constraint_implementation}
We can treat $\Lambda$ is a function of individual labels:
\begin{equation}
    \Lambda(\lab{\vp}^r,\lab{\vp}^s) = 
    \begin{cases}
        \chi(\vp) & \text{ if } r = s \\
        \frac{\chi(\vp) -\Theta(\lab{\vp}^r, \lab{\vp}^s)}{2} & \text{ else } \,.\\
    \end{cases}  \\
\end{equation}
We prove that the resulting QUBO obeys our constraints at its optimum, and then the rest of the proof follows exactly the derivations in \cref{subsubsec:CorrectBehaviour}.

To prove that every variable receives at least one label, the same argument given in \cref{subsubsec:atleast} holds in this case as well. We can show that for every $\vp$, there exists a label $\lab{\vp}^r$ such that flipping it to $1$ will cause an energy change of $\varphi_\vp(\lab{\vp}^r) + c - \chi(\vp) < 0$ if no other label has been flipped yet.

To prove that every variable receives at most one label, the argument given in \cref{subsubsec:atmost} needs to be modified slightly. In this case, the net change in energy from flipping $\vx_{\lab{\vp}^2}$ to $1$ is:
\begin{align}
    \begin{split}
        &\varphi_\vp(\lab{\vp}^s) - \chi(\vp) + 2 \frac{\chi(\vp) -\Theta(\lab{\vp}^r,\lab{\vp}^s)}{2} + c = \\
        &\varphi_\vp(\lab{\vp}^s) - \Theta(\lab{\vp}^r,\lab{\vp}^s) + c \,.\\
    \end{split}
\end{align}
From here, the proof follows the same logic as in \cref{PrimitiveBoundAtMost}. 

\subsection{Analysis of Improvement}
The decrease in $\Lambda(\lab{\vp}^r, \lab{\vp}^s)$ for  $r=s$ is: 
\begin{equation}
    \text{max} \{0 , \text{max}_{\lab{\vp}^r, \lab{\vp}^s \in \mathcal{L}_\vp} \{-\Theta(\lab{\vp}^r, \lab{\vp}^s)\} - \chi(\vp) \} \,.
\end{equation}
The decrease in $\Lambda(\lab{\vp}^r, \lab{\vp}^s)$ for  $r \neq s$ is:
\begin{equation}
        \text{max} \bigg\{ \frac{\chi(\vp) + \Theta(\lab{\vp}^r, \lab{\vp}^s)}{2} ,  \text{max}_{\lab{\vp}^r, \lab{\vp}^s \in \mathcal{L}_\vp} \{-\Theta(\lab{\vp}^r, \lab{\vp}^s)\} - \frac{\chi(\vp) -\Theta(\lab{\vp}^r, \lab{\vp}^s)}{2} \bigg\} \,.
\end{equation}
By implementing more granular constraints, we can be less disruptive to the energy landscape with the same constraint guarantees. Thus, this formulation is an improvement upon the less granular formulation presented in \cite{birdal2021quantum}
