# Supplementary material for: Quantum-Hybrid Stereo Matching With Nonlinear Regularization and Spatial Pyramids
Source: arXiv:2312.16118 source file (2024-12-06)
Supplement: Supplementary file 8 [file embedding_qubo_problems.tex]

\section{Embedding QUBO Problem Graphs onto D-Wave}\label{sec:embedding_problem_graphs}
One key bottleneck for modern quantum computing is minor embedding: once a QUBO is defined, all the binary variables of $\vx$ must be mapped to physical qubits present on the QPU, and all non-zero entries of the off-diagonals of $Q$ must be mapped to the appropriate physical couplers connecting physical qubits. To make this embedding process more flexible, it is possible to chain qubits together: any two physical qubits which share a coupler can be treated as a single physical qubit during the embedding. However, during annealing, qubit chains are at risk of breaking (\textit{i.e.,} not behaving like a single physical qubit), making it ill-defined to measure the QUBO solution from the annealer. The longer the qubit chain, the higher the risk of the chain breaking. Therefore, we aim to keep chains as small as possible.  

We first examine the embedding properties of our one-hot encoding scheme, and then turn our attention to the binary encoding scheme proposed in \cref{sec:binary_encoding_of_mrf_map}, and see why it is more challenging to embed.

\subsection{Embedding of the One-Hot Encoding Scheme}
A QUBO's \textit{problem graph} is a useful concept for discussing minor embedding. For a QUBO problem represented by the matrix $Q$, the corresponding problem graph has vertices corresponding to each binary variable of the QUBO, and edges connecting any two vertices whose corresponding binary variables interact in the QUBO problem. We visualize the QUBO problem graphs for the first epipolar line of the Venus image pair at all three coarse-to-fine steps in \cref{fig:qubo_problem_graphs}. We visualize those same problem graphs when they are embedded onto the D-Wave Pegasus hardware in \cref{fig:qubo_problem_embeddings}. The numerics for these problem graphs and embeddings are given in \cref{tab:dwave_embeddings_one_hot}.

For all steps, an embedding is possible, meaning our algorithm can be run on modern hardware. Additionally, the number of vertices of our QUBO problem graph grows linearly as the number of disparities considered by the algorithm increases, or when the length of the epipolar line increases. This means that the one-hot encoding scales well as our problem size increases.
\begin{figure}
    \centering
    \setlength\tabcolsep{1.5pt}
    \begin{tabular}{c c c}
                   \textbf{Step 1} & \textbf{Step 2} & \textbf{Step 3} \\
       \includegraphics[width=\embeddingtableimagewidth, height=\embeddingtableimageheight]{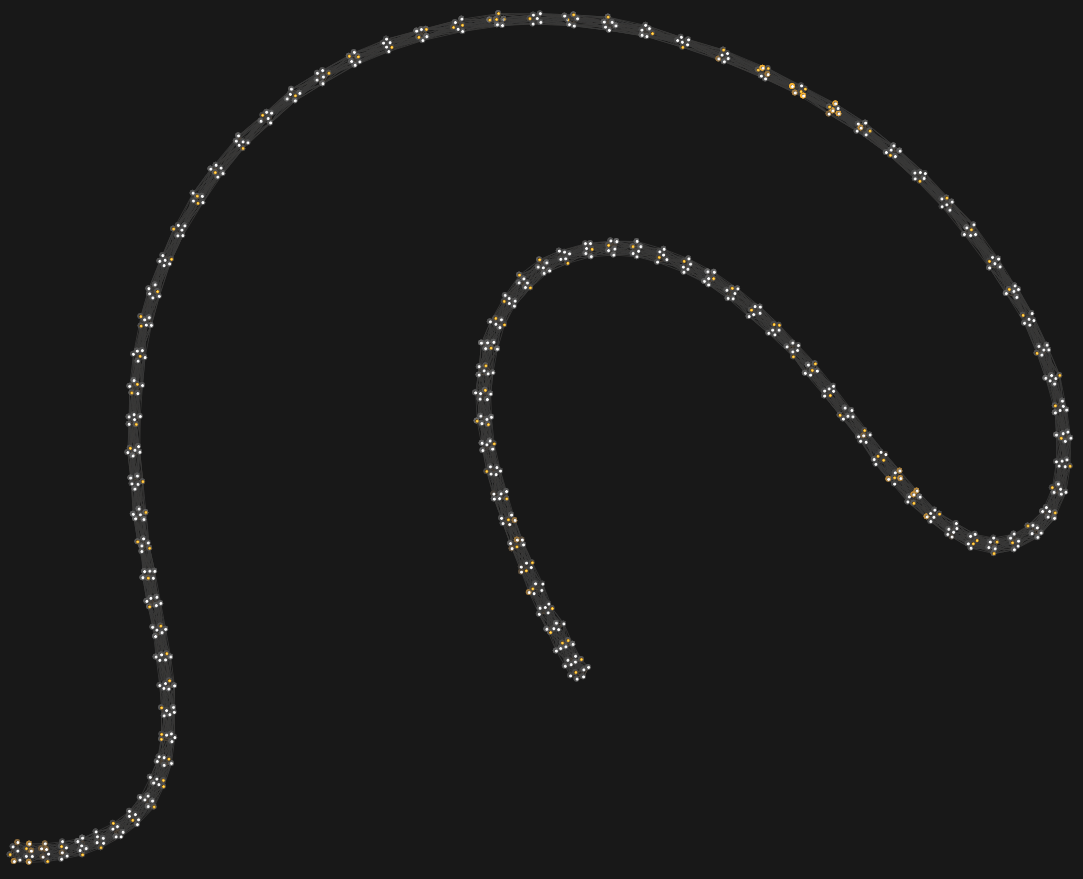} & \includegraphics[width=\embeddingtableimagewidth, height=\embeddingtableimageheight]{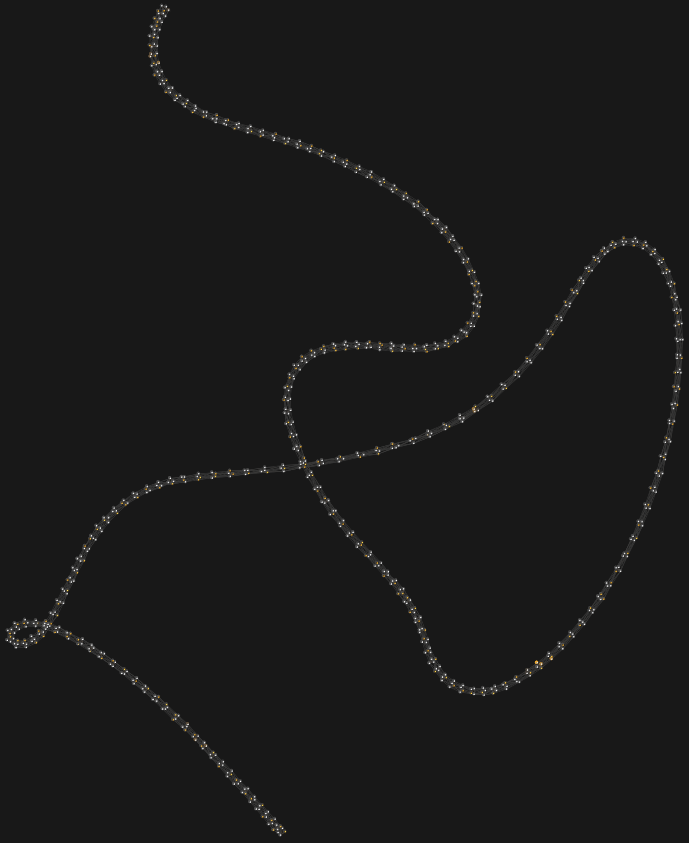}  & \includegraphics[width=\embeddingtableimagewidth, height=\embeddingtableimageheight]{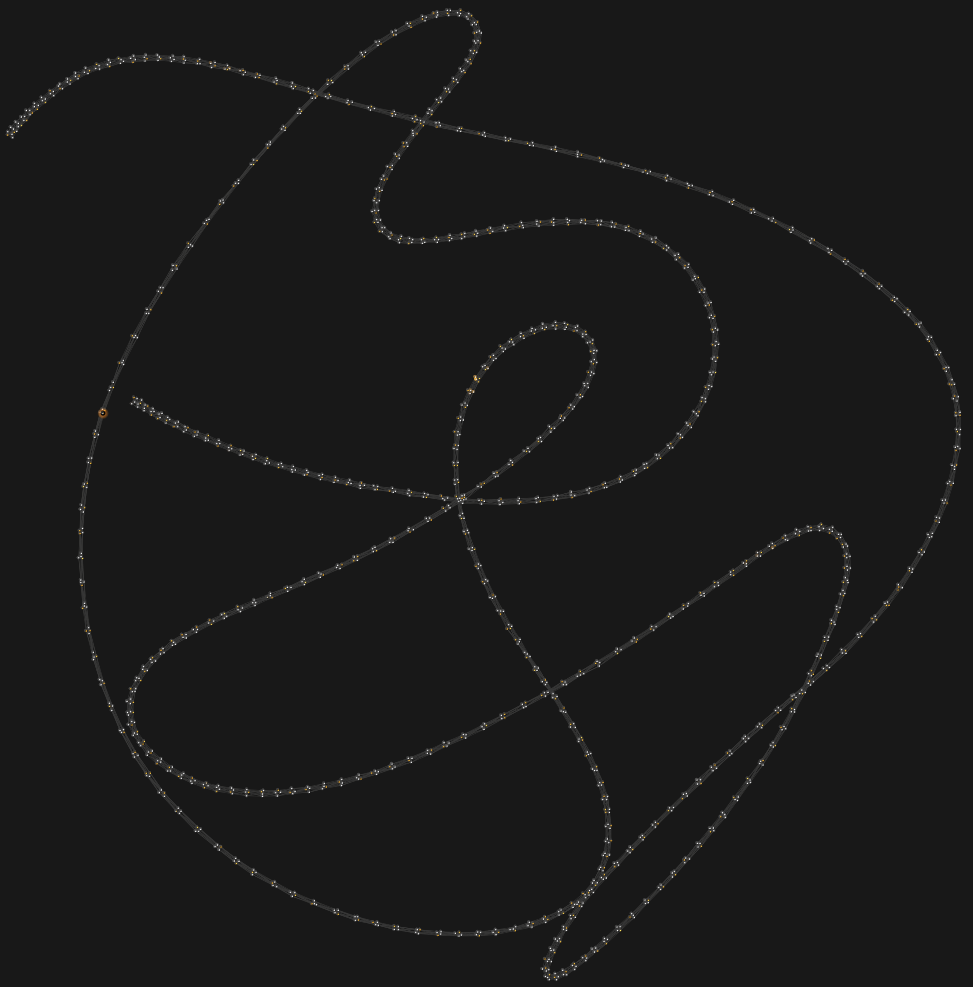} \\
    \end{tabular}
    \caption{The QUBO problem graphs for the first epipolar line of Venus image pair visualized using D-Wave's Problem Inspector. The single curve structure of these graphs arises because regularization costs only occur between the immediate neighbors on the epipolar line.} 
    \label{fig:qubo_problem_graphs}
\end{figure}
\begin{figure}
    \centering
    \setlength\tabcolsep{1.5pt}
    \begin{tabular}{c c c}
                   \textbf{Step 1} & \textbf{Step 2} & \textbf{Step 3} \\
       \includegraphics[width=\embeddingtableimagewidth, height=\embeddingtableimageheight]{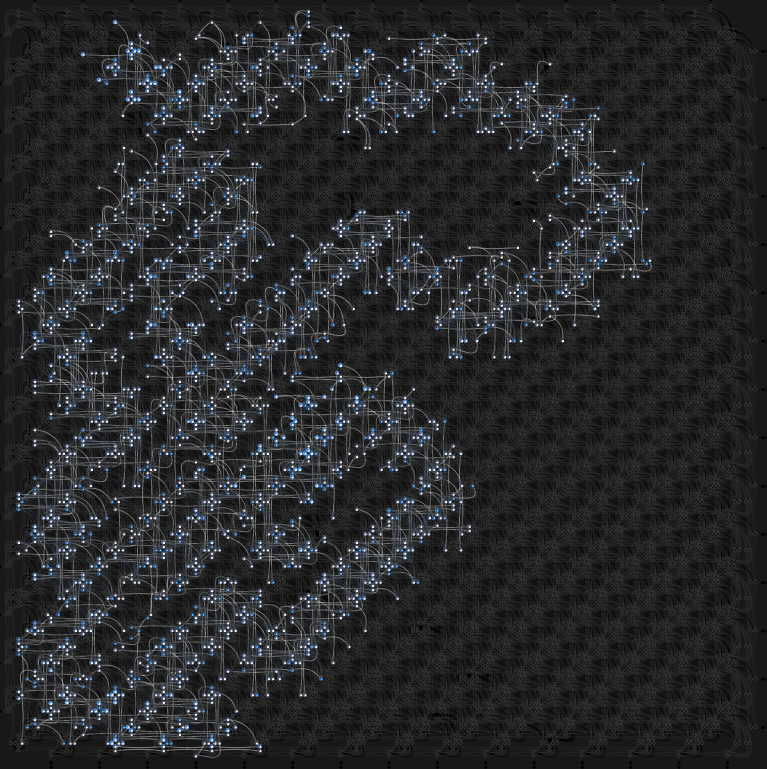} & \includegraphics[width=\embeddingtableimagewidth, height=\embeddingtableimageheight]{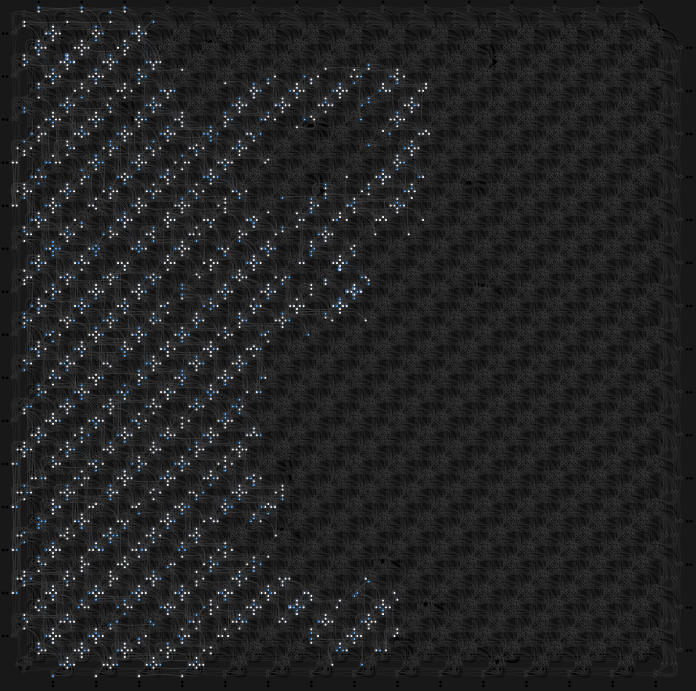}  & \includegraphics[width=\embeddingtableimagewidth, height=\embeddingtableimageheight]{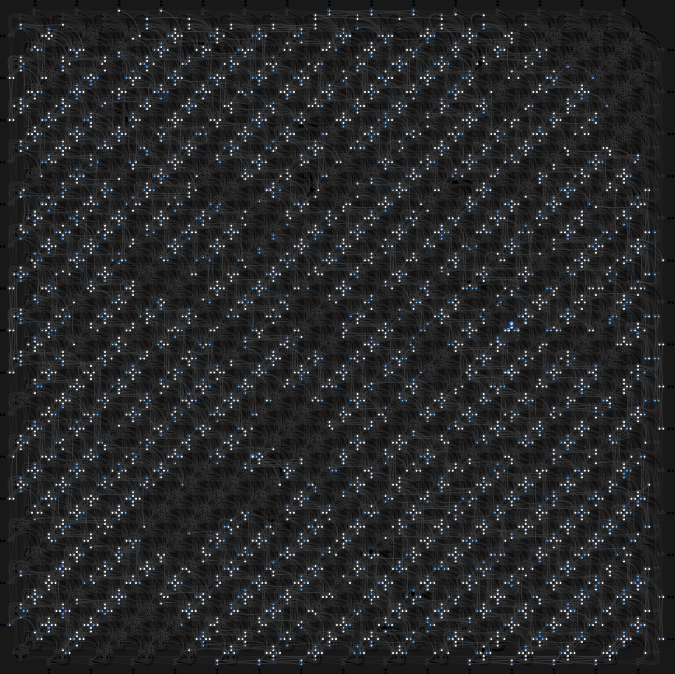} \\
    \end{tabular} 
    \caption{The QUBO problem embeddings onto D-Wave's Pegasus QPU for the first epipolar line of Venus image pair visualized using D-Wave's Problem Inspector. The Pegasus QPU has $5,640$ qubits with $40,484$ couplers \cite{2020arXiv200300133B}. Although the QUBO problem graphs have much fewer vertices and edges than the Pegasus QPU's qubits and couplers, one can see that a large portion of these resources are needed in order to embed properly. This is because many qubit chains are used for the embedding.} 
    \label{fig:qubo_problem_embeddings} 
\end{figure}

\begin{table}
    \centering
    \begin{tabular}{|c|c|c|c|}
        \hline
        \textbf{Step} & \textbf{1} & \textbf{2} & \textbf{3}  \\
        \hline
        \textbf{Epipolar Line Length} & 108 & 217 & 434 \\
        \hline
        \textbf{Disparity Levels} & 6 & 4 & 4 \\
        \hline
        \textbf{QUBO Graph Nodes} & 648 & 868 & 1,736 \\
        \hline
        \textbf{QUBO Graph Edges} & 5,472 & 4,758 & 9,532\\
        \hline
        \textbf{Physical Qubits} & 2,254 & 1,937 & 3,795\\
        \hline
        \textbf{Physical Couplers} & 6,541 & 5,827 & 11,591\\
        \hline
        \textbf{Physical Max Chain Length} & 10 & 5 & 5\\
        \hline
    \end{tabular}
  \caption{QUBO Problem graph statistics for our method with a one-hot encoding scheme for a single epipolar line, and statistics on the computed embeddings of the QUBO problem graphs onto the D-Wave Pegasus QPU. The epipolar line length is from the widest of the Middlebury images, Venus and Sawtooth. Thus, our stereo matching QUBO problems are embeddable on modern quantum hardware.}
  \label{tab:dwave_embeddings_one_hot}
\end{table}
\subsection{Embedding of the Binary Encoding Scheme}
We report the number of QUBO problem graph edges and vertices required for stereo matching the Venus image pair (across all steps) in \cref{tab:dwave_embeddings_binary_encoding}. For Step 1, the number of edges is greater than the number of couplers, meaning it is impossible to find an embedding.
As the number of disparities grows, the number of auxiliary binary variables needed grows exponentially (see Section 5.4 of Ishikawa \cite{5444874}). This explains why the problem graph for the initial step is so large. Note that the number of binary variables needed still grows linearly with respect to epipolar line length. 

D-Wave's upcoming QPU with the Zephyr topology (expected in 2024) should contain $7.4 \cdot 10^4$ qubits \cite{Zephyr2021}. However, we were still unable to find an embedding for Step 1 in this topology. Because we cannot embed this binary encoding approach into modern or next-generation QPU's, we decided to focus our attention on using the one-hot encoding scheme.
\begin{table}
    \centering
    \begin{tabular}{|c|c|c|c|}
        \hline
        \textbf{Step} & \textbf{1} & \textbf{2} & \textbf{3}  \\
        \hline
        \textbf{QUBO Graph Nodes} & 5,461 & 1,514 & 3,033 \\
        \hline
        \textbf{QUBO Graph Edges} & 147,452 & 7,561 & 15,156 \\
        \hline
    \end{tabular}
  \caption{Computed embeddings for the D-Wave Pegasus, binary encoding. Given the increased complexity of the graph topology, we were unable to calculate embeddings for all $3$ resolution levels. 
  } 
  \label{tab:dwave_embeddings_binary_encoding}
\end{table}
