# Supplementary material for: Quantum-Hybrid Stereo Matching With Nonlinear Regularization and Spatial Pyramids
Source: arXiv:2312.16118 source file (2024-12-06)
Supplement: Supplementary file 9 [file model_hyperparameters.tex]

\section{Model Hyperparameters} \label{sec:regularization_hyper_parameters}
We summarize our model parameters used across all three coarse-to-fine levels of our algorithm in \cref{tab:model_hyperparamters}. These parameters were found to optimize RMSE while keeping an acceptable BPP. The median filter is across an entire window -- and not a vertical median filter as in \cite{9653310} -- as we found this improved the estimation. We found that at the full resolution, a non-truncated regularizer worked best in general. Nevertheless, we still leverage the truncation at lower levels, so it is still present in our approach. Also, note that the range of $I^L, I^R$ is on the interval $[0,1]$. 
\begin{table}[]
    \centering
    \begin{tabular}{|c| c | c | c | }
        \hline
        \textbf{Step} & \textbf{1} & \textbf{2}  & \textbf{3}  \\ \hline
        Downsample Factor (\cref{alg:full_quantum_algorithm}) & 4 & 2 & 1  \\ \hline
        Displacements Considered (\cref{alg:full_quantum_algorithm})  & 6 & 4 & 4 \\ \hline
        $\tau$ (\cref{eq:edge_aware_potts_model}) & 0.15 & 0.15 & 0.3  \\ \hline
        q (\cref{eq:edge_aware_potts_model})  & 10 & 10 & 10 \\ \hline
        m (\cref{eq:truncated_linear_regularizer}) &  0.0015 & 0.0015 & $\infty$ \\ \hline
        s (\cref{eq:truncated_linear_regularizer}) & 0.0005 & 0.0003 & 0.0005\\ \hline
        Median Filter Window (\cref{alg:full_quantum_algorithm}) & 7$\times$7 & 7$\times$7& 7$\times$7 \\ \hline
        Bilateral Filter Diameter (\cref{alg:full_quantum_algorithm}) & \textbf{n/a} & \textbf{n/a} & 12 \\ \hline
        Bilateral Filter Sigma Color (\cref{alg:full_quantum_algorithm}) & \textbf{n/a} & \textbf{n/a} & 75 \\ \hline 
        Bilateral Filter Sigma Space (\cref{alg:full_quantum_algorithm}) & \textbf{n/a} & \textbf{n/a} & 75 \\ \hline 
        \end{tabular}   
    \caption{Hyperparameters for our stereo matching algorithm described in \cref{subsec:our_algorithm} of the main paper.} 
    \label{tab:model_hyperparamters}
\end{table}
