# Supplementary material for: Quantum-Hybrid Stereo Matching With Nonlinear Regularization and Spatial Pyramids
Source: arXiv:2312.16118 source file (2024-12-06)
Supplement: Supplementary file 10 [file rectifier_strength.tex]

\section{Ablation Study on the Strength of the Rectifiers}\label{sec:rectifier_strength}
As discussed in Birdal \etal \cite{birdal2021quantum}, larger constraint values can negatively affect annealer performance. Therefore, we wanted to see if we can improve performance by decreasing these constraint values. What this means in practice is that we modify our QUBO matrix given in \cref{eq:quadratic_form_equals_markov_energy_with_granular_constraints} to the following:
\begin{equation}
\begin{split}
    \forall \vv \in \mathcal{V},\, \forall \lab{\vv}^l \in \mathcal{L}_\vv: & \,\, Q_{\lab{\vv}^l,\lab{\vv}^l} = \varphi_\vv(\lab{\vv}^l)  - t \cdot \Lambda(\lab{\vv}^l,\lab{\vv}^l) \\
    \forall \vp \in \mathcal{V},\, \forall \lab{\vp}^r,\lab{\vp}^s \in \mathcal{L}_\vp,\, r \neq s: & \,\, Q_{\lab{\vp}^r,\lab{\vp}^s} = t \cdot \Lambda(\lab{\vp}^r,\lab{\vp}^s) \\
    & \,\, Q_{\ell_\vp^j,\ell_\vp^i} = t \cdot \Lambda(\lab{\vp}^r,\lab{\vp}^s) \\
    \forall (\vp,\vq) \in E, \forall \ell_\vp^i \in \mathcal{L}_\vp \forall \ell_\vq^j \in \mathcal{L}_\vq: & \,\, Q_{\ell_\vp^i, \ell_\vq^j} = \frac{1}{2}\varphi_{\vp,\vq}(\ell_\vp^i,\ell_\vq^j) \\ 
      & \,\, Q_{ \ell_\vq^j, \ell_\vp^i} = \frac{1}{2}\varphi_{\vp,\vq}(\ell_\vp^i,\ell_\vq^j). \\
\end{split}
\label{eq:quadratic_form_equals_markov_energy_with_variable_rectifiers}
\end{equation}
Here, $t \geq 0$ can adjust the strength of our rectifiers. Our formulation in \cref{eq:quadratic_form_equals_markov_energy_with_granular_constraints} is a specialized case of \cref{eq:quadratic_form_equals_markov_energy_with_variable_rectifiers} where $t = 1$. For this experiment, we ran our stereo matching algorithm on the four Middlebury image pairs using all the default settings as described in \cref{sec:regularization_hyper_parameters}, while changing this newly introduced variable $t$. We show the visual results in \cref{fig:ablation_rectifier_strength} and numerical results in \cref{tab:our_sa_vary_t}. Note that in the case that two or more disparities are chosen during annealing, the lower disparity is chosen. In the case that no disparity was selected, the lowest possible disparity was selected. These experiments ran on D-Wave's simulated annealer. 

By graphing the of the average RMSE and BPP of these stereo estimates over $t$ (as shown in \cref{fig:rectifier_strength_graph}), we observe that lowering $t$ actually improves our results, with an optimum around $t = 0.25$, even though for this value, our constraints have not been formally proven to be obeyed. We also observe that some $t > 0$ is necessary to avoid the simulator returning the trivial answer of $0$. Given more time, we would like to investigate this performance improvement further to optimize $t$, and conduct experiments on the actual QPU.

\begin{table}[]
    \centering
    \begin{adjustbox}{width=\columnwidth,center}
    \begin{tabular}{|c| c | c || c | c || c | c || c | c || c | c || c | c || c | c |}
        \hline
        \multirow{2}{*}{\textbf{Image Pair}} &  \multicolumn{2}{ c ||}{$t = 0$ (\textbf{SA}) } & \multicolumn{2}{ c ||}{$t = 0.25$ (\textbf{SA})} & \multicolumn{2}{ c ||}{$t = 0.5$ (\textbf{SA})} &  \multicolumn{2}{ c ||}{$t = 0.75$ (\textbf{SA})} &  \multicolumn{2}{ c ||}{$t = 1$ (\textbf{SA})} &  \multicolumn{2}{ c ||}{$t = 1.25$ (\textbf{SA})} &  \multicolumn{2}{ c |}{$t = 1.5$ (\textbf{SA})} \\ \cline{2-15}
            & RMSE & BPP & RMSE & BPP & RMSE & BPP & RMSE & BPP & RMSE & BPP & RMSE & BPP & RMSE & BPP \\
            \hline
        \textbf{Tsukuba}  & 7.29  & 100 & 1.87  & 26.24 & 1.80  & 23.70  & 1.79 & 24.37 & 1.87 & 30.64 & 1.84 & 27.11 & 1.89 & 30.06\\ \hline
        \textbf{Bull}     & 8.29  & 100 & 1.30  & 24.28 & 1.42  & 31.59  & 1.97 & 38.53 & 1.87 & 45.29 & 2.10 & 43.74 & 2.21 & 48.11 \\ \hline
        \textbf{Sawtooth} & 10.72 & 100 & 2.86  & 38.09 & 2.84  & 46.84  & 2.98 & 53.85 & 3.04 & 56.75 & 3.23 & 59.50 & 3.22 & 60.96 \\ \hline
        \textbf{Venus}    & 9.39  & 100 & 2.04  & 36.73 & 2.12  & 42.35  & 2.26 & 47.83 & 2.27 & 47.73 & 2.35 & 50.28 & 2.56 & 53.71 \\ \hline
        \textbf{Average}  & 8.92  & 100 & \textbf{2.02}  & \textbf{31.34} & 2.05  & 36.12  & 2.25 & 41.15 & 2.26 & 45.10 & 2.38 & 45.16 & 2.47 & 48.21\\ \hline
        \end{tabular}
    \end{adjustbox}
    
    \caption{The Root Mean Squared Error (RMSE) and Bad Pixel Percentage (BPP) of the \textbf{S}imulated \textbf{A}nnealing method for increasing values of $t$. Lowering $t$ below $1$ can improve our metrics. }
    \label{tab:our_sa_vary_t}
\end{table}
\begin{figure}
    \centering
    \includegraphics[width=\graphimagewidth, height=\graphimageheight]{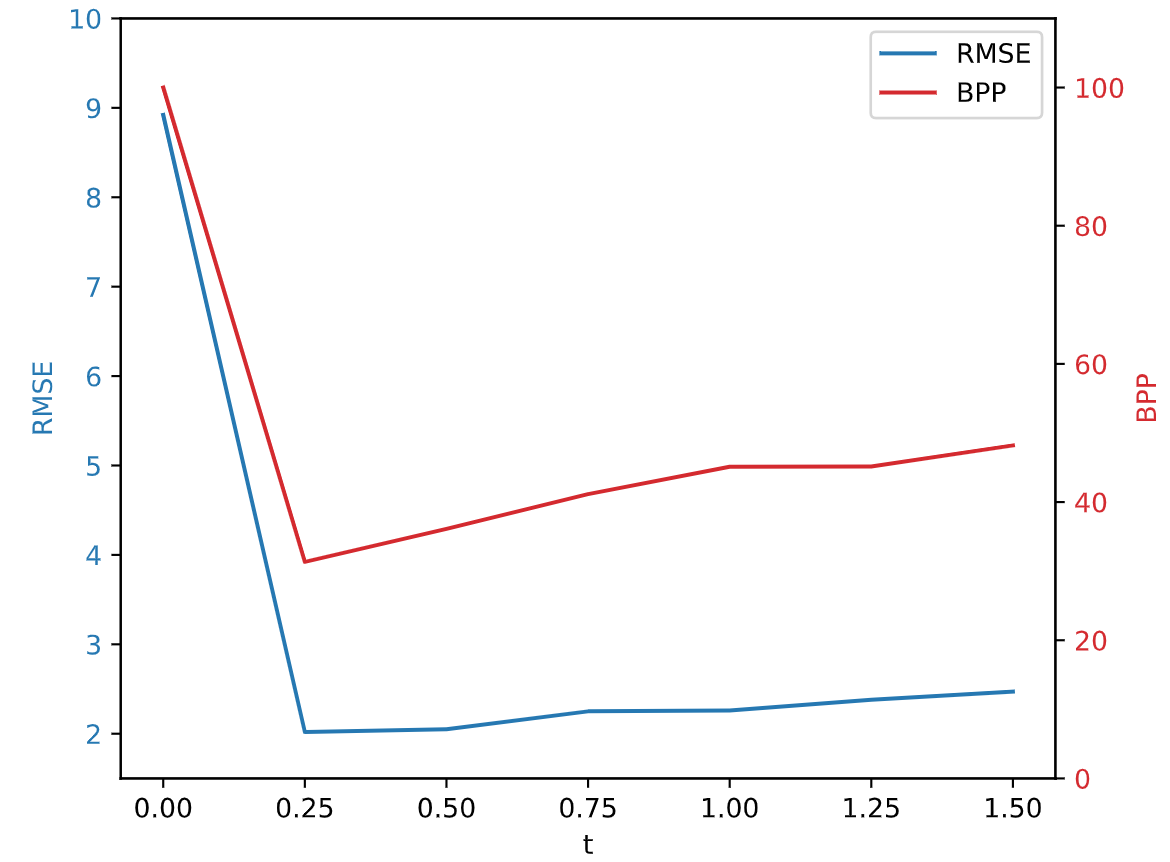}
    \caption{The average RMSE and BPP for the four Middlebury benchmarks over the rectifier strength $t$. We observe that both error metrics obtain a minimum around $t = 0.25$.} 
    \label{fig:rectifier_strength_graph}
\end{figure}

\begin{figure}
    \centering
    \setlength\tabcolsep{1.5pt}
    \begin{tabular}{c c c c c}
                   & Tsukuba & Bull & Sawtooth & Venus \\
       \rotatebox{90}{\textcolor{white}{-----.---}\textbf{GT}} & \includegraphics[width=\rectifiertableimagewidth, height=\rectifiertableimageheight]{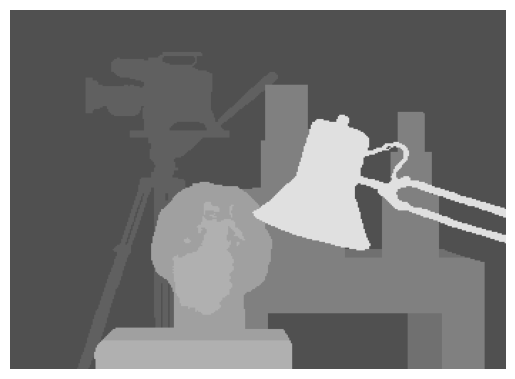} & \includegraphics[width=\rectifiertableimagewidth, height=\rectifiertableimageheight]{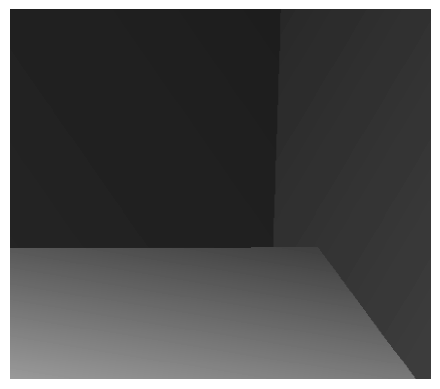}  & \includegraphics[width=\rectifiertableimagewidth, height=\rectifiertableimageheight]{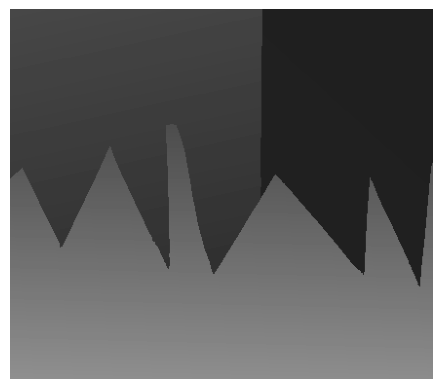} & \includegraphics[width=\rectifiertableimagewidth, height=\rectifiertableimageheight]{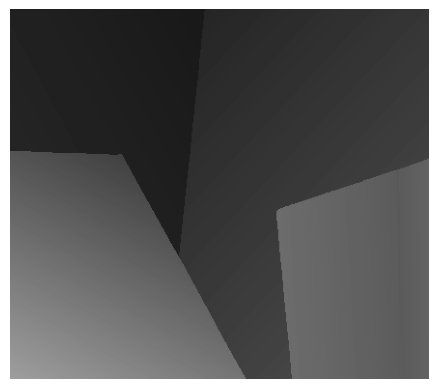}\\
       \rotatebox{90}{\textcolor{white}{----}$t = 0$ (\textbf{SA})} & \includegraphics[width=\rectifiertableimagewidth, height=\rectifiertableimageheight]{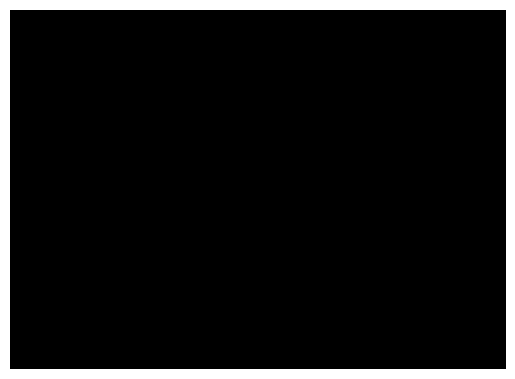} & \includegraphics[width=\rectifiertableimagewidth, height=\rectifiertableimageheight]{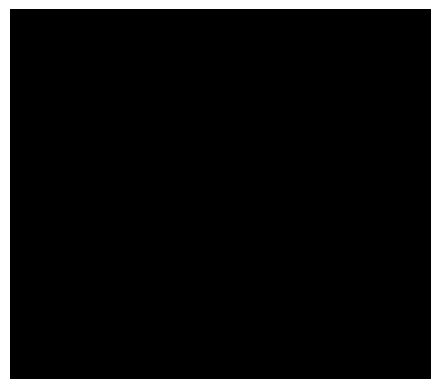}  & \includegraphics[width=\rectifiertableimagewidth, height=\rectifiertableimageheight]{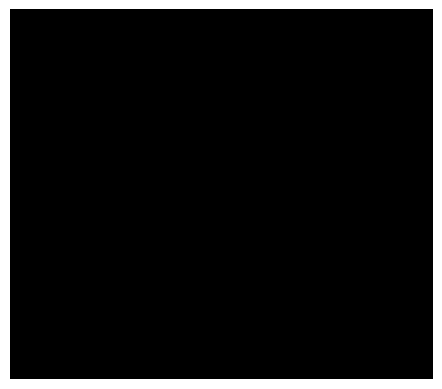} & \includegraphics[width=\rectifiertableimagewidth, height=\rectifiertableimageheight]{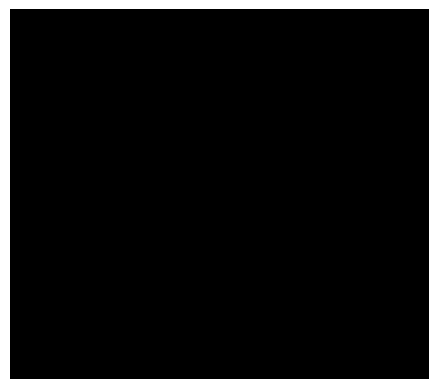}\\
       \rotatebox{90}{\textcolor{white}{--.}$t = 0.25$ (\textbf{SA})} & \includegraphics[width=\rectifiertableimagewidth, height=\rectifiertableimageheight]{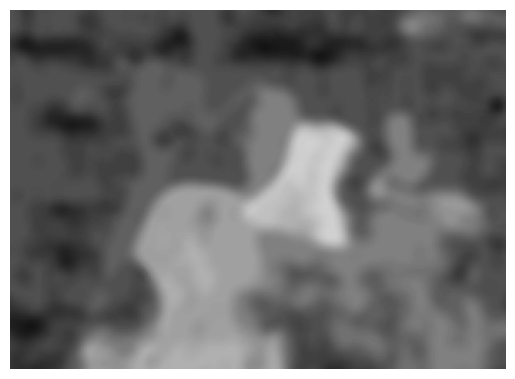} & \includegraphics[width=\rectifiertableimagewidth, height=\rectifiertableimageheight]{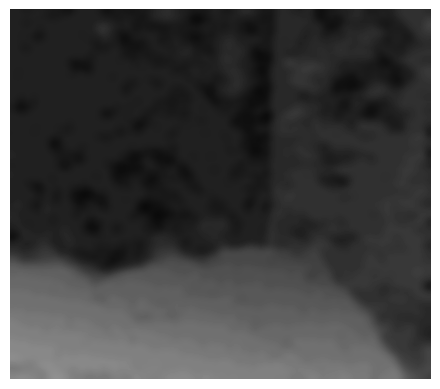}  & \includegraphics[width=\rectifiertableimagewidth, height=\rectifiertableimageheight]{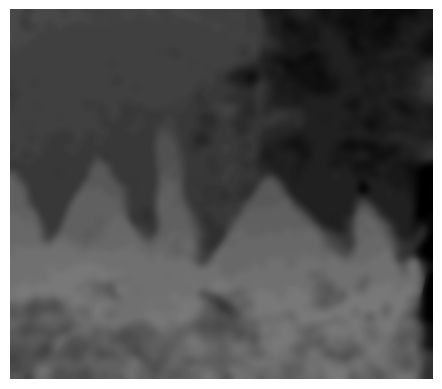} & \includegraphics[width=\rectifiertableimagewidth, height=\rectifiertableimageheight]{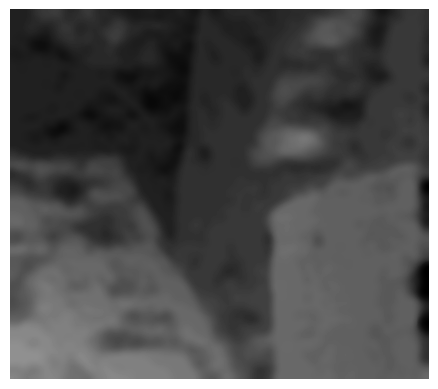}\\
       \rotatebox{90}{\textcolor{white}{---}$t = 0.5$ (\textbf{SA})} & \includegraphics[width=\rectifiertableimagewidth, height=\rectifiertableimageheight]{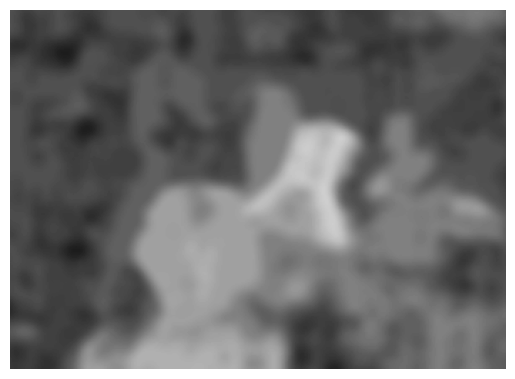} & \includegraphics[width=\rectifiertableimagewidth, height=\rectifiertableimageheight]{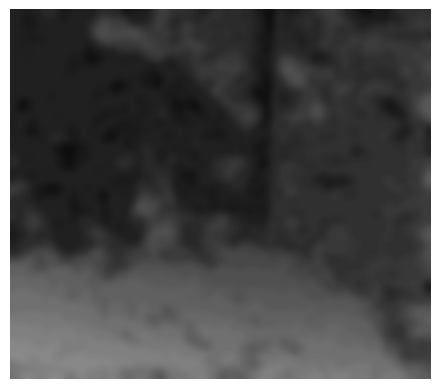}  & \includegraphics[width=\rectifiertableimagewidth, height=\rectifiertableimageheight]{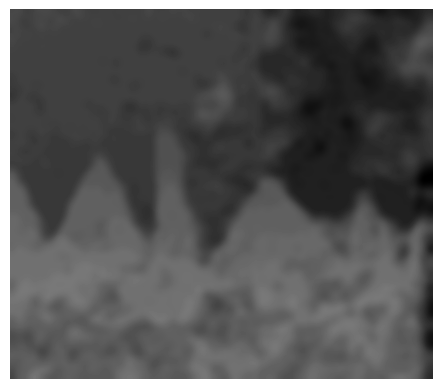} & \includegraphics[width=\rectifiertableimagewidth, height=\rectifiertableimageheight]{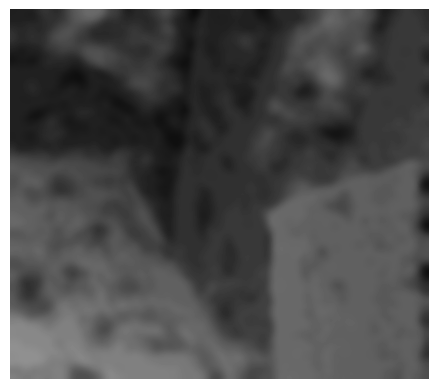}\\
       \rotatebox{90}{\textcolor{white}{--.}$t = 0.75$ (\textbf{SA})} & \includegraphics[width=\rectifiertableimagewidth, height=\rectifiertableimageheight]{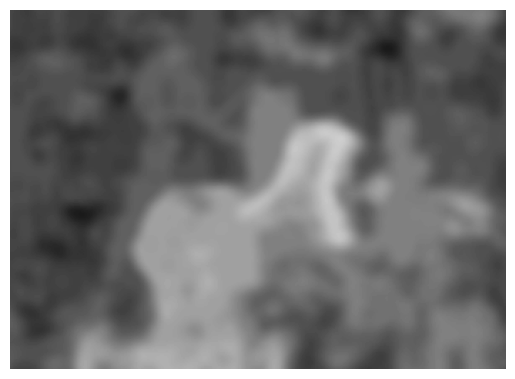} & \includegraphics[width=\rectifiertableimagewidth, height=\rectifiertableimageheight]{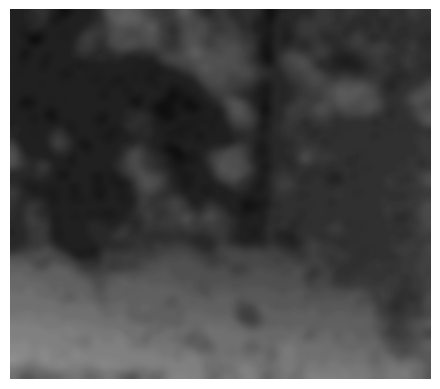}  & \includegraphics[width=\rectifiertableimagewidth, height=\rectifiertableimageheight]{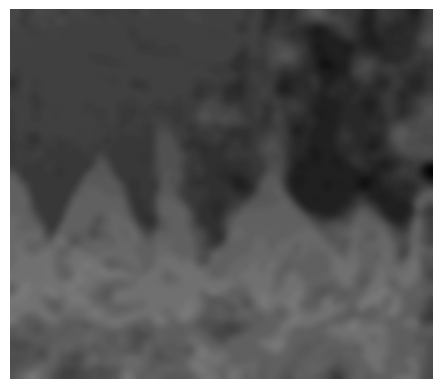} & \includegraphics[width=\rectifiertableimagewidth, height=\rectifiertableimageheight]{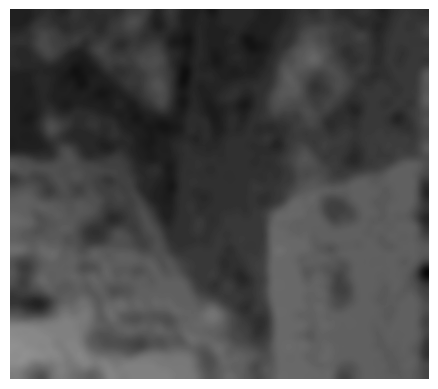}\\
       \rotatebox{90}{\textcolor{white}{----.}$t = 1$ (\textbf{SA})} & \includegraphics[width=\rectifiertableimagewidth, height=\rectifiertableimageheight]{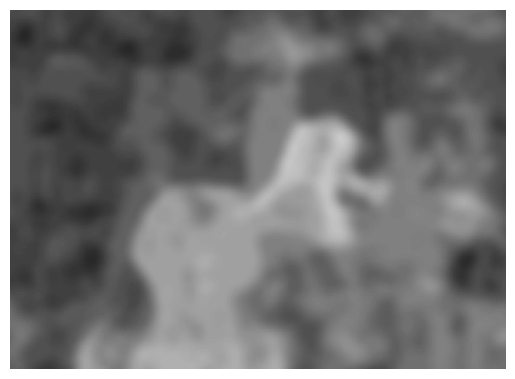} & \includegraphics[width=\rectifiertableimagewidth, height=\rectifiertableimageheight]{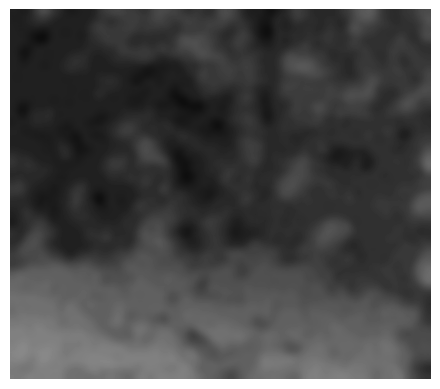}  & \includegraphics[width=\rectifiertableimagewidth, height=\rectifiertableimageheight]{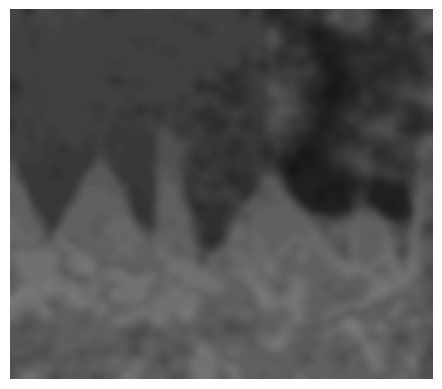} & \includegraphics[width=\rectifiertableimagewidth, height=\rectifiertableimageheight]{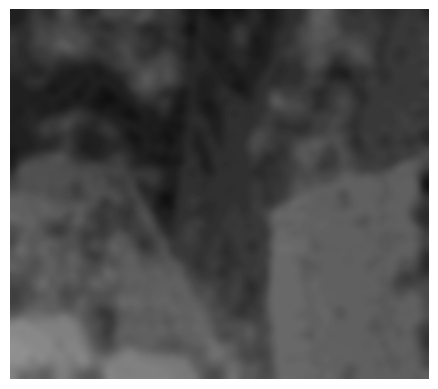}\\
       \rotatebox{90}{\textcolor{white}{--.}$t = 1.25$ (\textbf{SA})} & \includegraphics[width=\rectifiertableimagewidth, height=\rectifiertableimageheight]{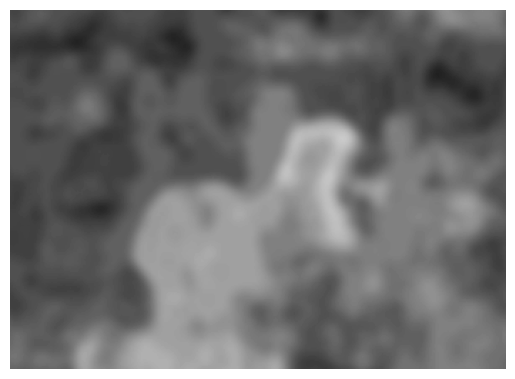} & \includegraphics[width=\rectifiertableimagewidth, height=\rectifiertableimageheight]{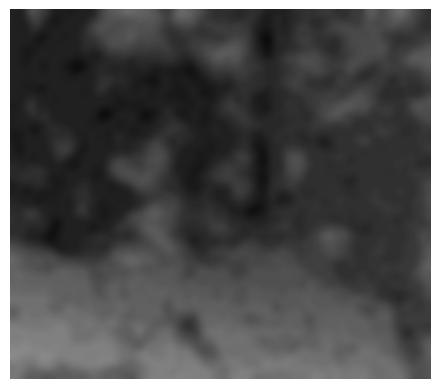}  & \includegraphics[width=\rectifiertableimagewidth, height=\rectifiertableimageheight]{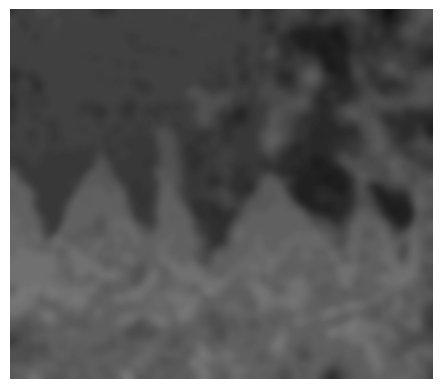} & \includegraphics[width=\rectifiertableimagewidth, height=\rectifiertableimageheight]{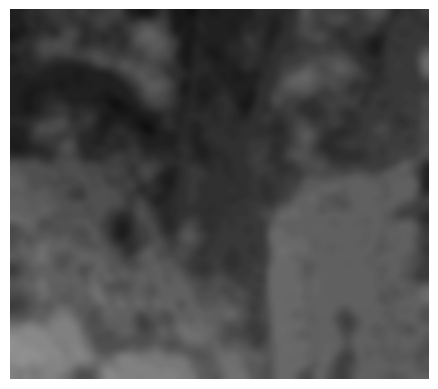}\\
       \rotatebox{90}{\textcolor{white}{---.}$t = 1.5$ (\textbf{SA})} & \includegraphics[width=\rectifiertableimagewidth, height=\rectifiertableimageheight]{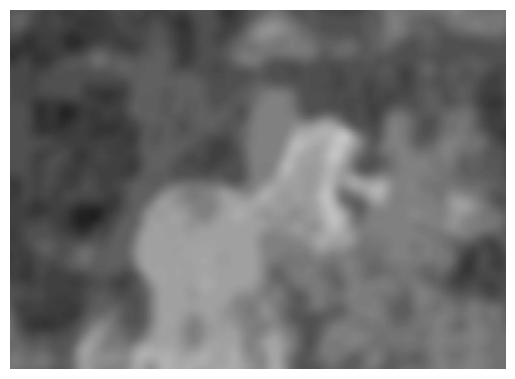} & \includegraphics[width=\rectifiertableimagewidth, height=\rectifiertableimageheight]{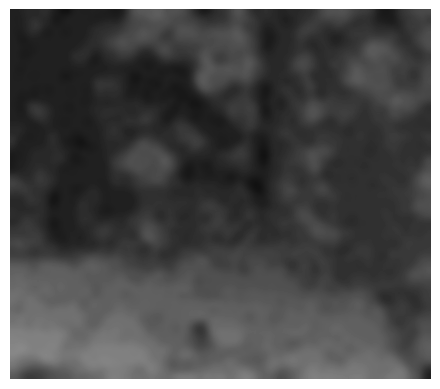}  & \includegraphics[width=\rectifiertableimagewidth, height=\rectifiertableimageheight]{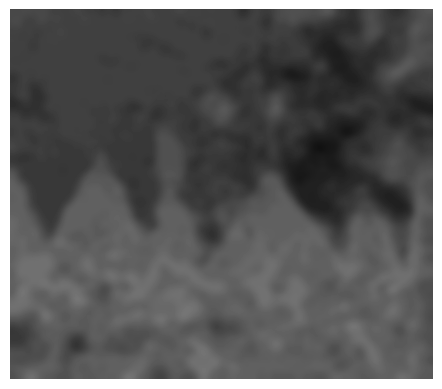} & \includegraphics[width=\rectifiertableimagewidth, height=\rectifiertableimageheight]{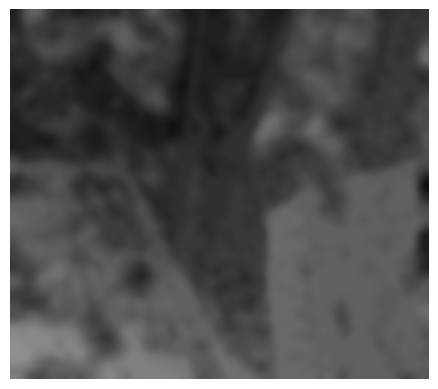}\\
    \end{tabular}
    \caption{\textbf{G}round-\textbf{T}ruth displacements compared with our \textbf{S}imulated \textbf{A}nnealing approach for increasing $t$ values.} 
    \label{fig:ablation_rectifier_strength}
\end{figure}
