# Supplementary material for: Quantum-Hybrid Stereo Matching With Nonlinear Regularization and Spatial Pyramids
Source: arXiv:2312.16118 source file (2024-12-06)
Supplement: Supplementary file 11 [file sintel_experiments.tex]

\section{Sintel Experiments} \label{sec:sintel_experiments}
We ran our model on several stereo image pairs from the  Sintel dataset \cite{Butler:ECCV:2012}. To account for the larger displacements present in the Sintel data, we adjusted our method to now have six coarse-to-fine levels in total. The full configuration of hyperparameters is given in \cref{tab:model_hyperparamters_sintel}. Visual results can be found in \cref{fig:sintel_results}, and numerical results can be found in \cref{tab:sintel_stats}. All estimates were done using Gurobi \cite{Gurobi2023}.

We observe that our method is capable of scaling up to larger image pairs with more complex scenes. In particular, stereo pairs with a continuous gradient of disparities, such as the walls in Alley 2, are estimated well. The method is also capable of picking out finer details, such as the ladder in the lower left section of Alley 2. At the same time, there are still some challenges. Small errors in coarser iterations compound into larger errors (observe the blotchy artifact in the upper right section of Alley 2, for example). The proposed approach also struggles with precision in detail-heavy foregrounds. For example, the hair in Alley 1 is missing some finer details. We suspect that in this case, the brightness constancy assumption is insufficient, and more advanced data terms could be investigated in the future. 

\begin{table}[]
    \centering
    %\begin{adjustbox}{width=\columnwidth,center}
    \begin{tabular}{|c| c | c | c | c | c | c | }
        \hline
        \textbf{Step} & \textbf{1} & \textbf{2}  & \textbf{3} & \textbf{4} & \textbf{5}  & \textbf{6}  \\ \hline\hline
        Downsample Factor (\cref{alg:full_quantum_algorithm}) & 32 & 16 & 8 & 4 & 2 & 1  \\ \hline
        Displacements Considered (\cref{alg:full_quantum_algorithm})  & 6 & 6 & 6 & 4 & 4 & 4 \\ \hline
        $\tau$ (\cref{eq:edge_aware_potts_model})  & 0.15 & 0.15 & 0.15 & 0.15 & 0.15 & 0.3  \\ \hline
        q (\cref{eq:edge_aware_potts_model})  & 10 & 10 & 10 & 10 & 10 & 10 \\ \hline
        m (\cref{eq:truncated_linear_regularizer})  &  0.0015 &  0.0015 & 0.0015 &  0.0015 & 0.0015 & $\infty$ \\ \hline
        s (\cref{eq:truncated_linear_regularizer}) & 0.0005  & 0.0005 & 0.0005 & 0.0005 & 0.0003 & 0.0005\\ \hline
        Median Filter Window (\cref{alg:full_quantum_algorithm}) & 3$\times$3 & 3$\times$3 & 3$\times$3 & 3$\times$3 & 3$\times$3 & 7$\times$7 \\ \hline
        Bilateral Filter Diameter (\cref{alg:full_quantum_algorithm}) & \textbf{n/a} & \textbf{n/a} & \textbf{n/a} & \textbf{n/a} & \textbf{n/a} & 12 \\ \hline
        Bilateral Filter Sigma Color (\cref{alg:full_quantum_algorithm}) & \textbf{n/a} & \textbf{n/a} & \textbf{n/a} & \textbf{n/a} & \textbf{n/a} & 75 \\ \hline 
        Bilateral Filter Sigma Space (\cref{alg:full_quantum_algorithm}) & \textbf{n/a} & \textbf{n/a} & \textbf{n/a} & \textbf{n/a} & \textbf{n/a} & 75 \\ \hline 
        \end{tabular}
    \caption{Hyperparameters for our stereo matching algorithm for the Sintel dataset \cite{Butler:ECCV:2012}.}
    \label{tab:model_hyperparamters_sintel}
\end{table}

\begin{figure}
    \centering
    \setlength\tabcolsep{1.5pt}
    \begin{tabular}{c c c c}
                & Alley 1 & Alley 2 & Sleeping 2 \\
        \rotatebox{90}{\textcolor{white}{--------}\textbf{LI}} & \includegraphics[width=\sinteltableimagewidth, height=\sinteltableimageheight]{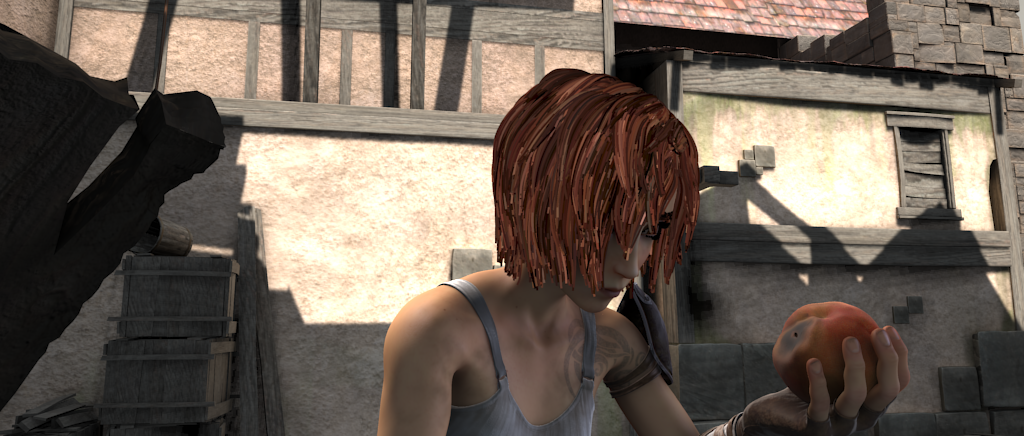} & \includegraphics[width=\sinteltableimagewidth, height=\sinteltableimageheight]{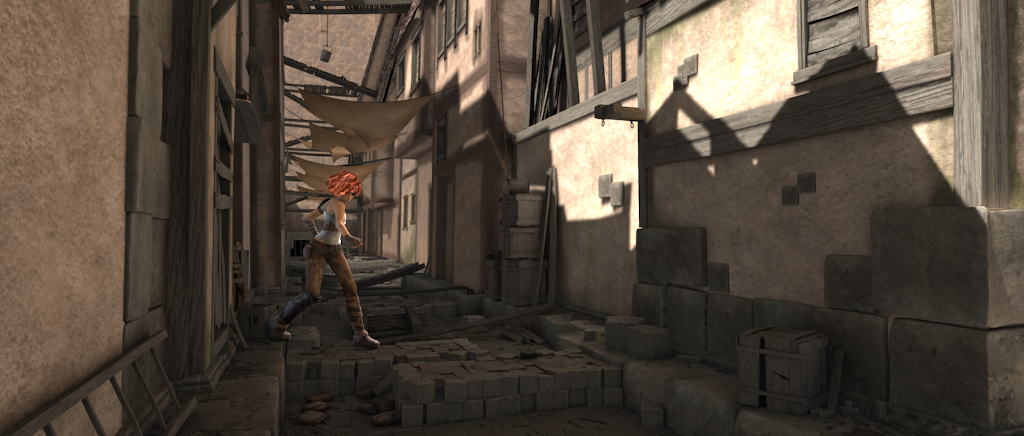}  & \includegraphics[width=\sinteltableimagewidth, height=\sinteltableimageheight]{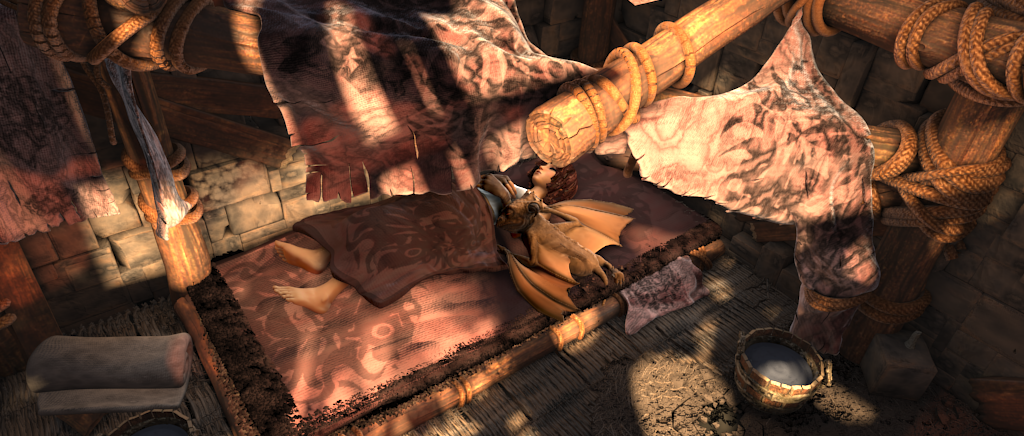} \\
       \rotatebox{90}{\textcolor{white}{---------}\textbf{GT}} & \includegraphics[width=\sinteltableimagewidth, height=\sinteltableimageheight]{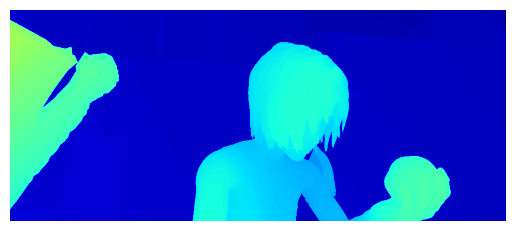} & \includegraphics[width=\sinteltableimagewidth, height=\sinteltableimageheight]{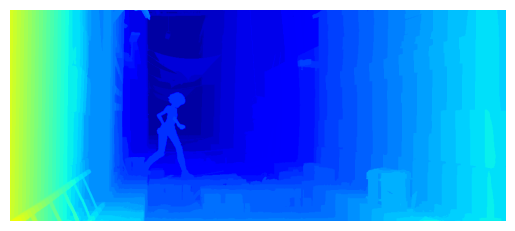}  & \includegraphics[width=\sinteltableimagewidth, height=\sinteltableimageheight]{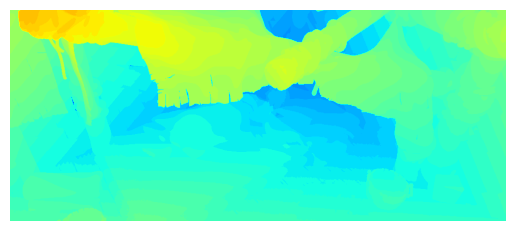} \\
       \rotatebox{90}{\textcolor{white}{------}Ours (\textbf{G})} & \includegraphics[width=\sinteltableimagewidth, height=\sinteltableimageheight]{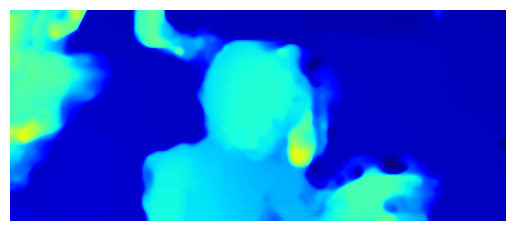} & \includegraphics[width=\sinteltableimagewidth, height=\sinteltableimageheight]{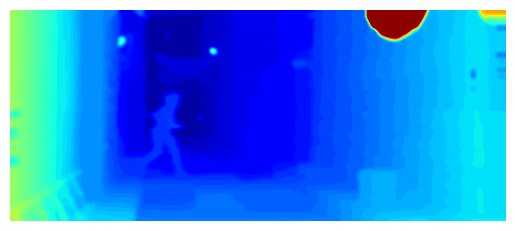}  & \includegraphics[width=\sinteltableimagewidth, height=\sinteltableimageheight]{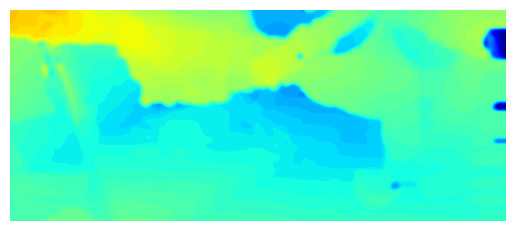} \\
                   & Temple 2 & Market 2 & Sleeping 1 \\
        \rotatebox{90}{\textcolor{white}{--------}\textbf{LI}} & \includegraphics[width=\sinteltableimagewidth, height=\sinteltableimageheight]{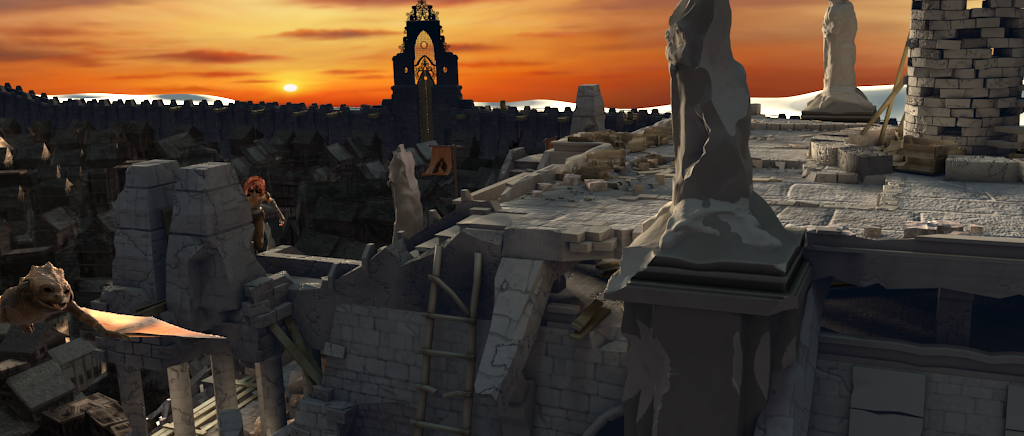} & \includegraphics[width=\sinteltableimagewidth, height=\sinteltableimageheight]{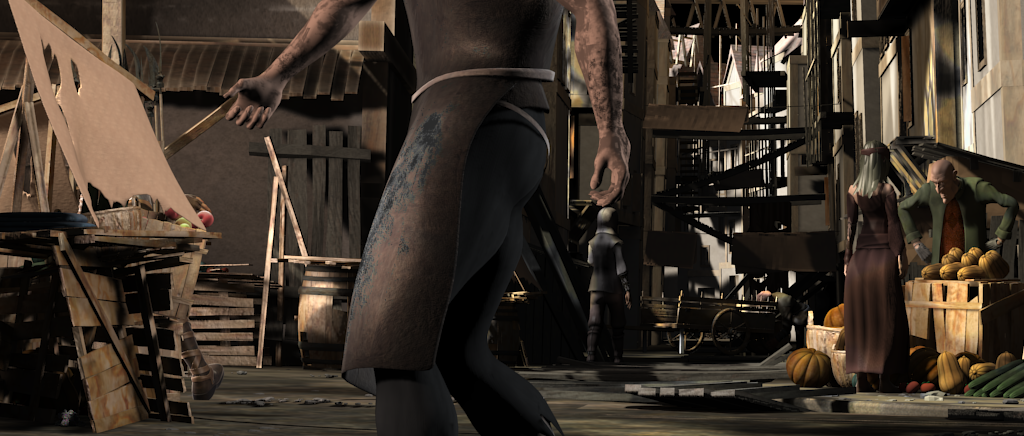}  & \includegraphics[width=\sinteltableimagewidth, height=\sinteltableimageheight]{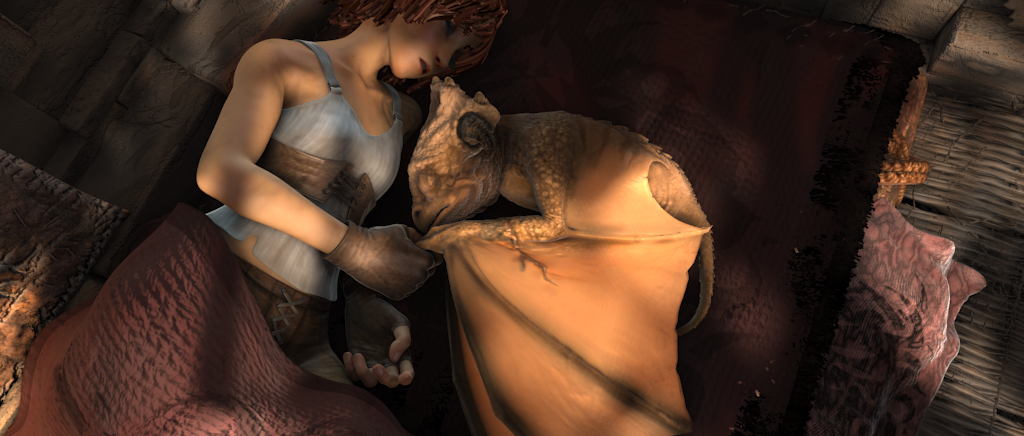} \\
       \rotatebox{90}{\textcolor{white}{---------}\textbf{GT}} & \includegraphics[width=\sinteltableimagewidth, height=\sinteltableimageheight]{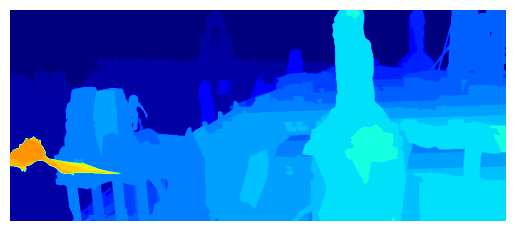} & \includegraphics[width=\sinteltableimagewidth, height=\sinteltableimageheight]{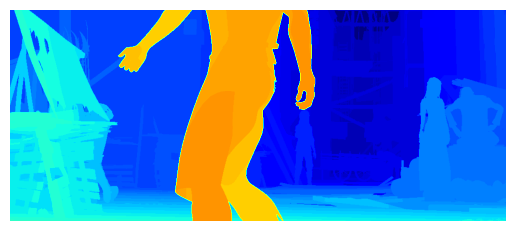}  & \includegraphics[width=\sinteltableimagewidth, height=\sinteltableimageheight]{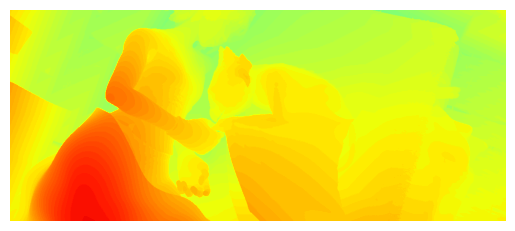} \\
       \rotatebox{90}{\textcolor{white}{------}Ours (\textbf{G})} & \includegraphics[width=\sinteltableimagewidth, height=\sinteltableimageheight]{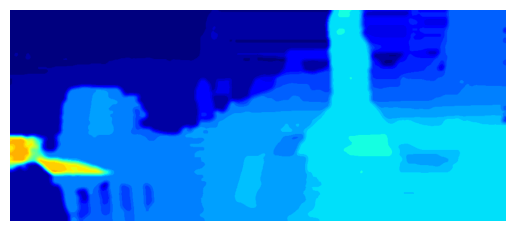} & \includegraphics[width=\sinteltableimagewidth, height=\sinteltableimageheight]{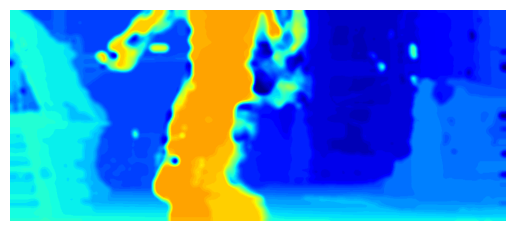}  & \includegraphics[width=\sinteltableimagewidth, height=\sinteltableimageheight]{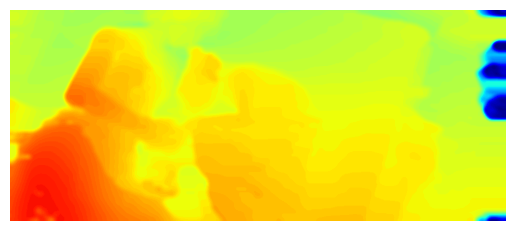} \\
    \end{tabular}
    \caption{The first and fourth rows show the \textbf{L}eft \textbf{I}mage from the first frame of the selected scenes of the Sintel stereo pairs. The second and fifth rows show the \textbf{G}round-\textbf{T}ruth displacements for each pair. The third and sixth rows show our stereo estimation approach using \textbf{G}urobi. We observe that our method can still make robust estimates, even though the input data is of higher resolution and more visually complex.} 
    \label{fig:sintel_results}
\end{figure}

\begin{table}[]
    \centering
    \begin{tabular}{|c| c | c |}
        \hline
        \multirow{2}{*}{\textbf{Image Pair}} &  \multicolumn{2}{ c |}{Ours (\textbf{G})} \\ \cline{2-3} 
            & RMSE & BPP \\
            \hline
        \textbf{Alley 1}    & 38.44 & 50.21  \\ \hline
        \textbf{Alley 2}    & 12.44 & 23.03  \\ \hline
        \textbf{Sleeping 2} &  3.47 & 20.23 \\ \hline
        \textbf{Temple 2}    &  1.88 & 10.30  \\ \hline
        \textbf{Market 2}    & 10.83 & 31.22  \\ \hline
        \textbf{Sleeping 1}  &  8.73 & 60.35  \\ \hline
        \end{tabular}
    
    \caption{The Root Mean Squared Error (RMSE) and Bad Pixel Percentage (BPP) of our method using \textbf{G}urobi on frame pairs from the Sintel dataset.} 
    \label{tab:sintel_stats}
\end{table}
